# Supplementary material for: A2Z GameSpec-Bench: How Faithfully Can Coding Agents Generate Games from Game Design Specifications?
Source: arXiv:2609.39564 source file (2026-09-30)
Supplement: Supplementary file 1 [file appendix_contract_gdd_rows.tex]

\begin{figure*}[t]
  \centering
  \includegraphics[width=1\textwidth]{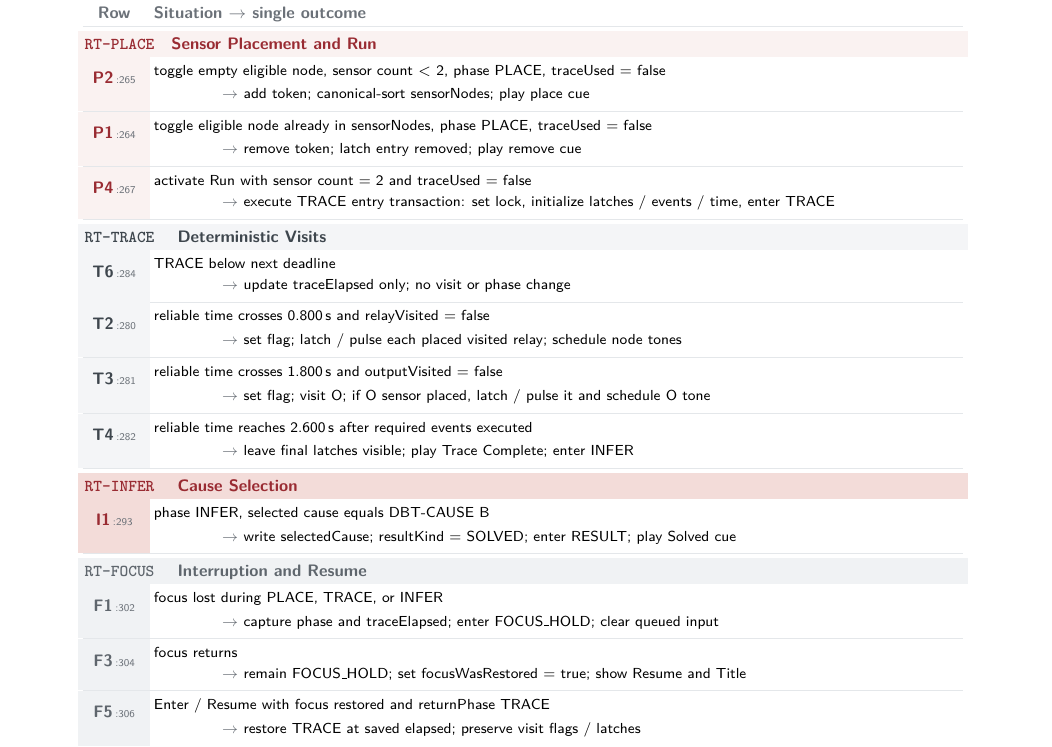}
  \caption{The GDD rows the entries in Figure~\ref{fig:contract-graph} were derived from, in the four
    sections of \texttt{traces\_left} that the run touched, each labelled with its line in the framed
    GDD. A row states a situation and its required effects ($\rightarrow$); the pipeline formalizes the situation as the rule's trigger and preconditions, and the required effects as state updates or event emissions.}
  \label{fig:contract-gdd-rows}
\end{figure*}
