# Supplementary material for: A2Z GameSpec-Bench: How Faithfully Can Coding Agents Generate Games from Game Design Specifications?
Source: arXiv:2609.39564 source file (2026-09-30)
Supplement: Supplementary file 2 [file appendix_contract_graph.tex]

\begin{figure*}[t]
  \centering
  \includegraphics[width=0.8\textwidth]{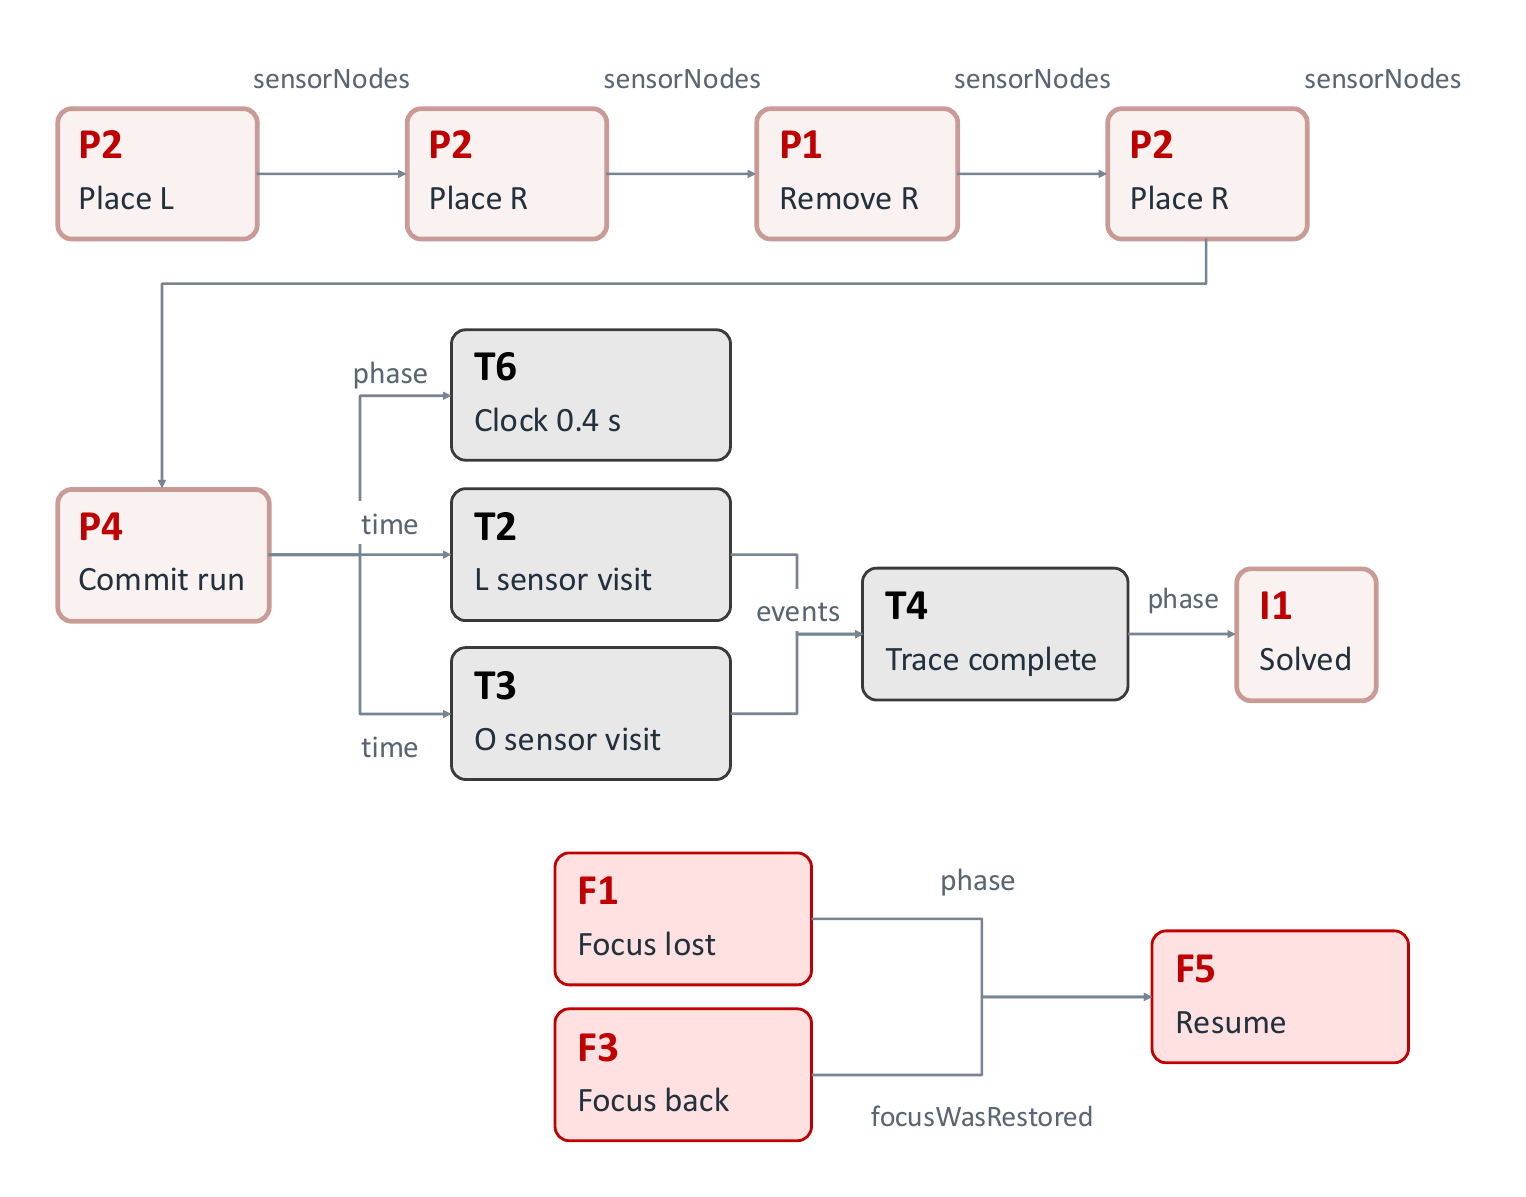}
  \caption{\textbf{Contract-linked execution of \texttt{traces\_left}.} Nodes show rule occurrences in a recorded normal playtest, and labeled links indicate the state attributes connecting them. Three sensor placements and one removal precede \texttt{P4}, which commits the run. The fixed contract supplies the rule identities and dependencies; the trace supplies their observed order. Source GDD rows appear in Figure~\ref{fig:contract-gdd-rows}.}
  \label{fig:contract-graph}
\end{figure*}
