# Supplementary material for: A2Z GameSpec-Bench: How Faithfully Can Coding Agents Generate Games from Game Design Specifications?
Source: arXiv:2609.39564 source file (2026-09-30)
Supplement: Supplementary file 3 [file brief_cv_gdd.tex]

\begin{figure*}[t]
\centering
\includegraphics[width=\textwidth]{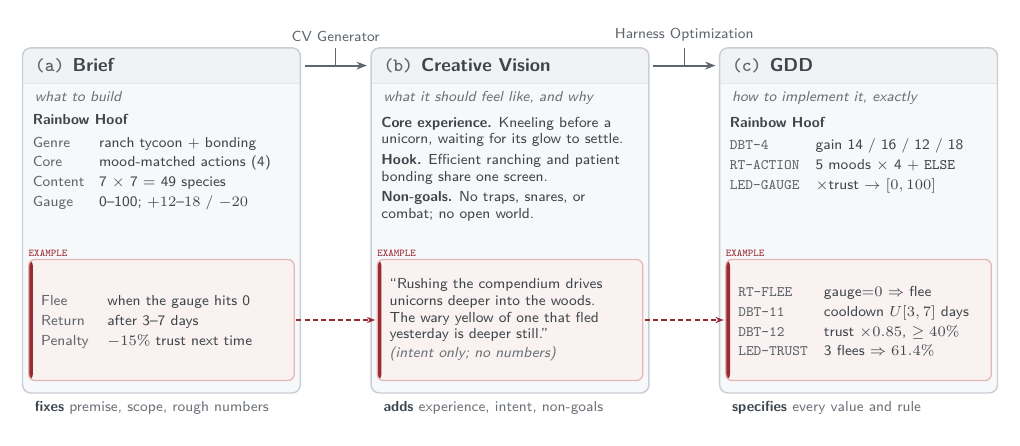}
\caption{One game traced from brief to GDD. The brief fixes what to build, the
CV adds how the game should feel and why (without numbers), and the GDD
specifies every value and rule. The highlighted boxes follow one requirement, the
cost of letting a unicorn flee, through all three stages: a rough rule in the
brief, a design intent in the CV, and a cited rule, constants, and a worked
example in the GDD.}
\label{fig:brief_cv_gdd}
\end{figure*}
