# Supplementary material for: A2Z GameSpec-Bench: How Faithfully Can Coding Agents Generate Games from Game Design Specifications?
Source: arXiv:2609.39564 source file (2026-09-30)
Supplement: Supplementary file 4 [file card_helpers.tex]

% Card-style case panels. Required: graphicx, tikz (calc). Frames 1920x1080; crop units bp = px.
\usetikzlibrary{calc}
% Image folders (edit to match the manuscript). Files expected inside:
%   \CardRainDir   : rain_affordable_held.png, rain_unaffordable_held.png
%   \CardStrataDir : strata_keepers_before.png, strata_keepers_after.png
%   \CardChromaDir : chroma_bastion_after.png
\providecommand{\CardRainDir}{assets/appendix/rain_affordable}
\providecommand{\CardStrataDir}{assets/appendix/strata_keepers}
\providecommand{\CardChromaDir}{assets/appendix/chroma}
\definecolor{CInk}{HTML}{263544}\definecolor{CMuted}{HTML}{64717C}\definecolor{CRed}{HTML}{B32F2A}
\definecolor{CLine}{HTML}{C5CDD4}\definecolor{CFill}{HTML}{ECF0F3}\definecolor{CRedFill}{HTML}{F8E3E0}\definecolor{CDot}{HTML}{C3CAD0}
% card frame: #1 game name, #2 source label, #3 playtest label
\newcommand{\CardFrame}[4]{%
  \draw[CLine,line width=.6pt,fill=white,rounded corners=6pt] (0,0) rectangle (17.80,7.67);
  \fill[CFill] (0.02,6.90) rectangle (17.78,7.65); \draw[CLine,line width=.4pt] (0,6.90)--(17.80,6.90);
  \definecolor{CDotR}{HTML}{FF5F57}\definecolor{CDotY}{HTML}{FEBC2E}\definecolor{CDotG}{HTML}{28C840}
  \fill[CDotR] (.42,7.28) circle (.075); \fill[CDotY] (.70,7.28) circle (.075); \fill[CDotG] (.98,7.28) circle (.075);
  \node[anchor=west,font=\ttfamily\fontsize{13}{14}\selectfont\bfseries,text=CInk] at (1.35,7.28) {#4#1};
  \node[draw=CLine,fill=white,rounded corners=3pt,inner xsep=9pt,inner ysep=3.5pt,font=\sffamily\fontsize{9.5}{11}\selectfont,text=CInk,anchor=center] at (9.3,7.28) {Source Code: \textbf{#2}};
  \node[draw=CRed!45,fill=CRedFill,rounded corners=3pt,inner xsep=9pt,inner ysep=3.5pt,font=\sffamily\fontsize{9.5}{11}\selectfont,text=CInk,anchor=center] at (14.9,7.28) {Playtest: \textcolor{CRed}{\textbf{#3}}};
}
% main screenshot: #1 file (9.3cm wide → 5.23cm tall), origin (.30,.35)
\newcommand{\CardMain}[1]{%
  \node[anchor=south west,inner sep=0pt] at (.30,.35) {\includegraphics[width=9.30cm]{#1}};
  \draw[CLine,line width=.4pt] (.30,.35) rectangle (9.60,5.58);
}
% cause bar over the screenshot: #1 text
% cause strip below the screenshot (full card width): #1 text
\newcommand{\CardCause}[1]{%
  \draw[CLine,line width=.4pt,fill=CFill,rounded corners=3pt] (.30,.30) rectangle (17.50,.82);
  \node[anchor=west,font=\sffamily\fontsize{9}{10}\selectfont,text=CInk] at (.48,.56) {\textcolor{CRed}{\bfseries Cause:}\; \texttt{#1}};
}
% callout label: #1 x, #2 y (in main-frame fractions), #3 text; #4 = 1 draws a cursor at the anchor
\newcommand{\CardCallout}[4]{%
  \begin{scope}[shift={(.30,.35)},x=9.30cm,y=5.23125cm]
    \node[anchor=south west,fill=white,fill opacity=.96,text opacity=1,rounded corners=2pt,draw=CRed,line width=.5pt,inner xsep=5pt,inner ysep=3pt,font=\sffamily\fontsize{9}{10}\selectfont\bfseries,text=CRed] (co) at (#1,#2) {#3};
    \ifnum#4=1
      \begin{scope}[shift={($(co.south west)+(.10cm,-.02cm)$)},x=1cm,y=1cm]
        \fill[white,draw=CInk,line width=.5pt] (0,0)--(0,-.42)--(.11,-.32)--(.19,-.50)--(.26,-.47)--(.18,-.29)--(.31,-.29)--cycle;
      \end{scope}
    \fi
  \end{scope}
}
% right column boxes (x 9.90–17.50)
\newcommand{\CardReq}[1]{%
  \draw[CLine,line width=.4pt,fill=CFill,rounded corners=3pt] (9.90,4.30) rectangle (17.50,5.58);
  \node[anchor=north west,font=\sffamily\fontsize{10}{11}\selectfont\bfseries,text=CInk] at (10.08,5.43) {\raisebox{-1pt}{\tikz\draw[CMuted,line width=.5pt] (0,0) rectangle (.22,.28) (.05,.09)--(.17,.09) (.05,.15)--(.17,.15) (.05,.21)--(.17,.21);}\; GDD Requirement};
  \node[anchor=north west,text width=7.2cm,align=left,font=\rmfamily\fontsize{10}{12}\selectfont,text=CInk] at (10.08,5.03) {#1};
}
% #1 title, #2 file, #3-#6 trim l b r t, #7 unused (kept for compatibility); crops are set by height
\newcommand{\CardBefore}[7]{%
  \draw[CLine,line width=.4pt,fill=CFill,rounded corners=3pt] (9.90,2.56) rectangle (17.50,4.16);
  \node[anchor=north west,font=\sffamily\fontsize{10}{11}\selectfont\bfseries,text=CInk] at (10.08,4.01) {#1};
  \node[anchor=north west,inner sep=0pt] at (10.08,3.60) {\includegraphics[trim=#3bp #4bp #5bp #6bp,clip,height=0.92cm]{#2}};
}
% #1 title, #2 file, #3-#6 trim, #7 unused, #8 verdict line
\newcommand{\CardAfter}[8]{%
  \draw[CRed!55,line width=.5pt,fill=CRedFill,rounded corners=3pt] (9.90,.35) rectangle (17.50,2.44);
  \node[anchor=north west,font=\sffamily\fontsize{10}{11}\selectfont\bfseries,text=CRed] at (10.08,2.29) {#1};
  \node[anchor=north west,inner sep=0pt] at (10.08,1.88) {\includegraphics[trim=#3bp #4bp #5bp #6bp,clip,height=0.92cm]{#2}};
  \node[anchor=south west,font=\sffamily\fontsize{9.5}{11}\selectfont\bfseries,text=CRed] at (10.08,.50) {$\times$\; #8};
}
\newcommand{\CardChameleon}[1]{%
\begin{tikzpicture}[x=1cm,y=1cm,every node/.style={inner sep=0pt},font=\sffamily]
  \path[use as bounding box] (0,0) rectangle (17.80,7.67);
  \CardFrame{\texttt{Chameleon Slide}}{Pass}{Violated}{#1}
  \begin{scope}[yshift=.62cm]
  \CardMain{\CardRainDir/../intro_chameleon/cham_after_key1.png}
  \begin{scope}[shift={(.30,.35)},x=9.30cm,y=5.23125cm]
    \draw[CRed!65,line width=.85pt] (.405,.575) rectangle (.465,.655);
  \end{scope}
  \CardCallout{.475}{.66}{Press 1 (Red) at rest}{0}
  \CardReq{At rest, key 1--4 \underline{recolors the body instantly}; no move is spent.}
  \CardBefore{Before key 1: green, moves 0}{\CardRainDir/../intro_chameleon/cham_before.png}{700}{628}{720}{372}{6.3}
  \CardAfter{After key 1: still green, moves 0}{\CardRainDir/../intro_chameleon/cham_after_key1.png}{700}{628}{720}{372}{5.9}{Body never recolors}
  \end{scope}
  \CardCause{handler bound to keydown-1; engine emits keydown-ONE}
\end{tikzpicture}}
\newcommand{\CardStrata}[1]{%
\begin{tikzpicture}[x=1cm,y=1cm,every node/.style={inner sep=0pt},font=\sffamily]
  \path[use as bounding box] (0,0) rectangle (17.80,7.67);
  \CardFrame{\texttt{Strata Keepers}}{Pass}{Violated}{#1}
  \begin{scope}[yshift=.62cm]
  \CardMain{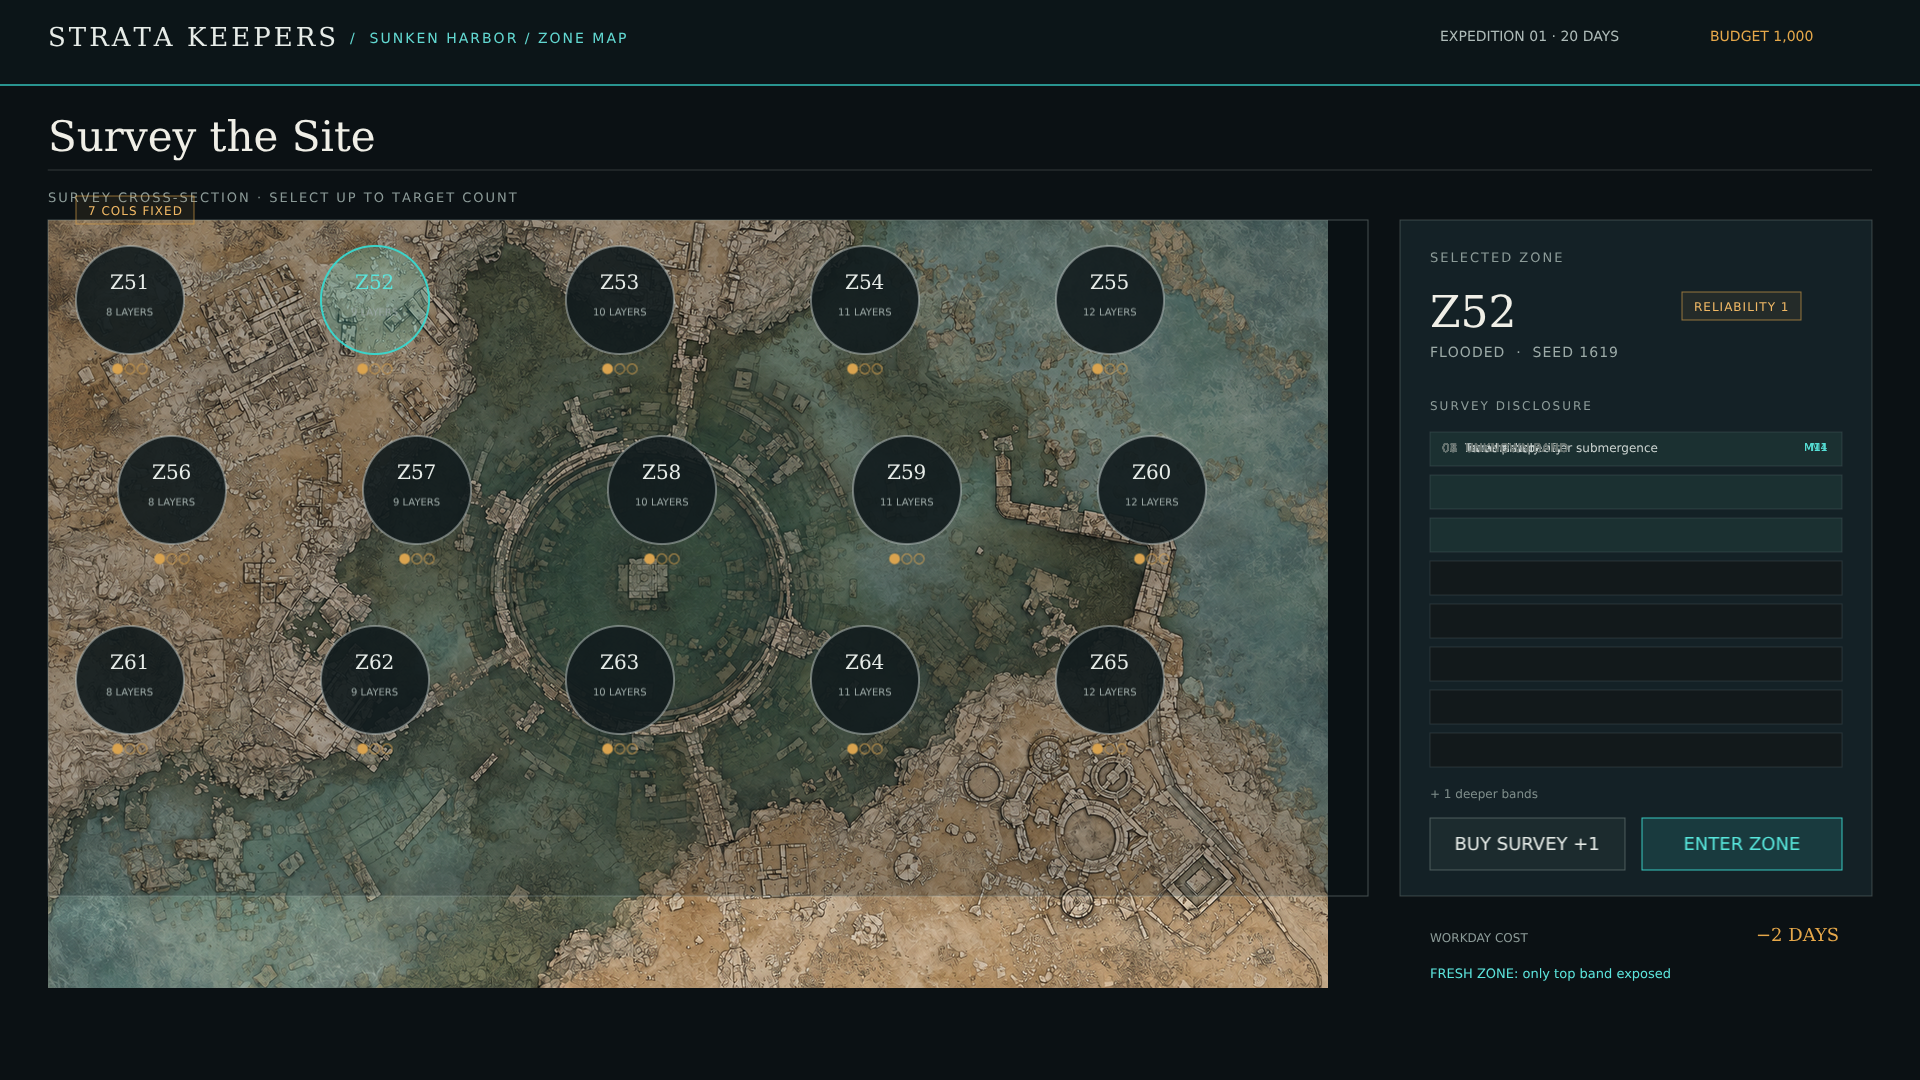}
  \begin{scope}[shift={(.30,.35)},x=9.30cm,y=5.23125cm]
    \draw[CRed!65,line width=.85pt] (.742,.941) rectangle (.848,.989);
    \draw[CRed!65,line width=.85pt] (.851,.185) rectangle (.964,.246);
    \draw[CRed!65,line width=.85pt] (.906,.117) rectangle (.970,.151);
  \end{scope}
  \CardCallout{.56}{.30}{Click ENTER ZONE}{1}
  \CardReq{Entering a zone costs \underline{two workdays}; the map shows ``\,$-$2 DAYS''.}
  \CardBefore{Before entry: 20 days remaining}{\CardStrataDir/strata_keepers_before.png}{1370}{1005}{260}{0}{4.1}
  \CardAfter{After one entry: Day 4 / 20}{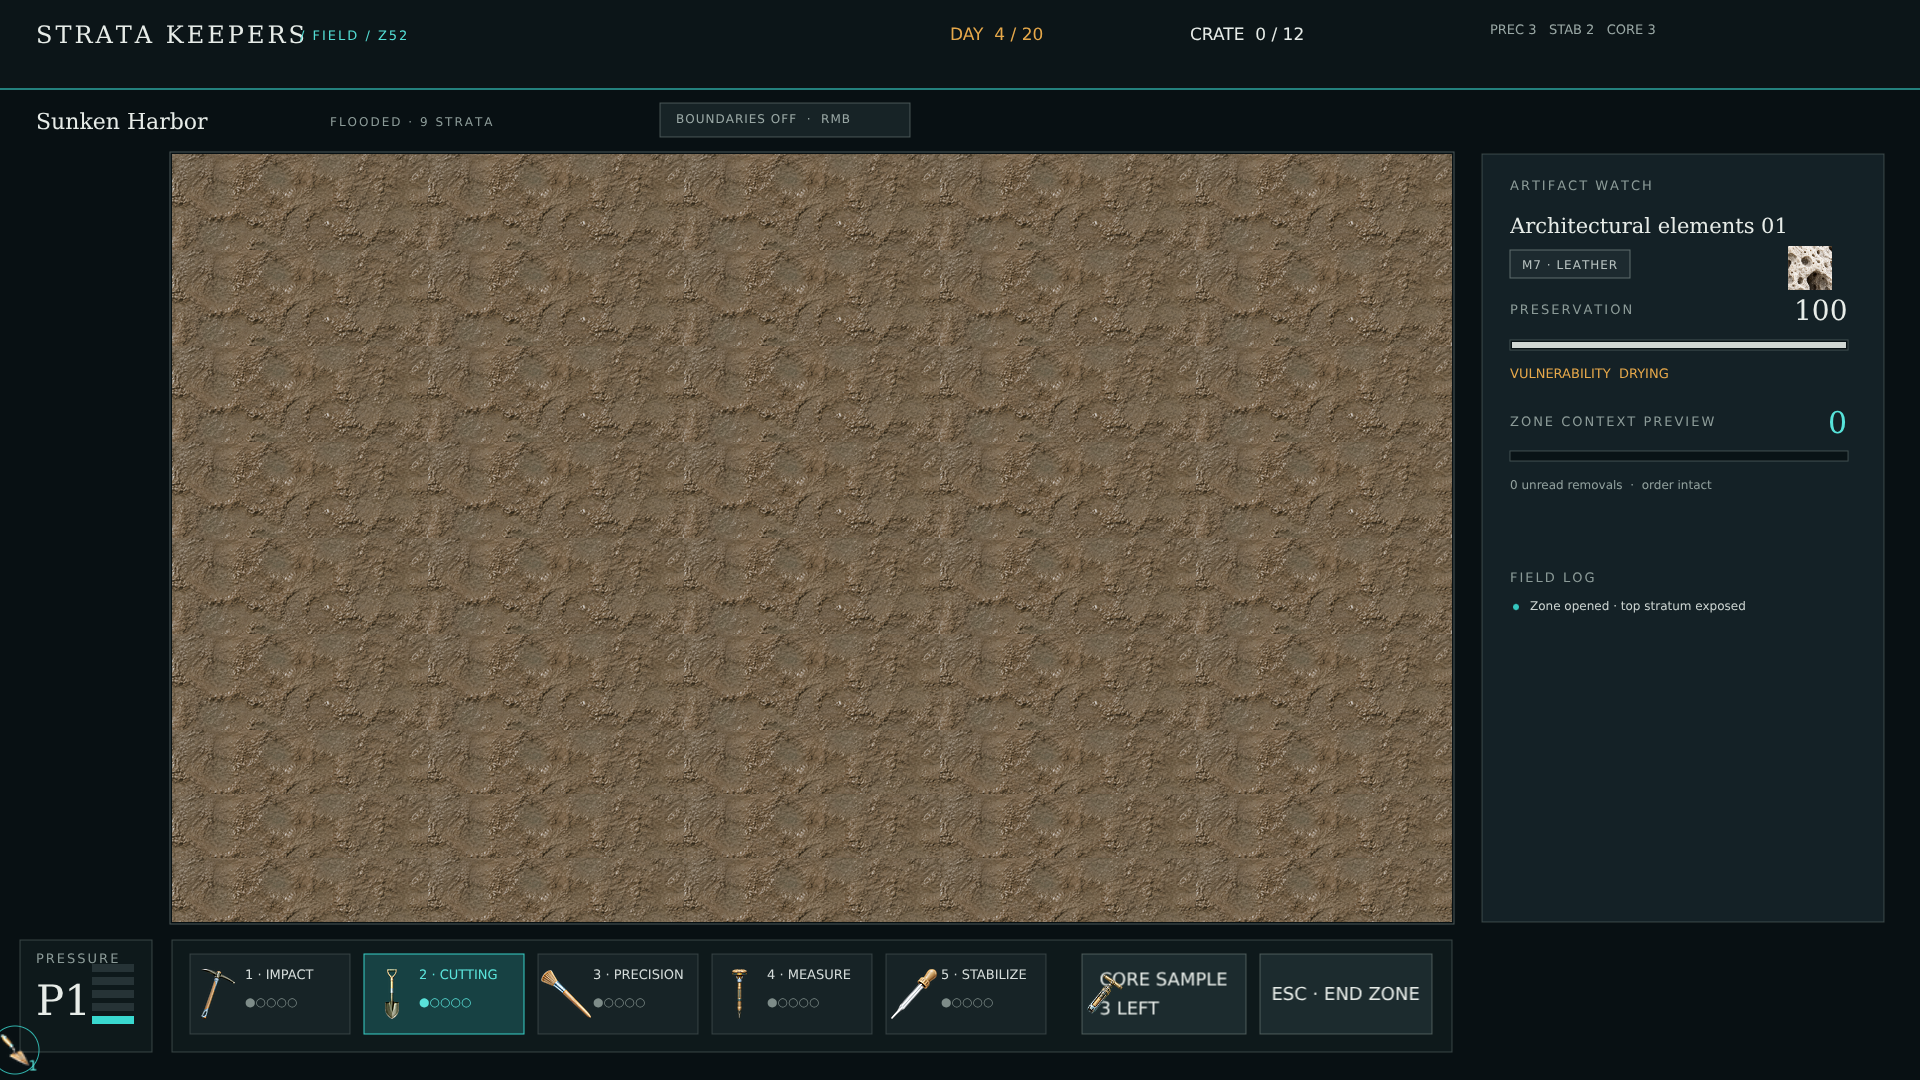}{905}{1008}{810}{0}{2.7}{Four days spent, not two}
  \end{scope}
  \CardCause{workday cost applied twice (state 18, then map -2)}
\end{tikzpicture}}
\newcommand{\CardChroma}[1]{%
\begin{tikzpicture}[x=1cm,y=1cm,every node/.style={inner sep=0pt},font=\sffamily]
  \path[use as bounding box] (0,0) rectangle (17.80,7.67);
  \CardFrame{\texttt{Chroma Bastion}}{Pass}{Violated}{#1}
  \begin{scope}[yshift=.62cm]
  \CardMain{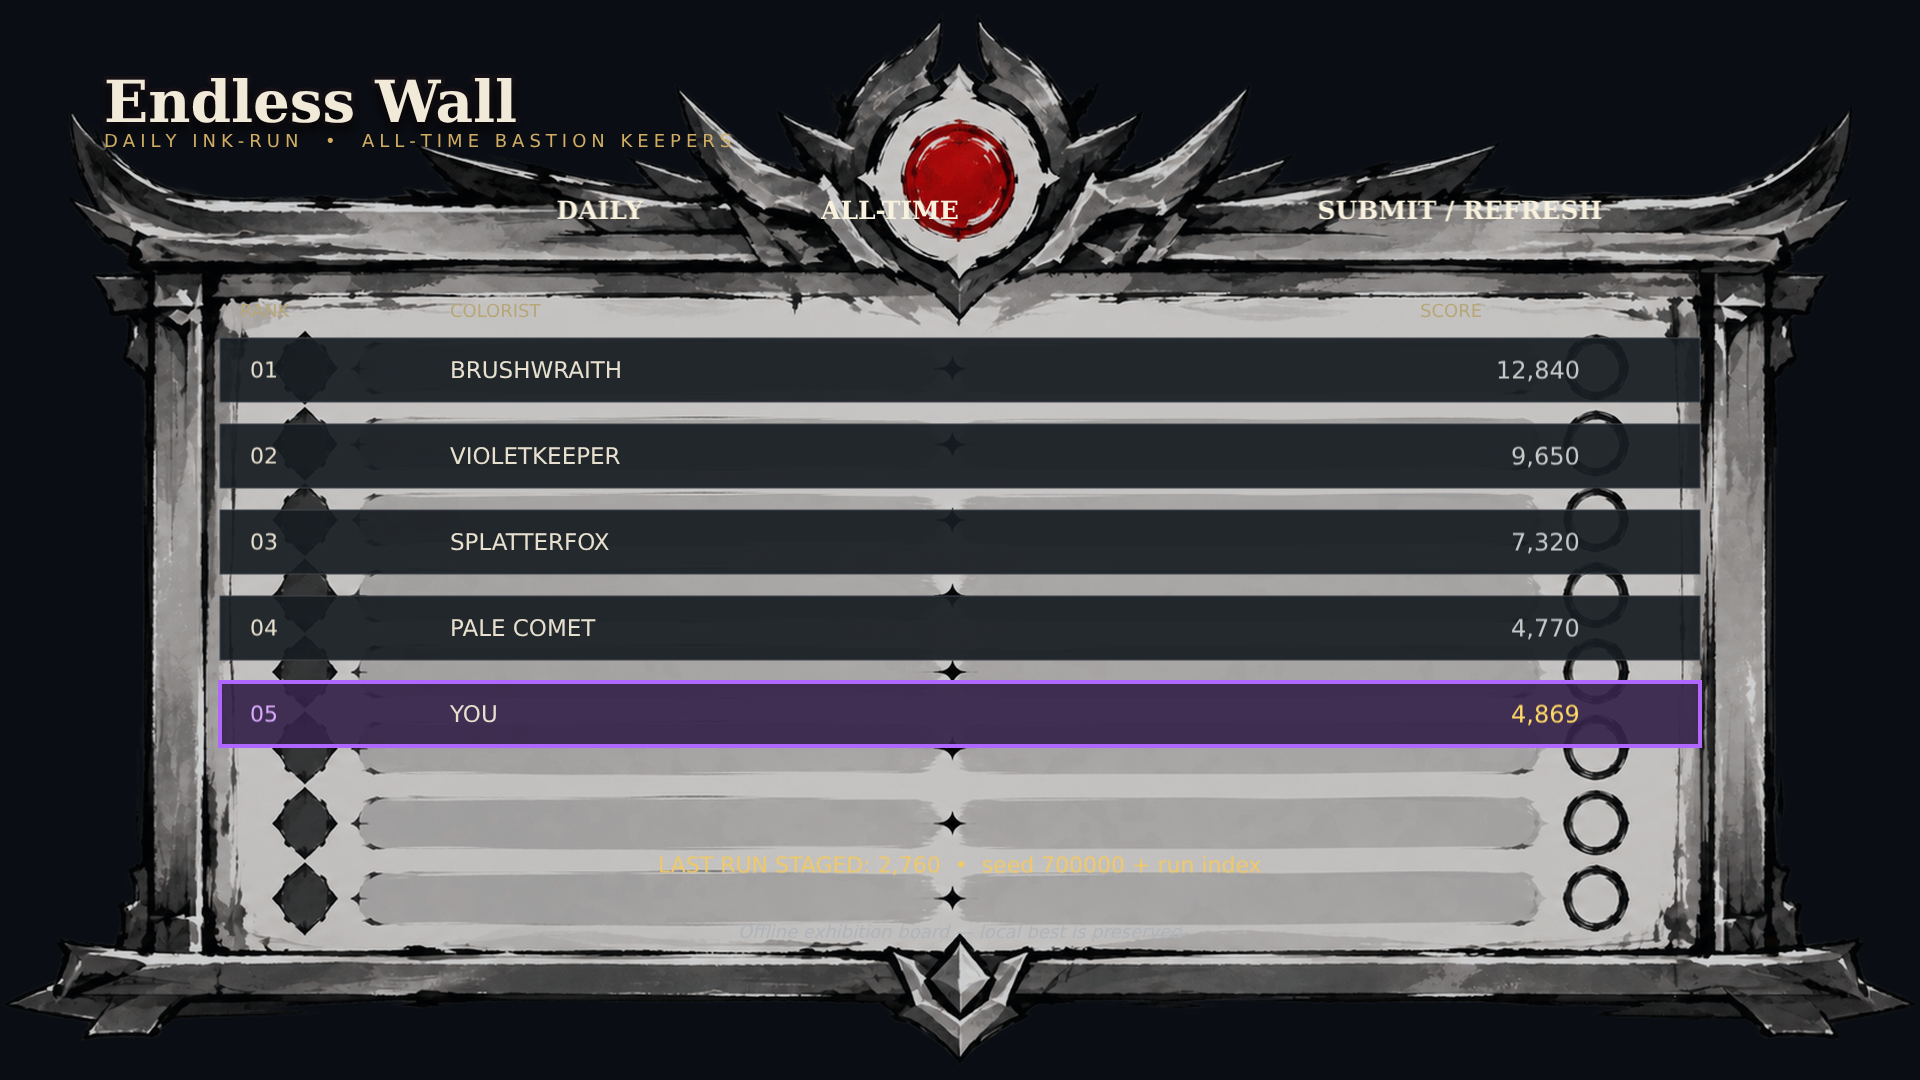}
  \begin{scope}[shift={(.30,.35)},x=9.30cm,y=5.23125cm]
    \draw[CRed!65,line width=.85pt] (.765,.322) rectangle (.838,.357);
    \draw[CRed!65,line width=.85pt] (.335,.181) rectangle (.496,.218);
  \end{scope}
  \CardCallout{.34}{.37}{Run ends at erosion 100\%}{0}
  \CardReq{When erosion reaches 100\%, the run ends and \underline{its score is staged} for submission.}
  \CardBefore{Completed run: 4,869 points}{\CardChromaDir/chroma_bastion_after.png}{1420}{305}{270}{655}{2.4}
  \CardAfter{Staged for submission: 2,760}{\CardChromaDir/chroma_bastion_after.png}{630}{175}{965}{815}{3.7}{Wrong score staged}
  \end{scope}
  \CardCause{stagedScore hard-coded to 2760, never updated}
\end{tikzpicture}}

\newcommand{\CardRain}[1]{%
\begin{tikzpicture}[x=1cm,y=1cm,every node/.style={inner sep=0pt},font=\sffamily]
  \path[use as bounding box] (0,0) rectangle (17.80,7.67);
  \CardFrame{\texttt{Rainwright}}{Pass}{Violated}{#1}
  \begin{scope}[yshift=.62cm]
  \CardMain{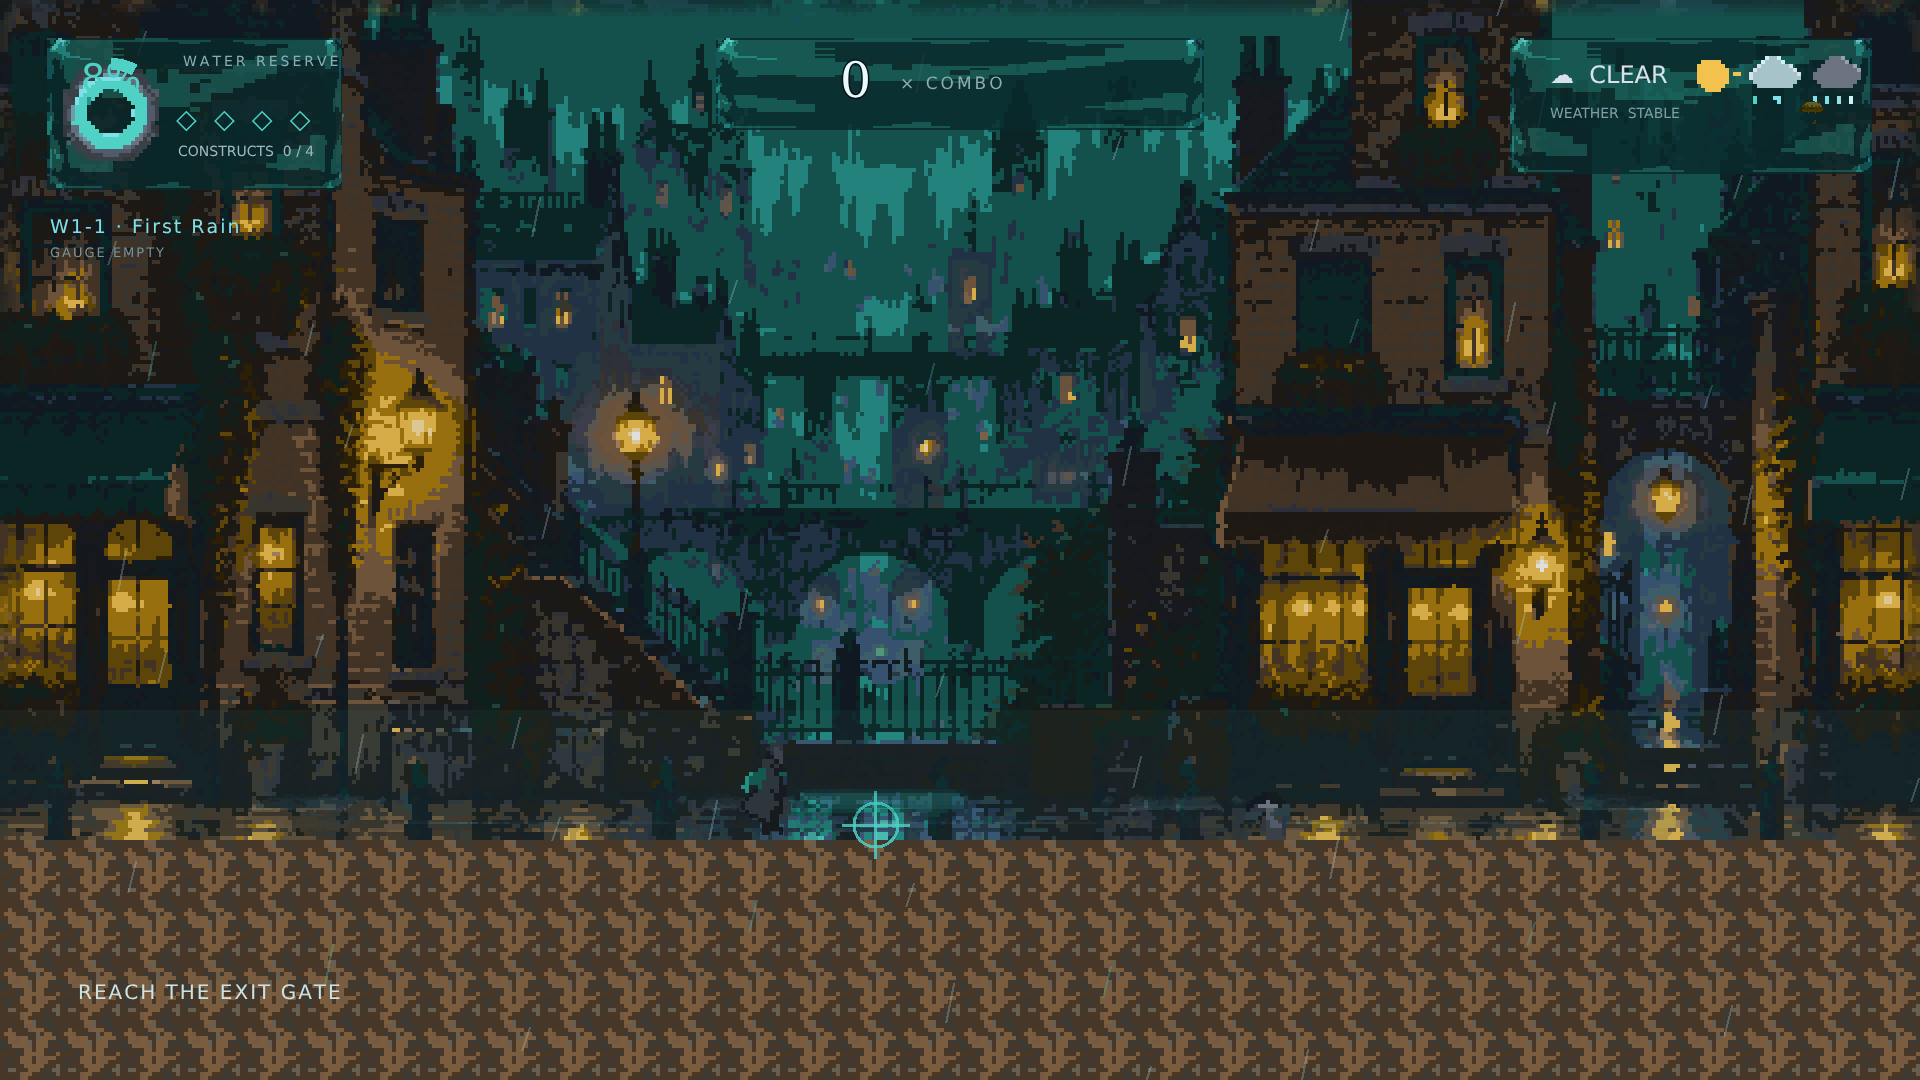}
  \begin{scope}[shift={(.30,.35)},x=9.30cm,y=5.23125cm]
    \draw[CRed!65,line width=.85pt] (.022,.819) rectangle (.182,.970);
    \draw[CRed!65,line width=.85pt] (.380,.185) rectangle (.527,.307);
  \end{scope}
  \CardCallout{.545}{.33}{Hold build (right mouse)}{1}
  \CardReq{While the build input is held, the ghost preview is \underline{tinted red if the build would fail}.}
  \CardBefore{Water 50\% (affordable): teal preview}{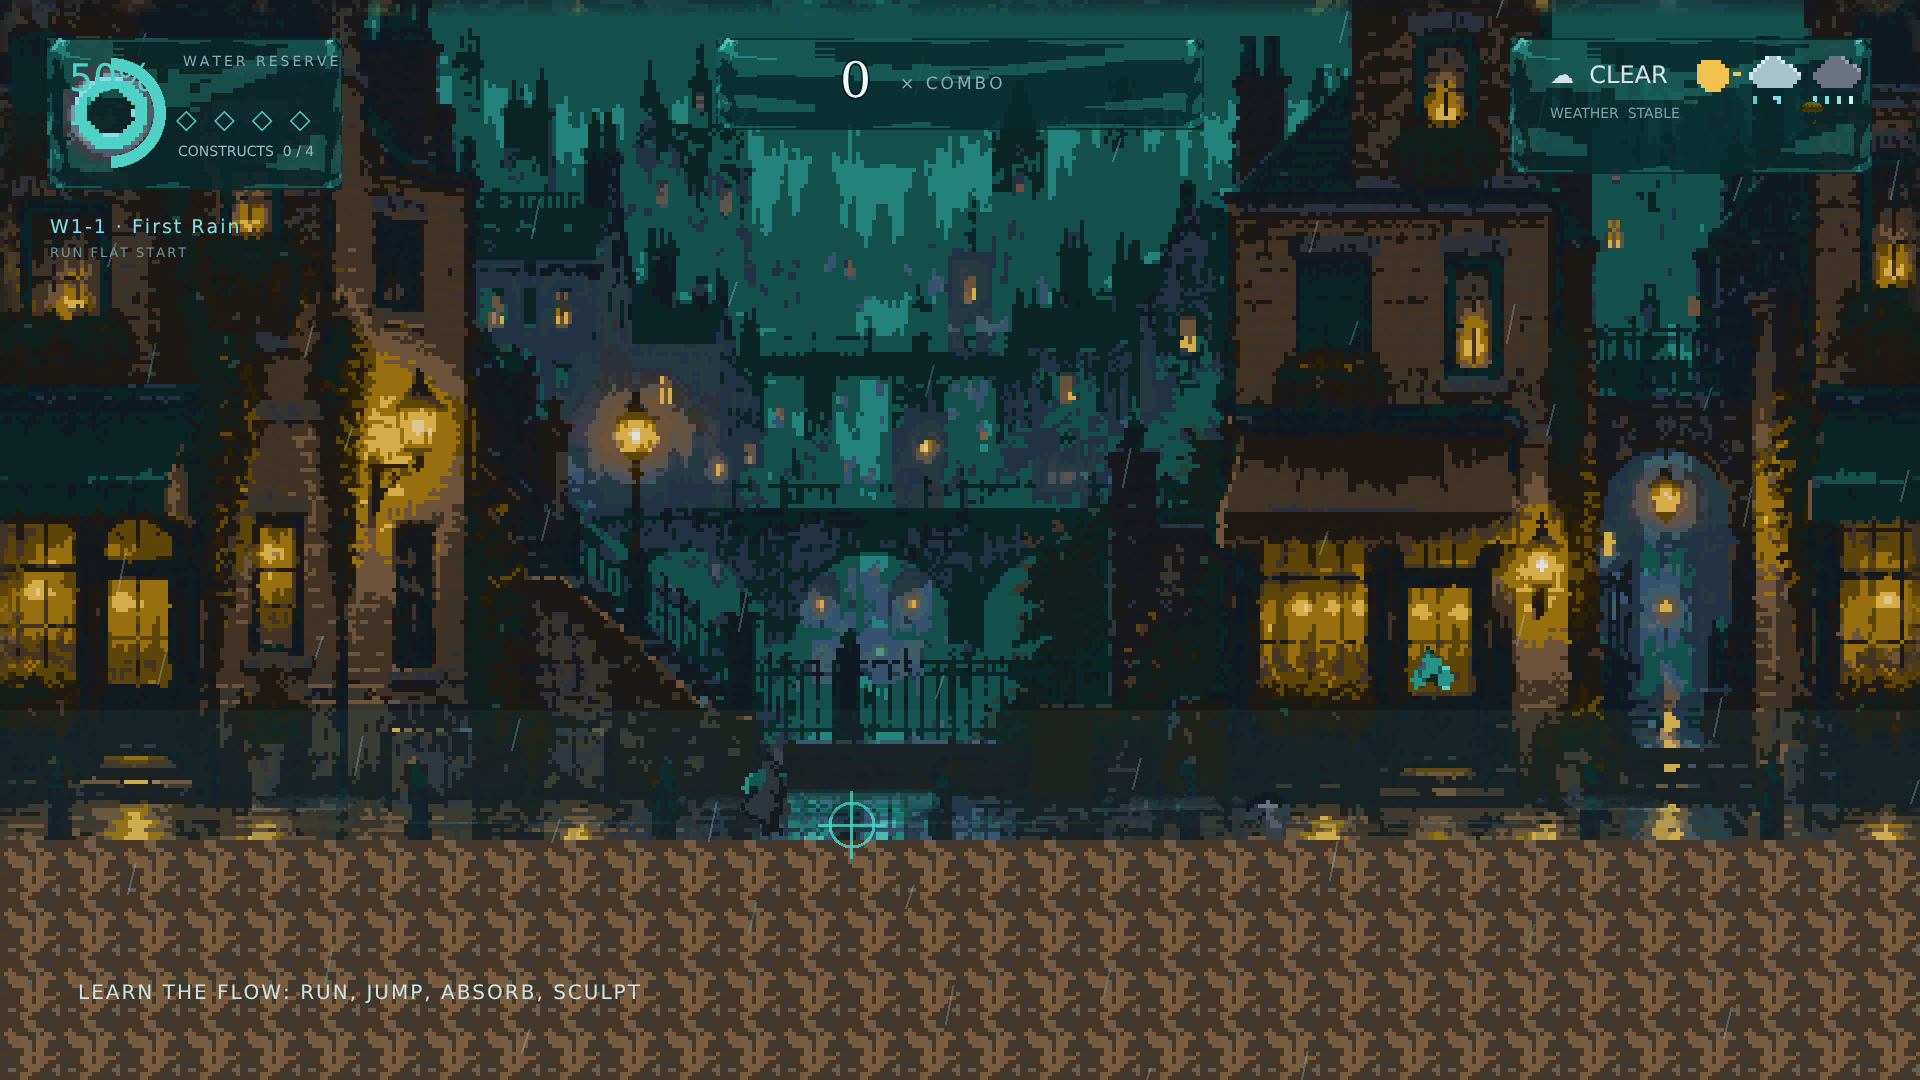}{730}{200}{910}{750}{2.6}
  \CardAfter{Water 8\%, minimum cost 25\%: still teal}{\CardRainDir/rain_unaffordable_held.png}{730}{200}{910}{750}{2.05}{No red warning while held}
  \end{scope}
  \CardCause{buildDenied set only in tryBuild(), on release}
\end{tikzpicture}}
