# Supplementary material for: A2Z GameSpec-Bench: How Faithfully Can Coding Agents Generate Games from Game Design Specifications?
Source: arXiv:2609.39564 source file (2026-09-30)
Supplement: Supplementary file 5 [file cards_all.tex]

% Lives in figures/appendix/. Use from the manuscript root: \input{figures/appendix/cards_all.tex}. Requires graphicx, tikz.
\begin{figure*}[t]
\centering
\begingroup
\input{figures/appendix/card_helpers.tex}
\resizebox{\textwidth}{!}{\CardRain{(a)\;}}\par\vspace{4pt}
\resizebox{\textwidth}{!}{\CardStrata{(b)\;}}\par\vspace{4pt}
\resizebox{\textwidth}{!}{\CardChroma{(c)\;}}
\endgroup
\vspace{-4pt}
\caption{\textbf{Full source-code credit with a runtime violation.} Each rule passes the source-code judge (item score 1.00) and is judged \emph{violated} in the playtest. (a)~\texttt{Rainwright}: with 8\% water, below the 25\% minimum cost, the held build preview stays teal instead of turning red, because the denial flag is set only on release. (b)~\texttt{Strata Keepers}: a two-day zone entry consumes four days because the cost is applied twice. (c)~\texttt{Chroma Bastion}: the finished run scores 4,869 but a constant 2,760 is staged for submission. Screenshots are from asset-integrated builds whose relevant logic is unchanged from the evaluated source; boxes, callouts, and crops are annotations.}
\label{fig:source_runtime_gap}
\end{figure*}
