# Supplementary material for: A2Z GameSpec-Bench: How Faithfully Can Coding Agents Generate Games from Game Design Specifications?
Source: arXiv:2609.39564 source file (2026-09-30)
Supplement: Supplementary file 6 [file qualitative.tex]

% Required preamble packages: graphicx, subcaption.
% Input from the manuscript root: \input{afs_three_columns_english}
% FOUR panels; TWO method rows per panel; THREE image columns in EVERY row.
% Each AFSRow takes exactly one method label and three frame cards.
% Original PNGs are unchanged; edit all crops, timestamps, and labels below.

\begin{figure}[p]
    \centering
    \captionsetup{font=small,skip=6pt}
    \renewcommand{\thesubfigure}{(\alph{subfigure})}
    \captionsetup[subfigure]{font={small,rm,bf},labelfont=bf,labelformat=simple,labelsep=space,justification=raggedright,singlelinecheck=false,position=top,skip=3pt,hypcap=true}

    % Crop margins: LEFT BOTTOM RIGHT TOP.
    % Blackout and Rooftop: 1920 x 1080; Chalk and Tile Merge: 1280 x 720.
    % PNGs have no DPI metadata; 1 bp equals one source pixel at 72 dpi.
    % Use {0bp 0bp 0bp 0bp} to show a complete original frame.
    \newcommand{\AFSBlackoutCrop}{1480bp 50bp 122bp 852bp}
    \newcommand{\AFSChalkCrop}{150bp 77bp 740bp 473bp}
    \newcommand{\AFSRooftopCrop}{30bp 350bp 990bp 390bp}
    \newcommand{\AFSTileCrop}{350bp 443bp 350bp 108bp}

    \newcommand{\AFSMethodWidth}{0.09\linewidth}
    \newcommand{\AFSFrameWidth}{0.27\linewidth}
    \newcommand{\AFSRowGap}{1pt}
    \newcommand{\AFSPanelGap}{2pt}
    \newcommand{\AFSLabelFont}{\rmfamily\color{A2ZFigText}\fontsize{8}{9}\selectfont}

    \newcommand{\AFSMethod}[1]{%
        \begin{minipage}[c]{\AFSMethodWidth}
            \raggedright
            {\rmfamily\color{A2ZFigText}\fontsize{8.5}{10}\selectfont\strut\textbf{#1}\par}
        \end{minipage}%
    }

    % Arguments: [crop], timestamp, original PNG path, state label.
    \newcommand{\AFSFrame}[4][0bp 0bp 0bp 0bp]{%
        \begin{minipage}[c]{\AFSFrameWidth}
            \edef\AFSImageOptions{trim=#1,clip,width=\the\linewidth}
            \vbox{%
                \offinterlineskip
                \hbox to\linewidth{\hfil{\AFSLabelFont\strut #2}\hfil}%
                \vskip1pt
                \hbox{\expandafter\includegraphics\expandafter[\AFSImageOptions]{#3}}%
                \vskip1pt
                \hbox to\linewidth{\hfil{\AFSLabelFont\strut #4}\hfil}%
            }%
        \end{minipage}%
    }

    % All three cards stay in one unbreakable horizontal row.
    % Arguments: method label, frame 1, frame 2, frame 3.
    \newcommand{\AFSRow}[4]{%
        \noindent\hbox to\linewidth{%
            \AFSMethod{#1}\hfil#2\hfil#3\hfil#4%
        }\par
    }

    \begin{subfigure}[t]{\linewidth}
        \caption{\texttt{Blackout Dispatch}: Confirm Gating}
        \label{fig:afs_blackout}
        \AFSRow{Uniform}%
            {\AFSFrame[\AFSBlackoutCrop]{1,013.8\,ms}{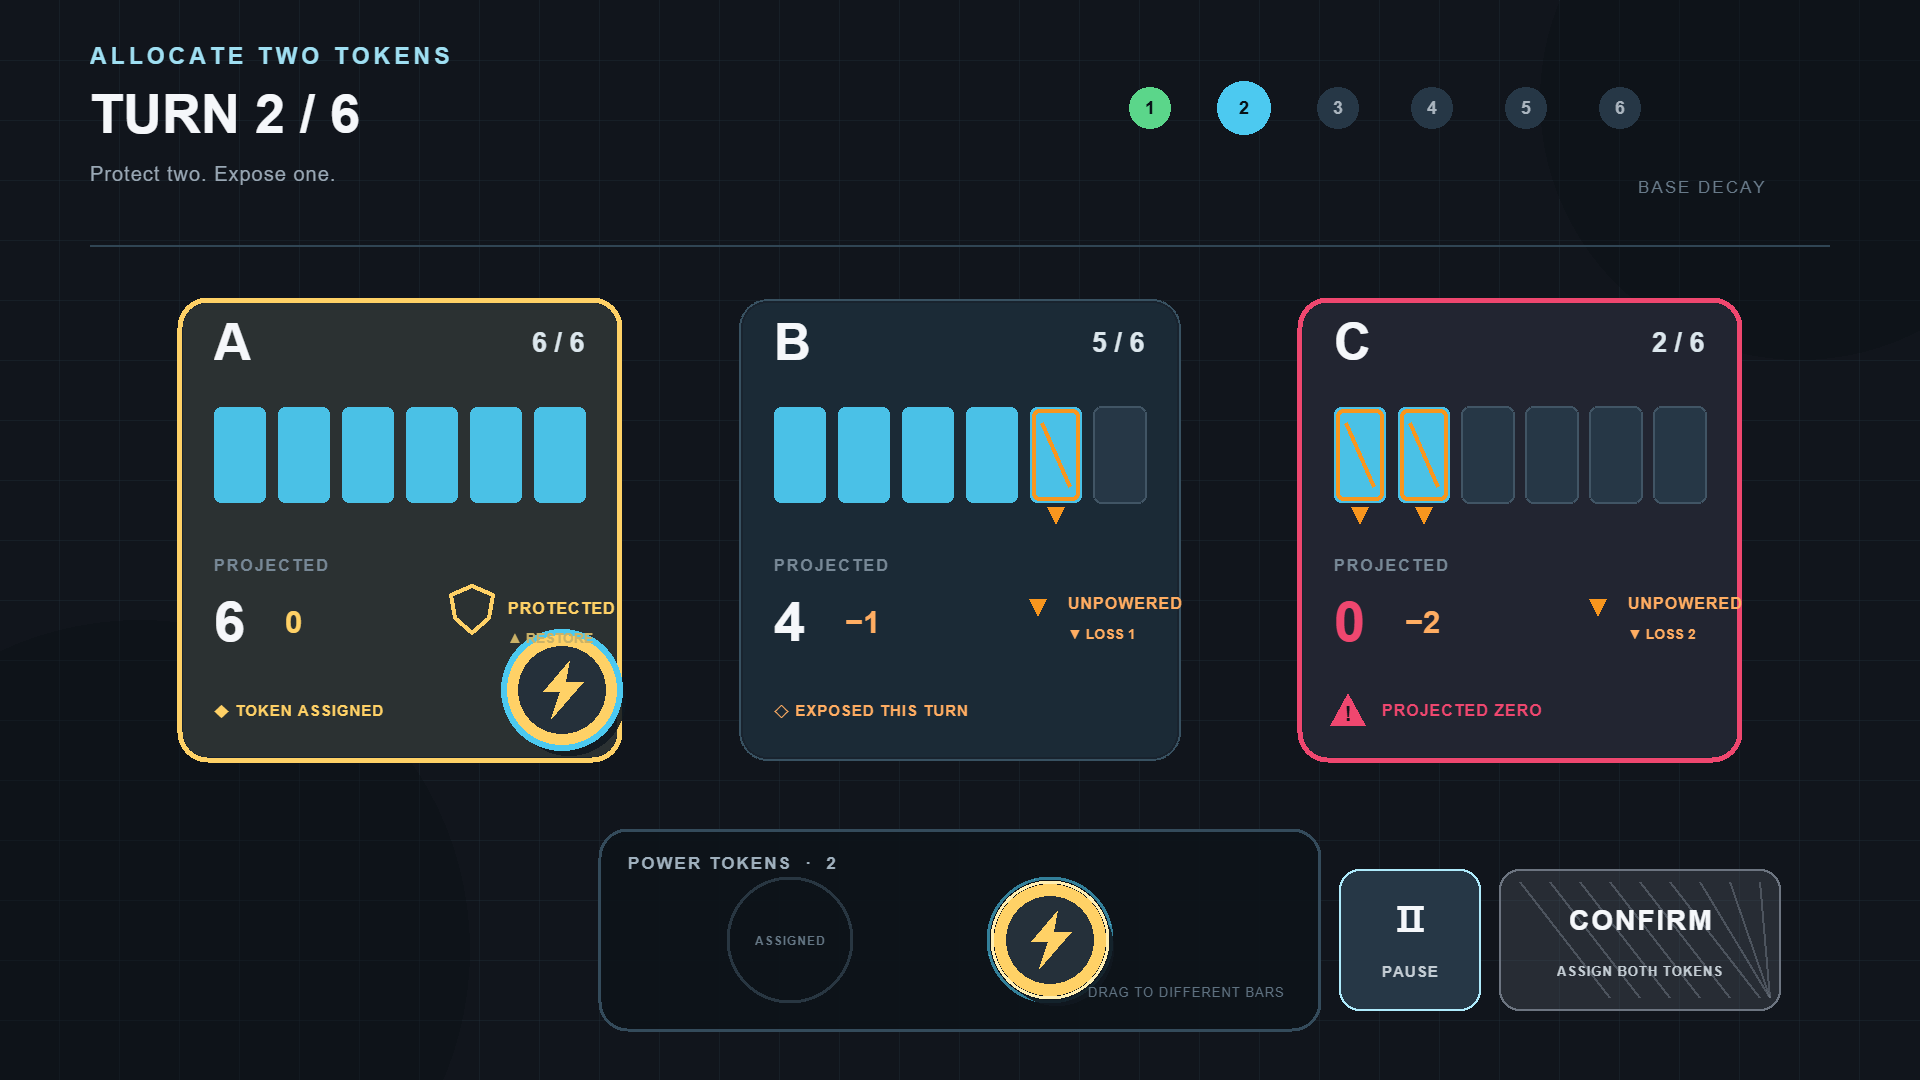}{Incomplete Allocation}}%
            {\AFSFrame[\AFSBlackoutCrop]{1,535.7\,ms}{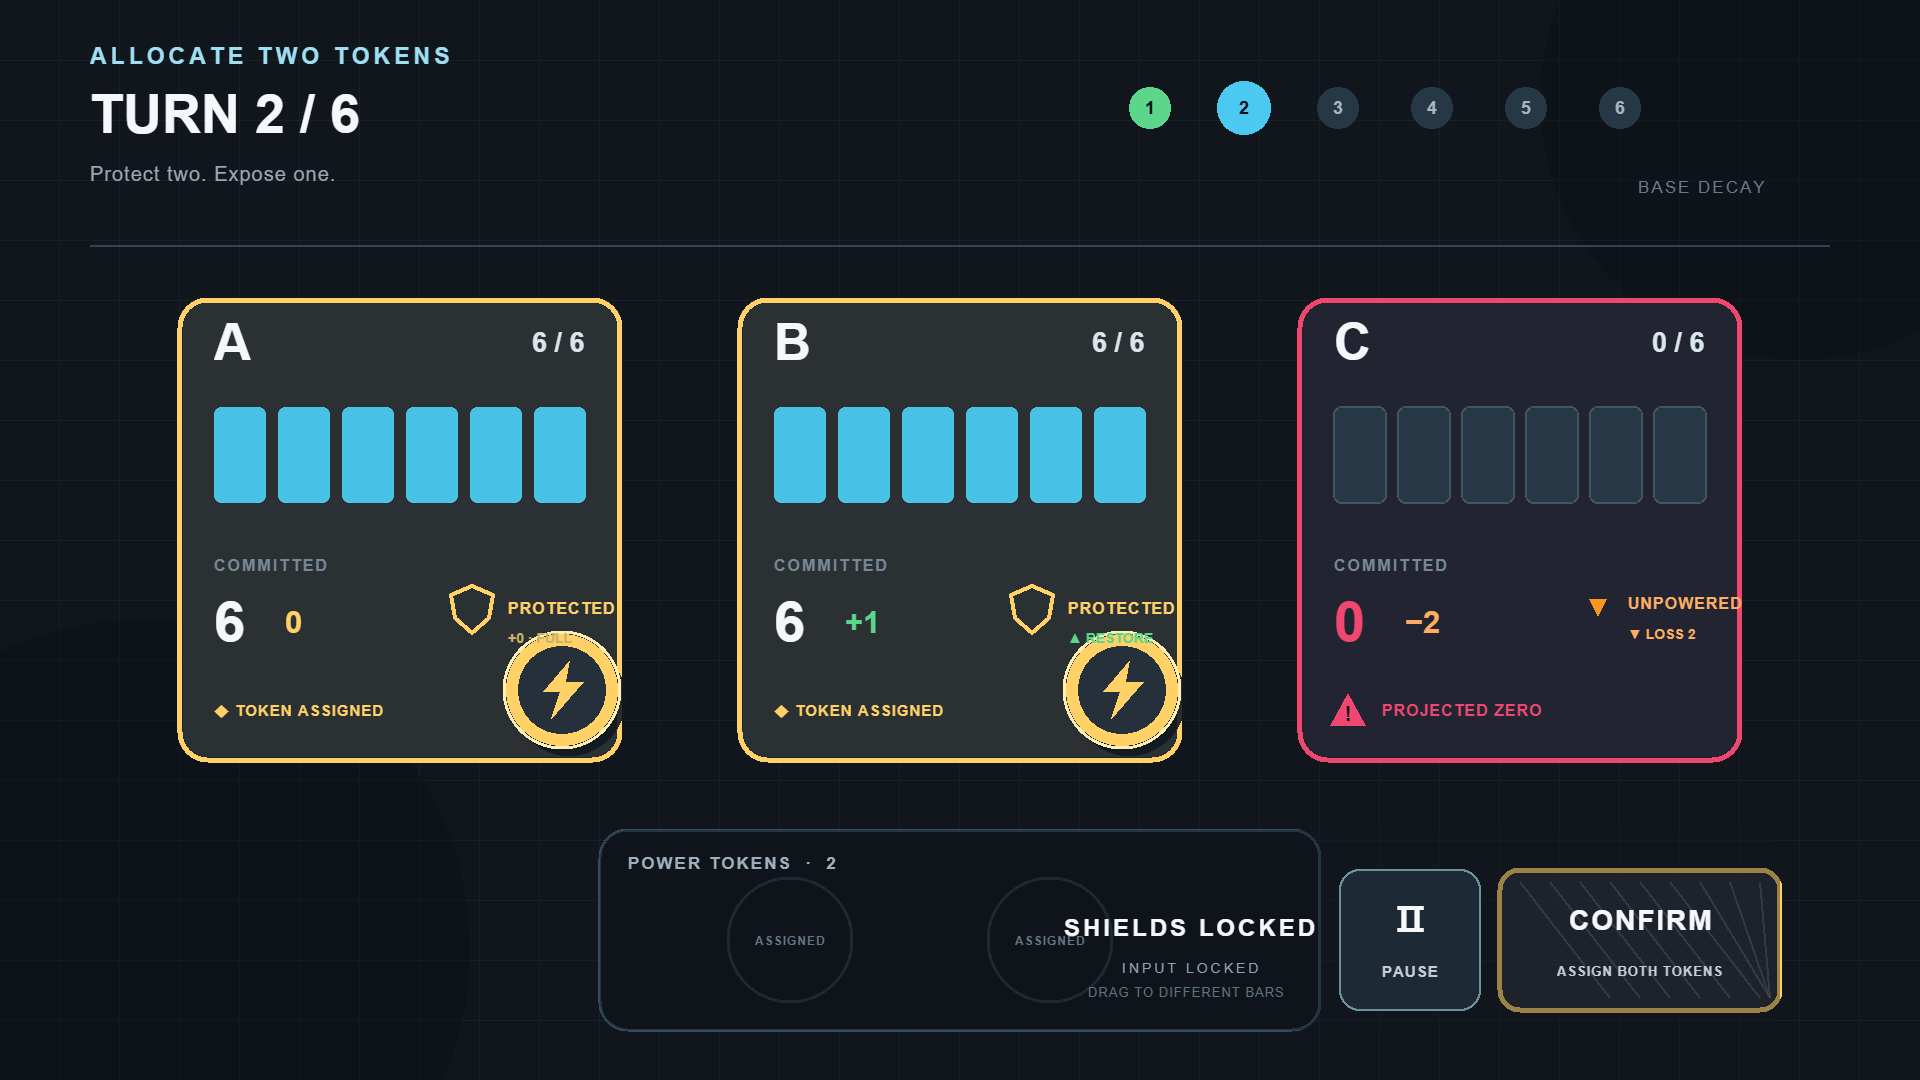}{After Confirmation}}%
            {\AFSFrame[\AFSBlackoutCrop]{2,014.6\,ms}{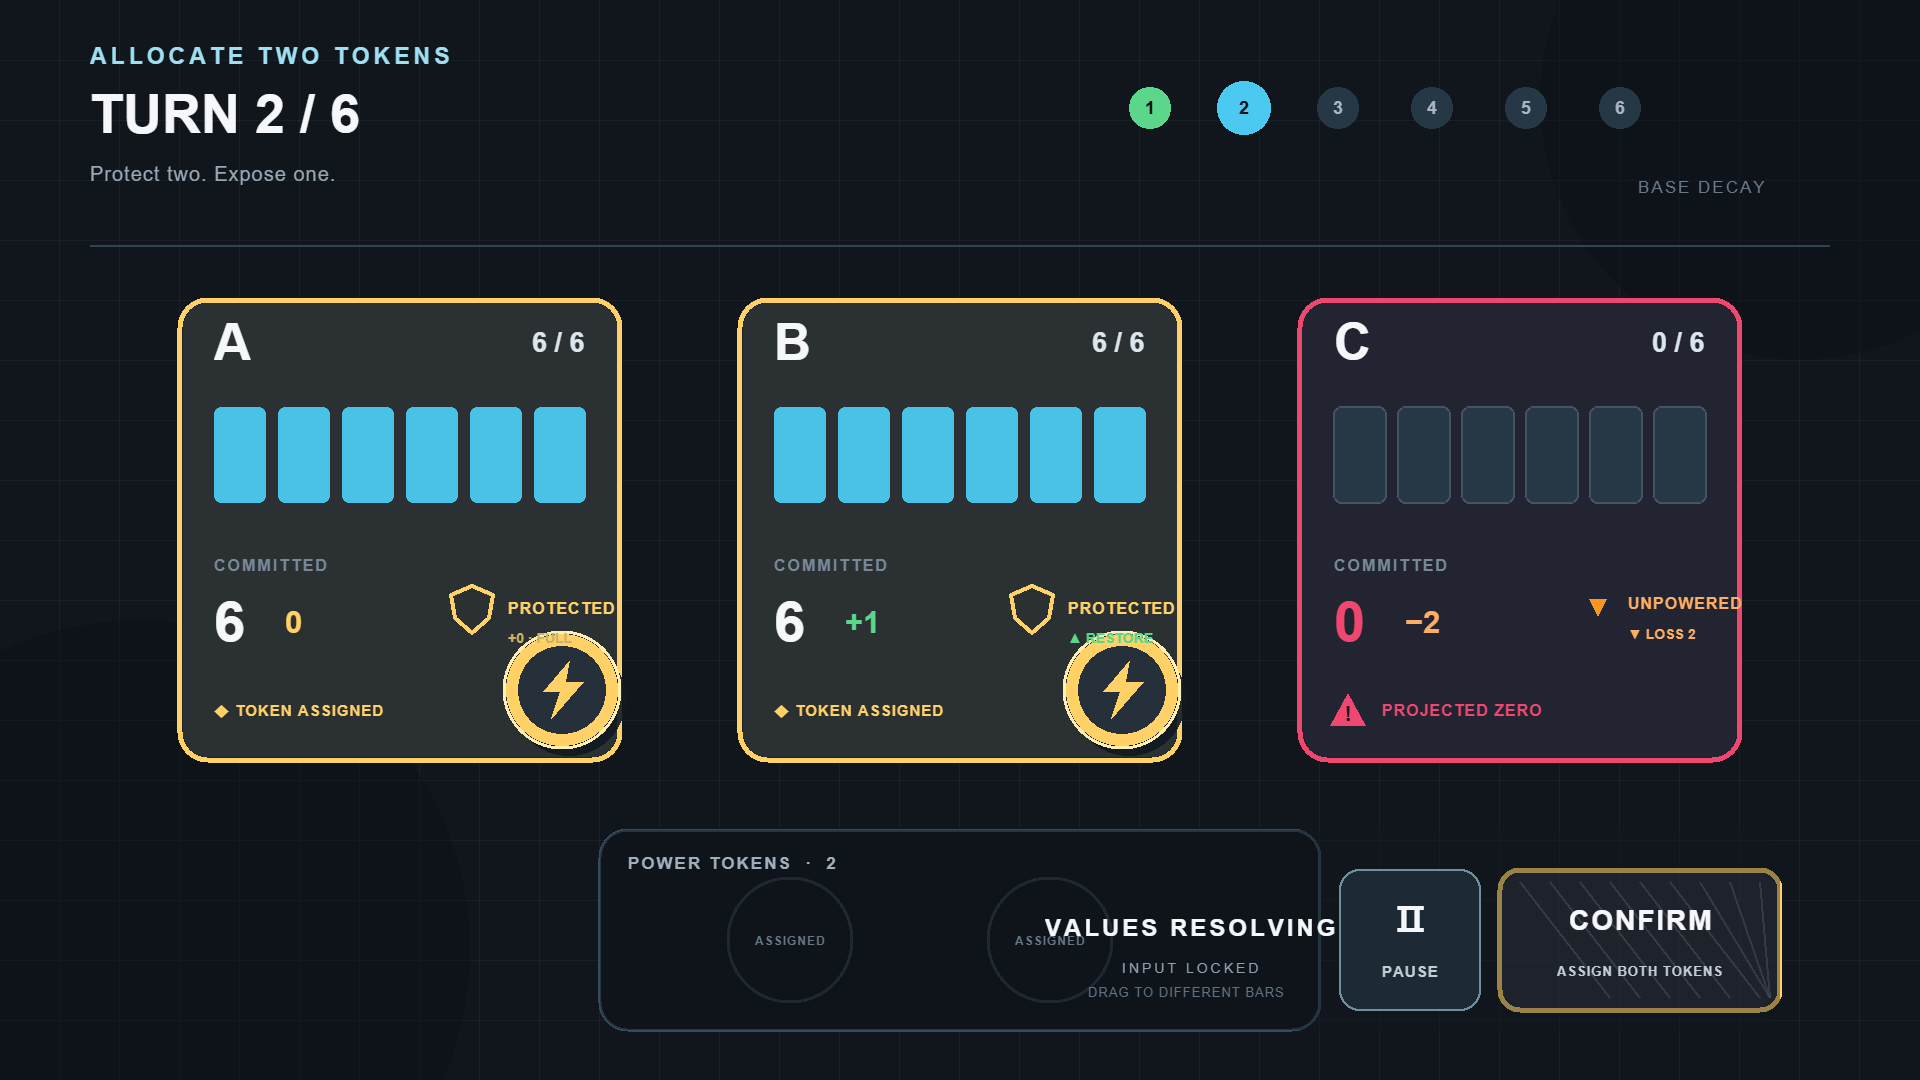}{During Resolution}}%

        \vspace{\AFSRowGap}
        \AFSRow{Adaptive}%
            {\AFSFrame[\AFSBlackoutCrop]{1,213.8\,ms}{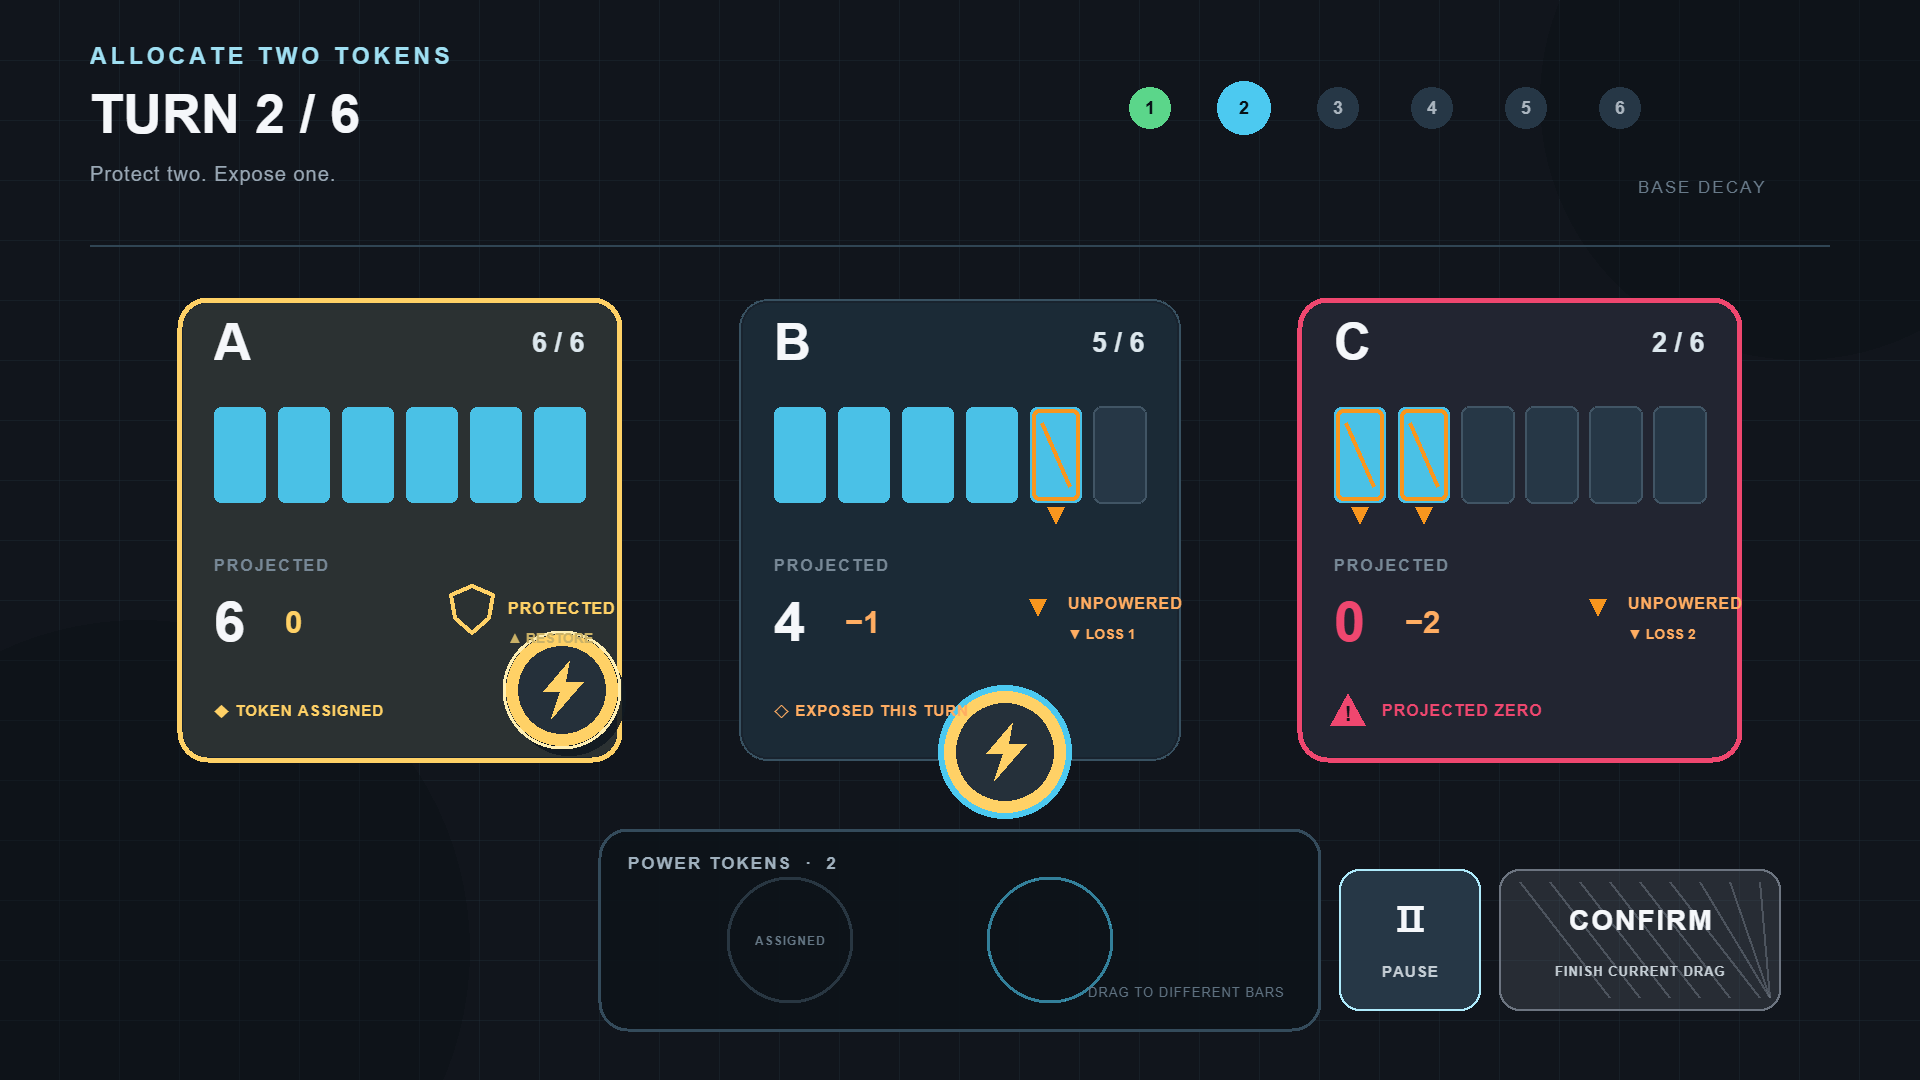}{Drag In Progress}}%
            {\AFSFrame[\AFSBlackoutCrop]{1,405.6\,ms}{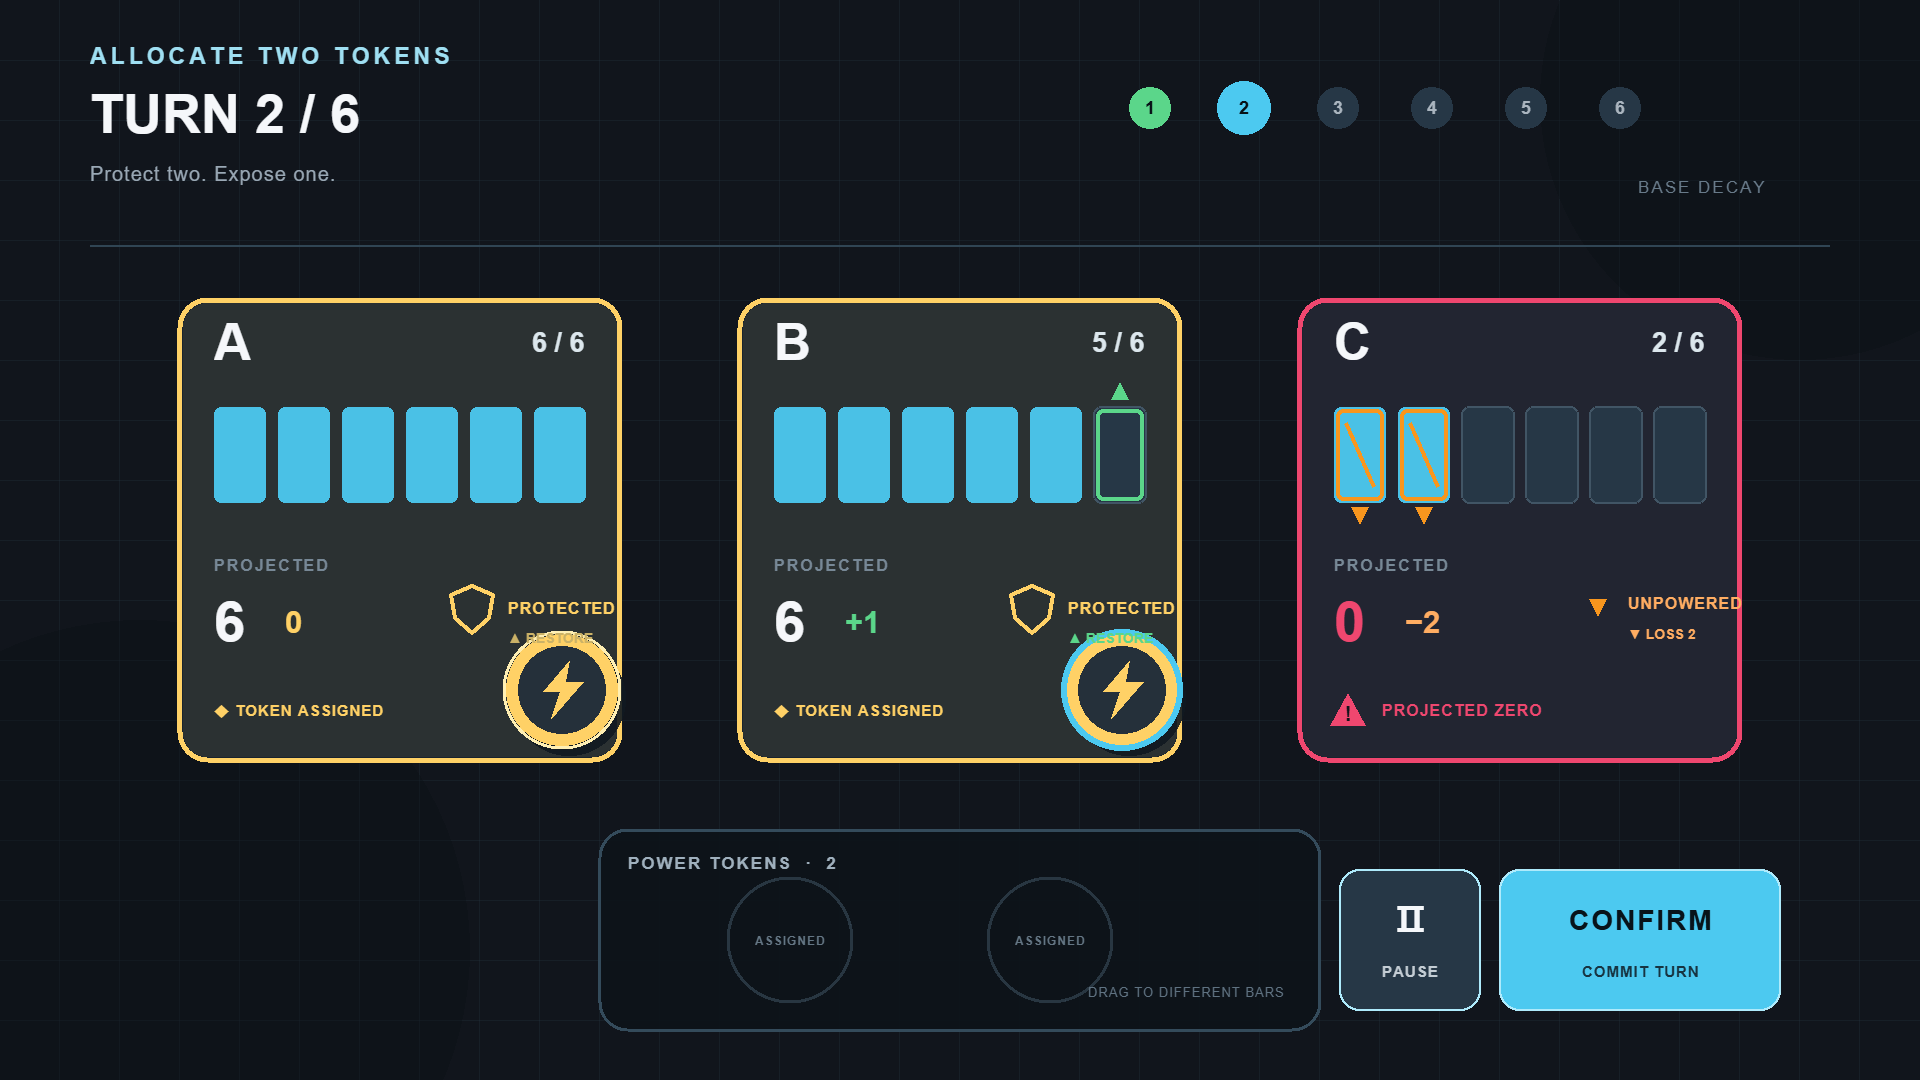}{Confirm Enabled}}%
            {\AFSFrame[\AFSBlackoutCrop]{1,535.7\,ms}{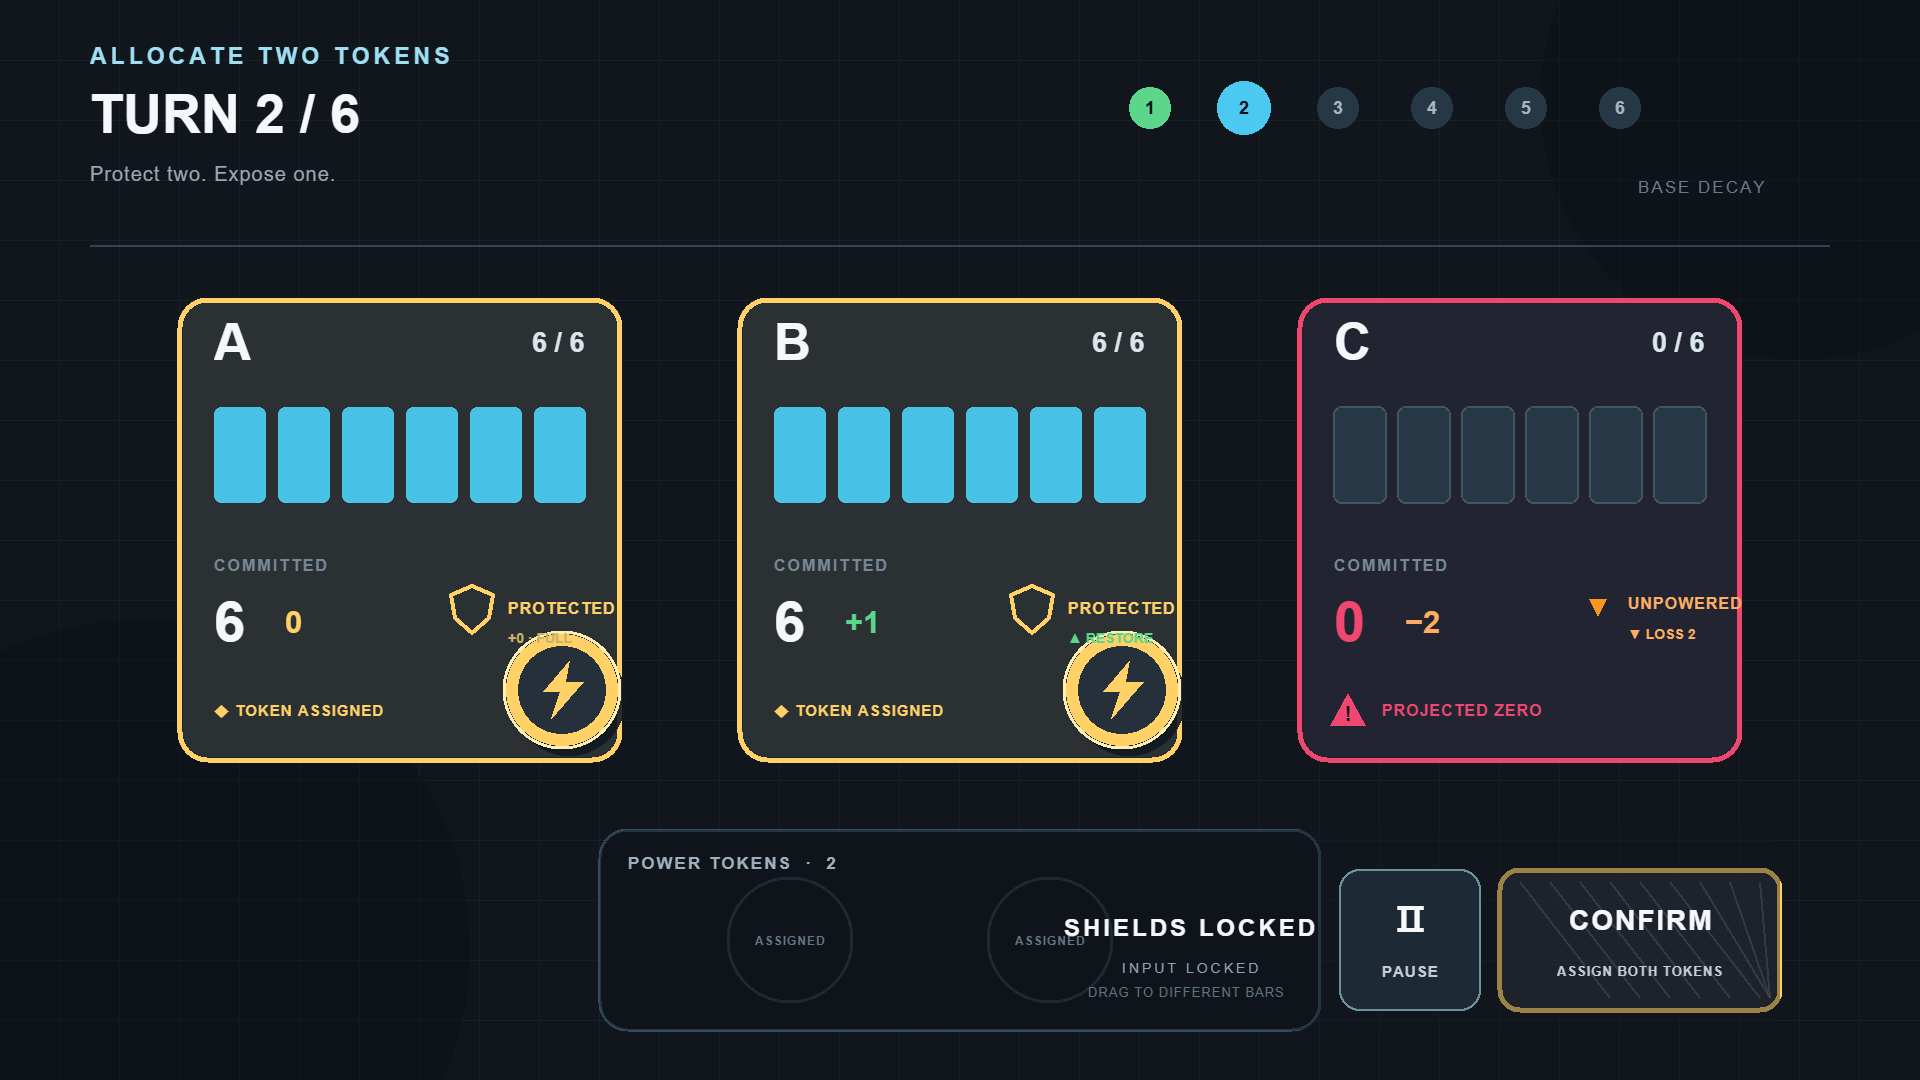}{After Confirmation}}%
    \end{subfigure}

    \vspace{\AFSPanelGap}

    \begin{subfigure}[t]{\linewidth}
        \caption{\texttt{Chalk Escape}: Path Removal}
        \label{fig:afs_chalk}
        \AFSRow{Uniform}%
            {\AFSFrame[\AFSChalkCrop]{9.8\,ms}{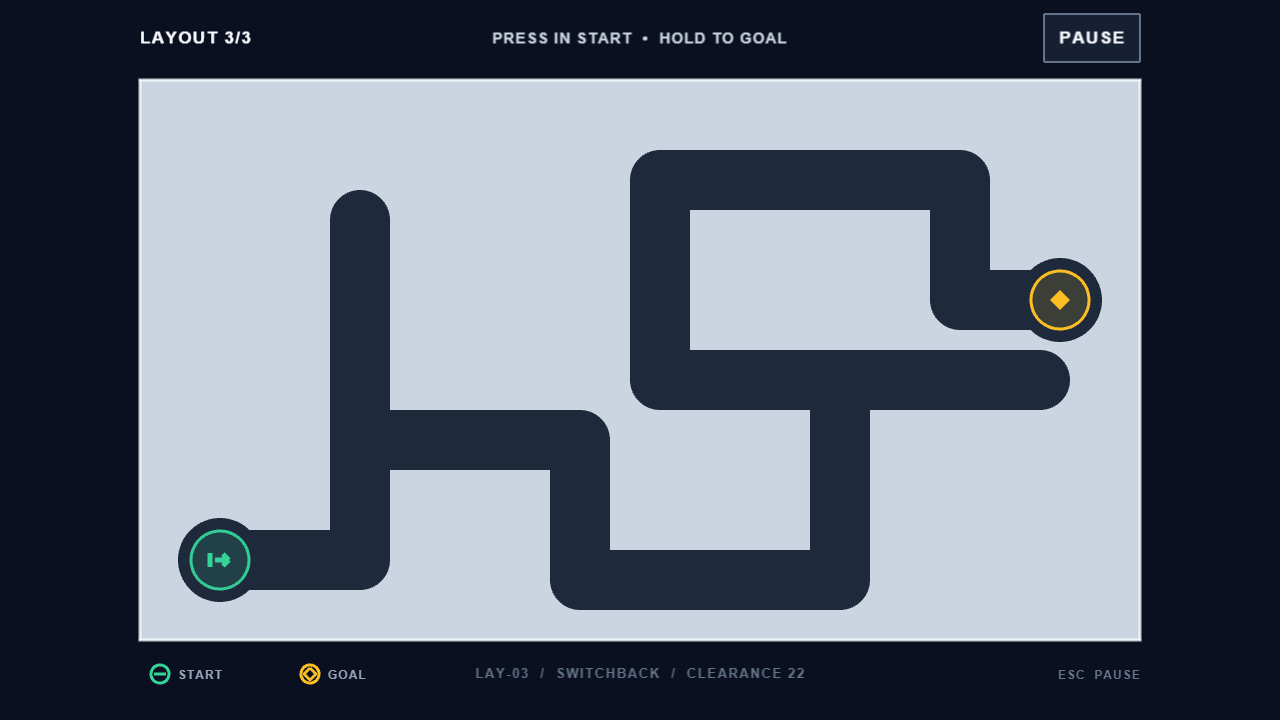}{No Path Yet}}%
            {\AFSFrame[\AFSChalkCrop]{508.4\,ms}{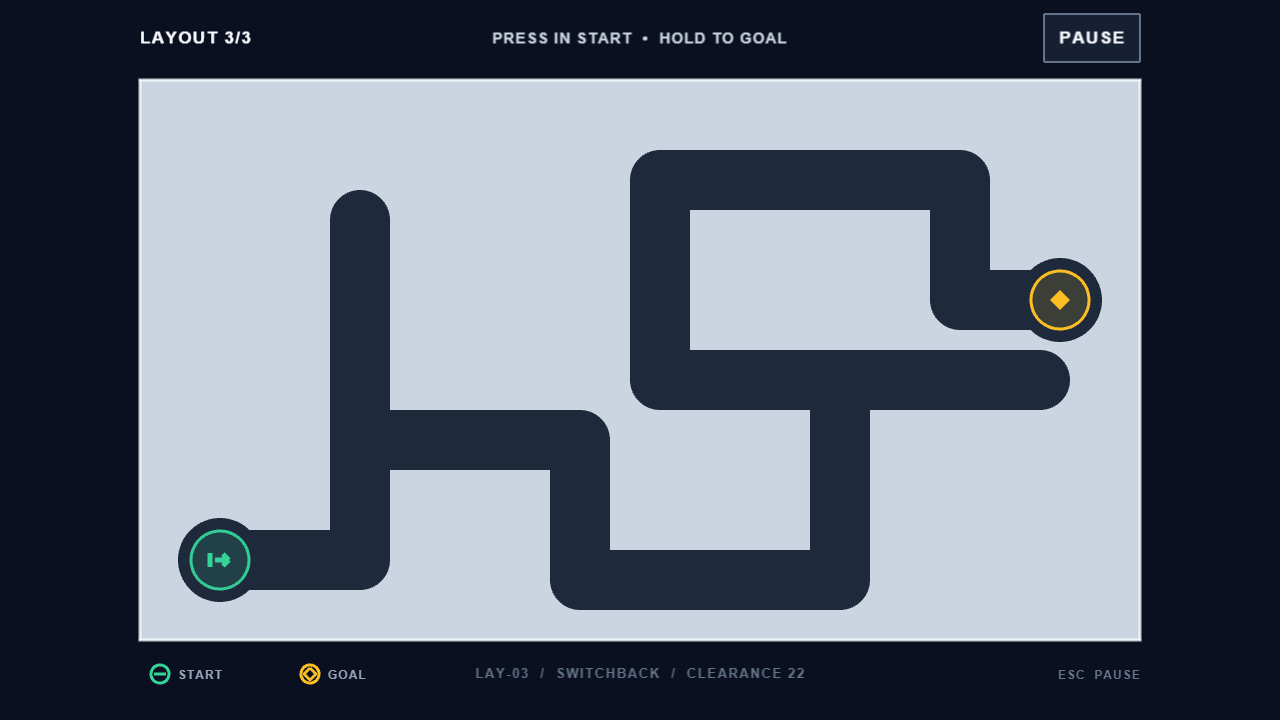}{No Path Yet}}%
            {\AFSFrame[\AFSChalkCrop]{1,009.2\,ms}{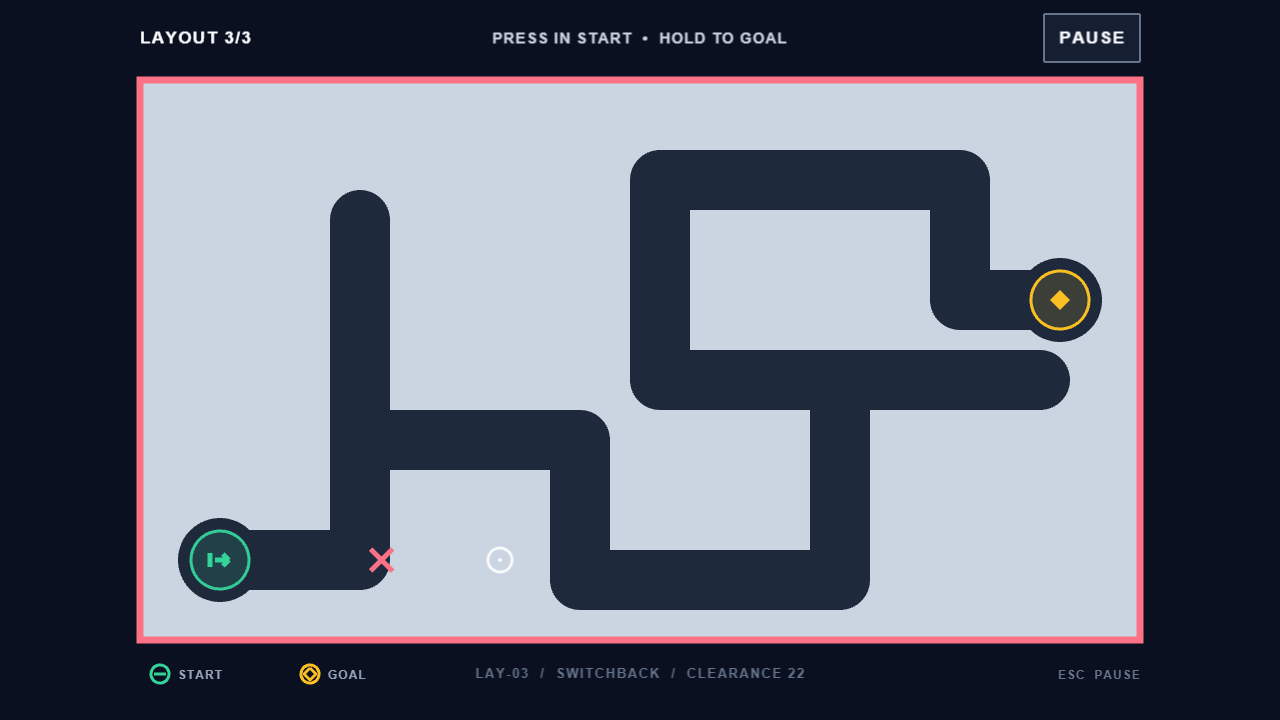}{Collision Aftermath}}%

        \vspace{\AFSRowGap}
        \AFSRow{Adaptive}%
            {\AFSFrame[\AFSChalkCrop]{9.8\,ms}{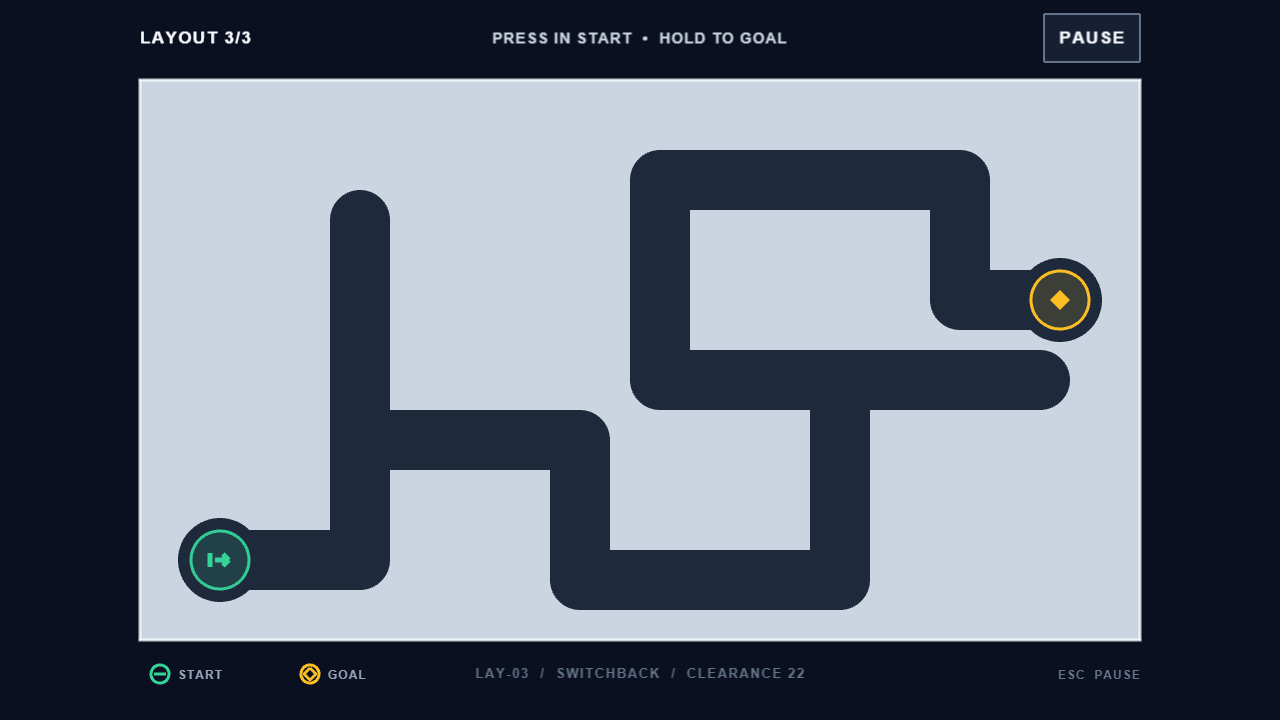}{No Path Yet}}%
            {\AFSFrame[\AFSChalkCrop]{867.0\,ms}{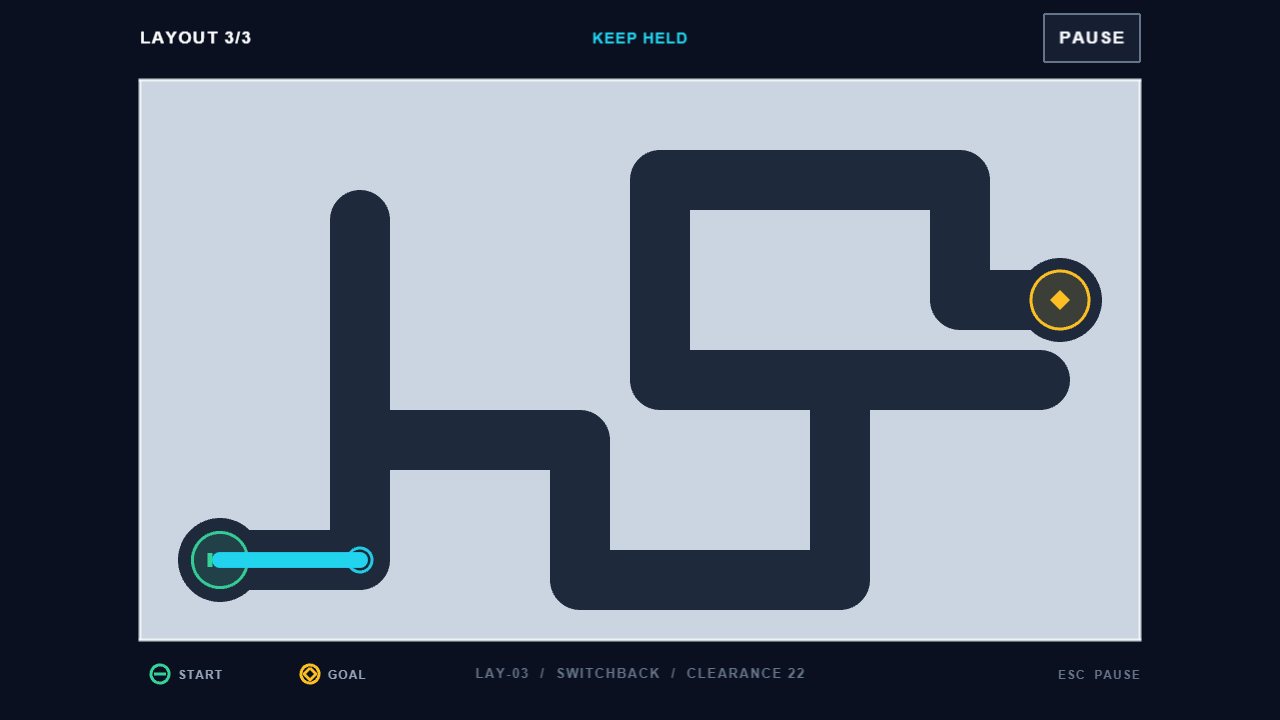}{Drawn Path}}%
            {\AFSFrame[\AFSChalkCrop]{941.1\,ms}{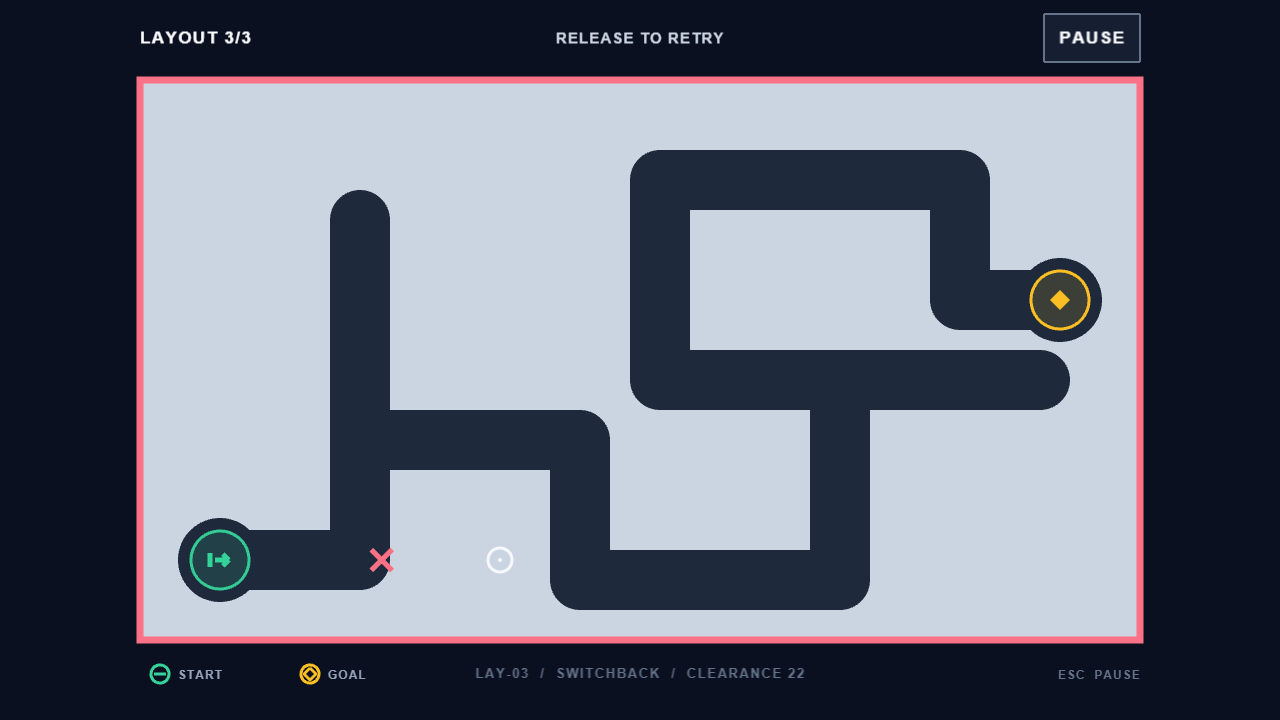}{Path Cleared}}%
    \end{subfigure}

    \vspace{\AFSPanelGap}

    \begin{subfigure}[t]{\linewidth}
        \caption{\texttt{Rooftop Rumble}: Hold and Defense Feedback}
        \label{fig:afs_rooftop}
        \AFSRow{Uniform}%
            {\AFSFrame[\AFSRooftopCrop]{2,511.7\,ms}{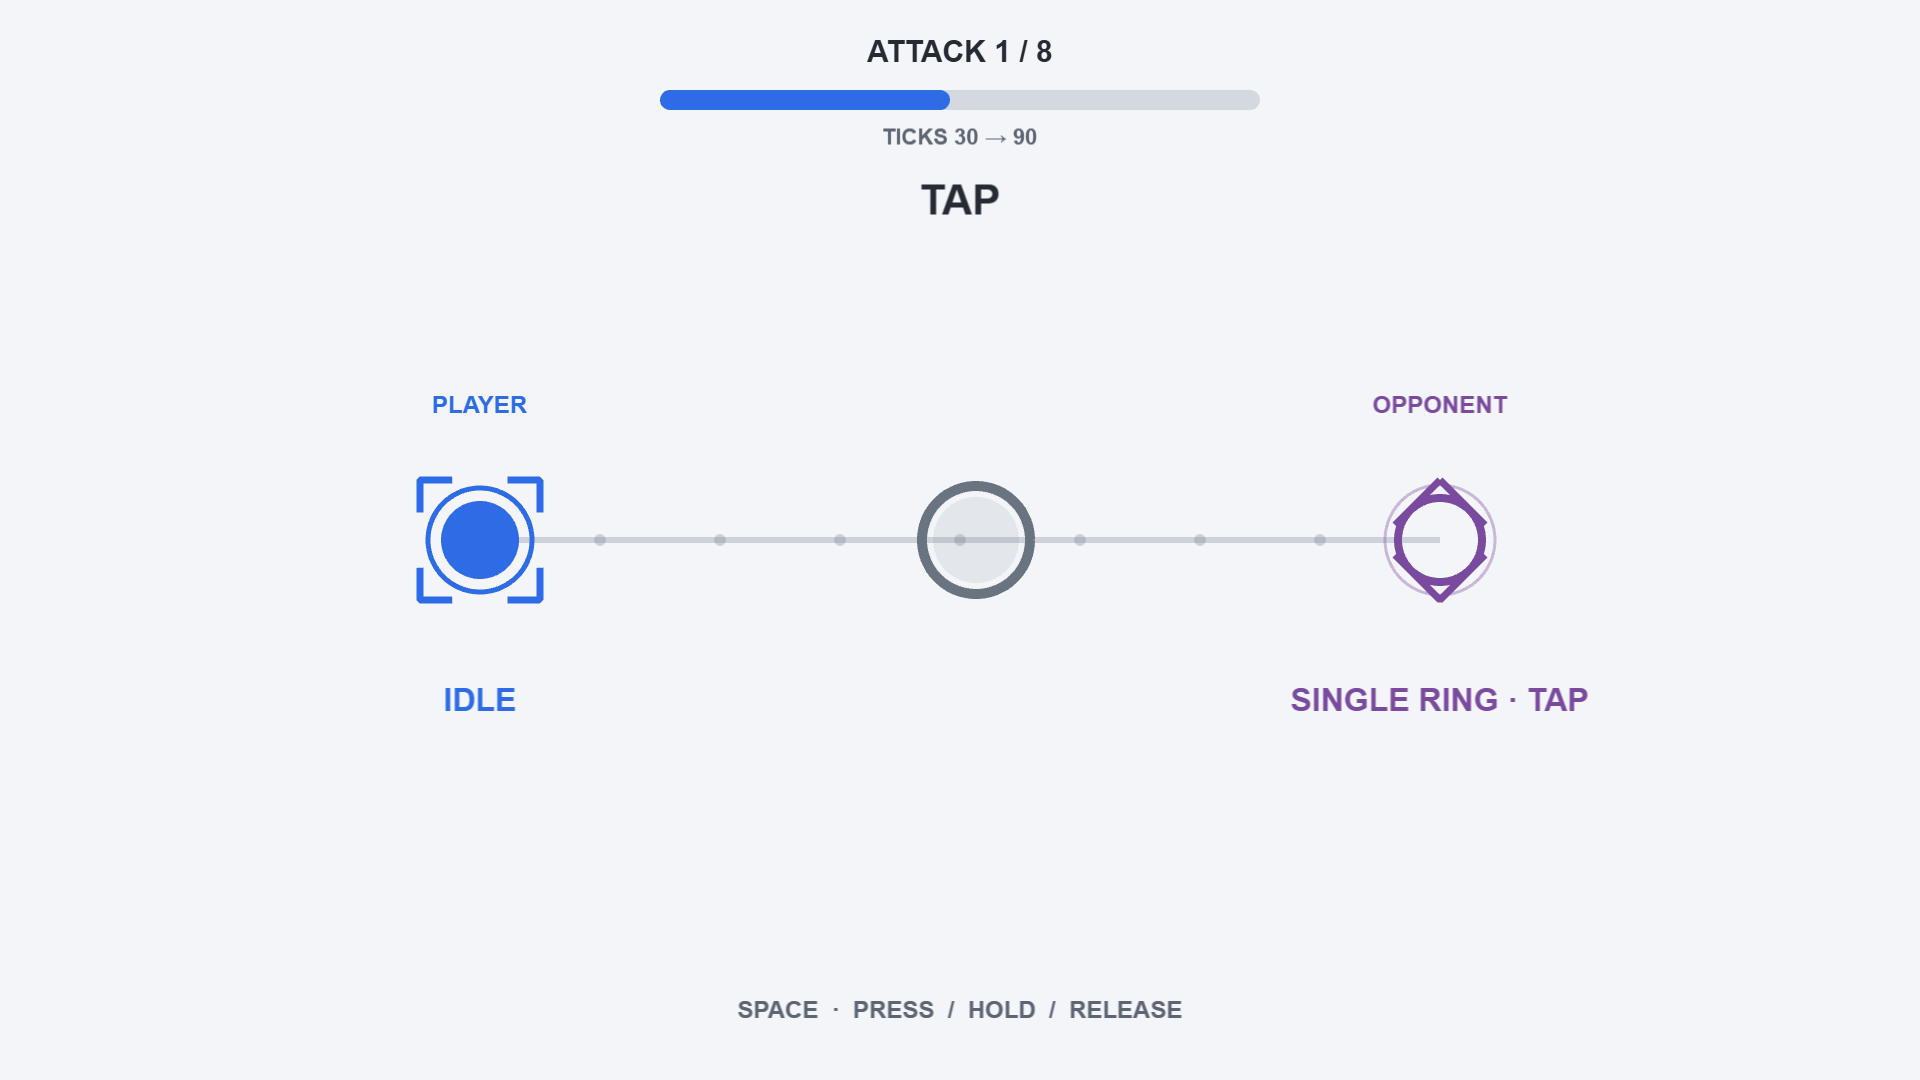}{Idle}}%
            {\AFSFrame[\AFSRooftopCrop]{3,017.0\,ms}{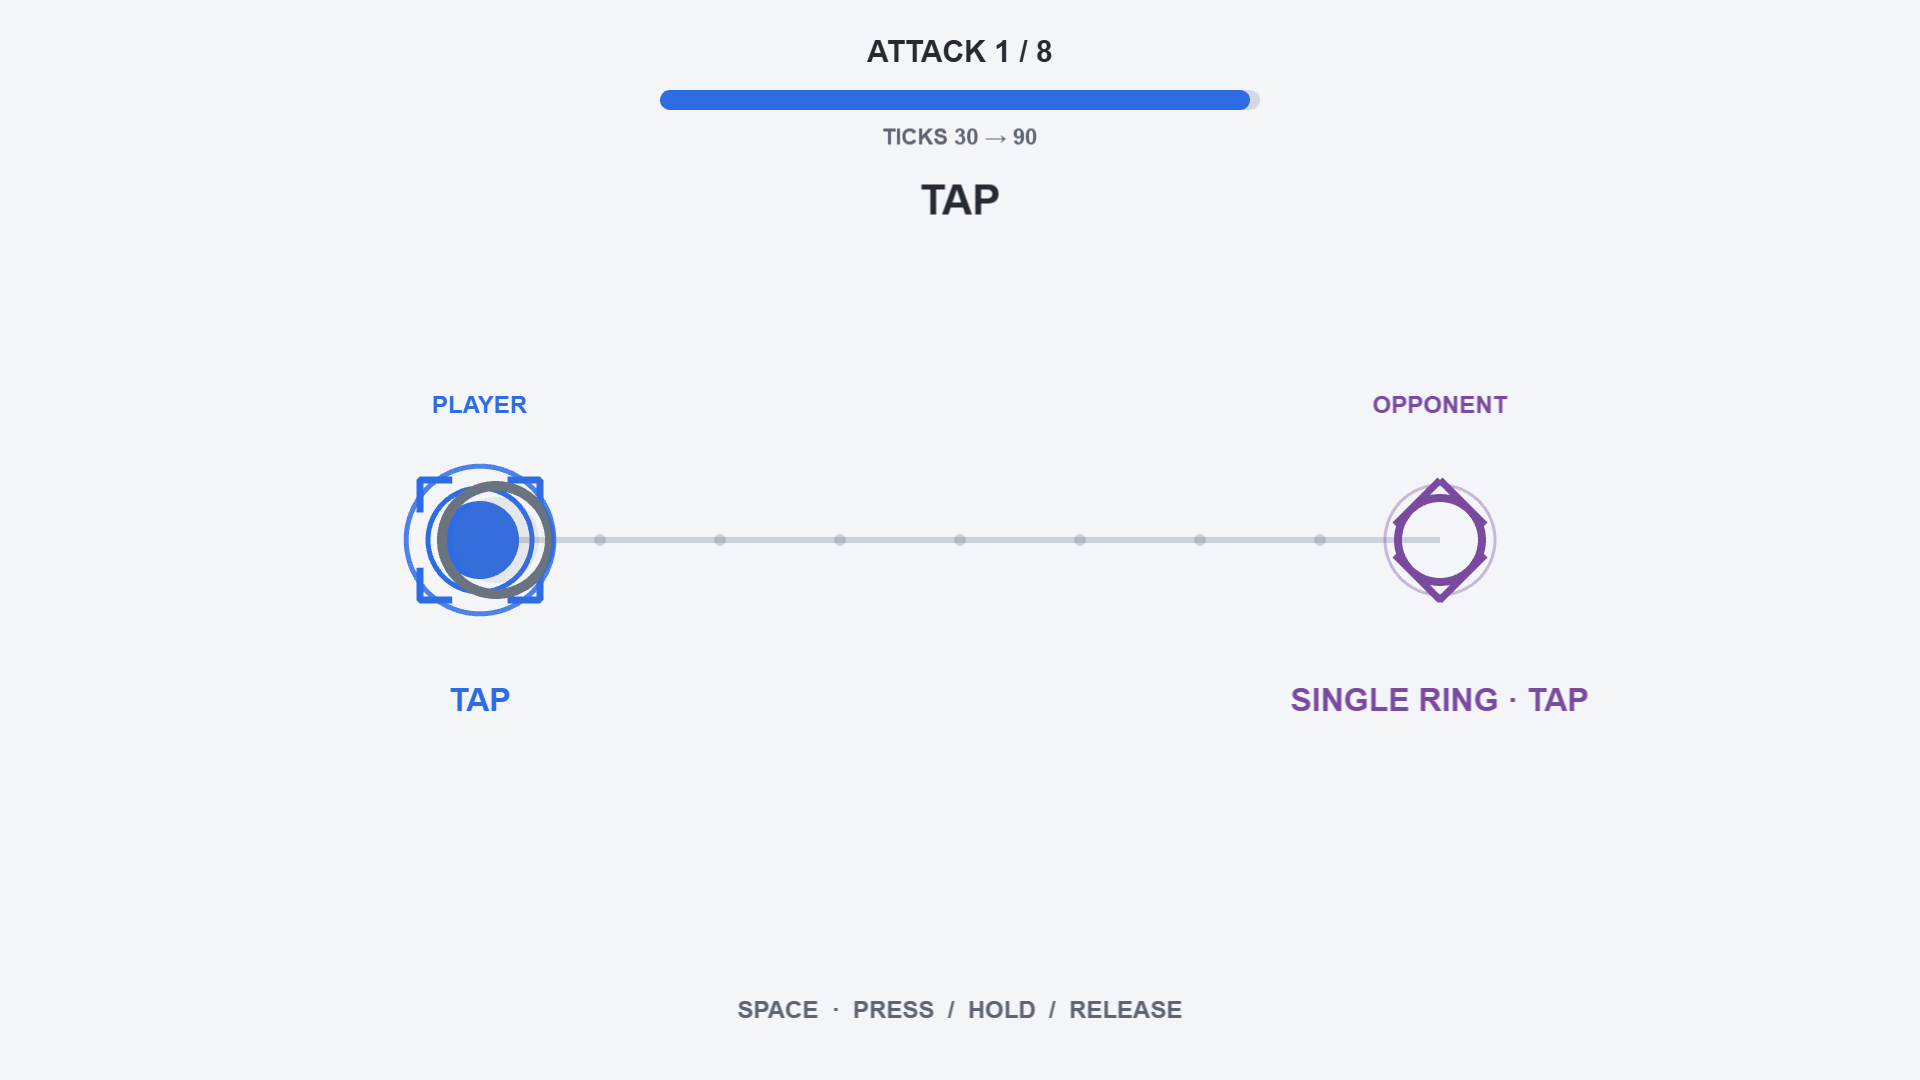}{Released: Tap}}%
            {\AFSFrame[\AFSRooftopCrop]{3,502.8\,ms}{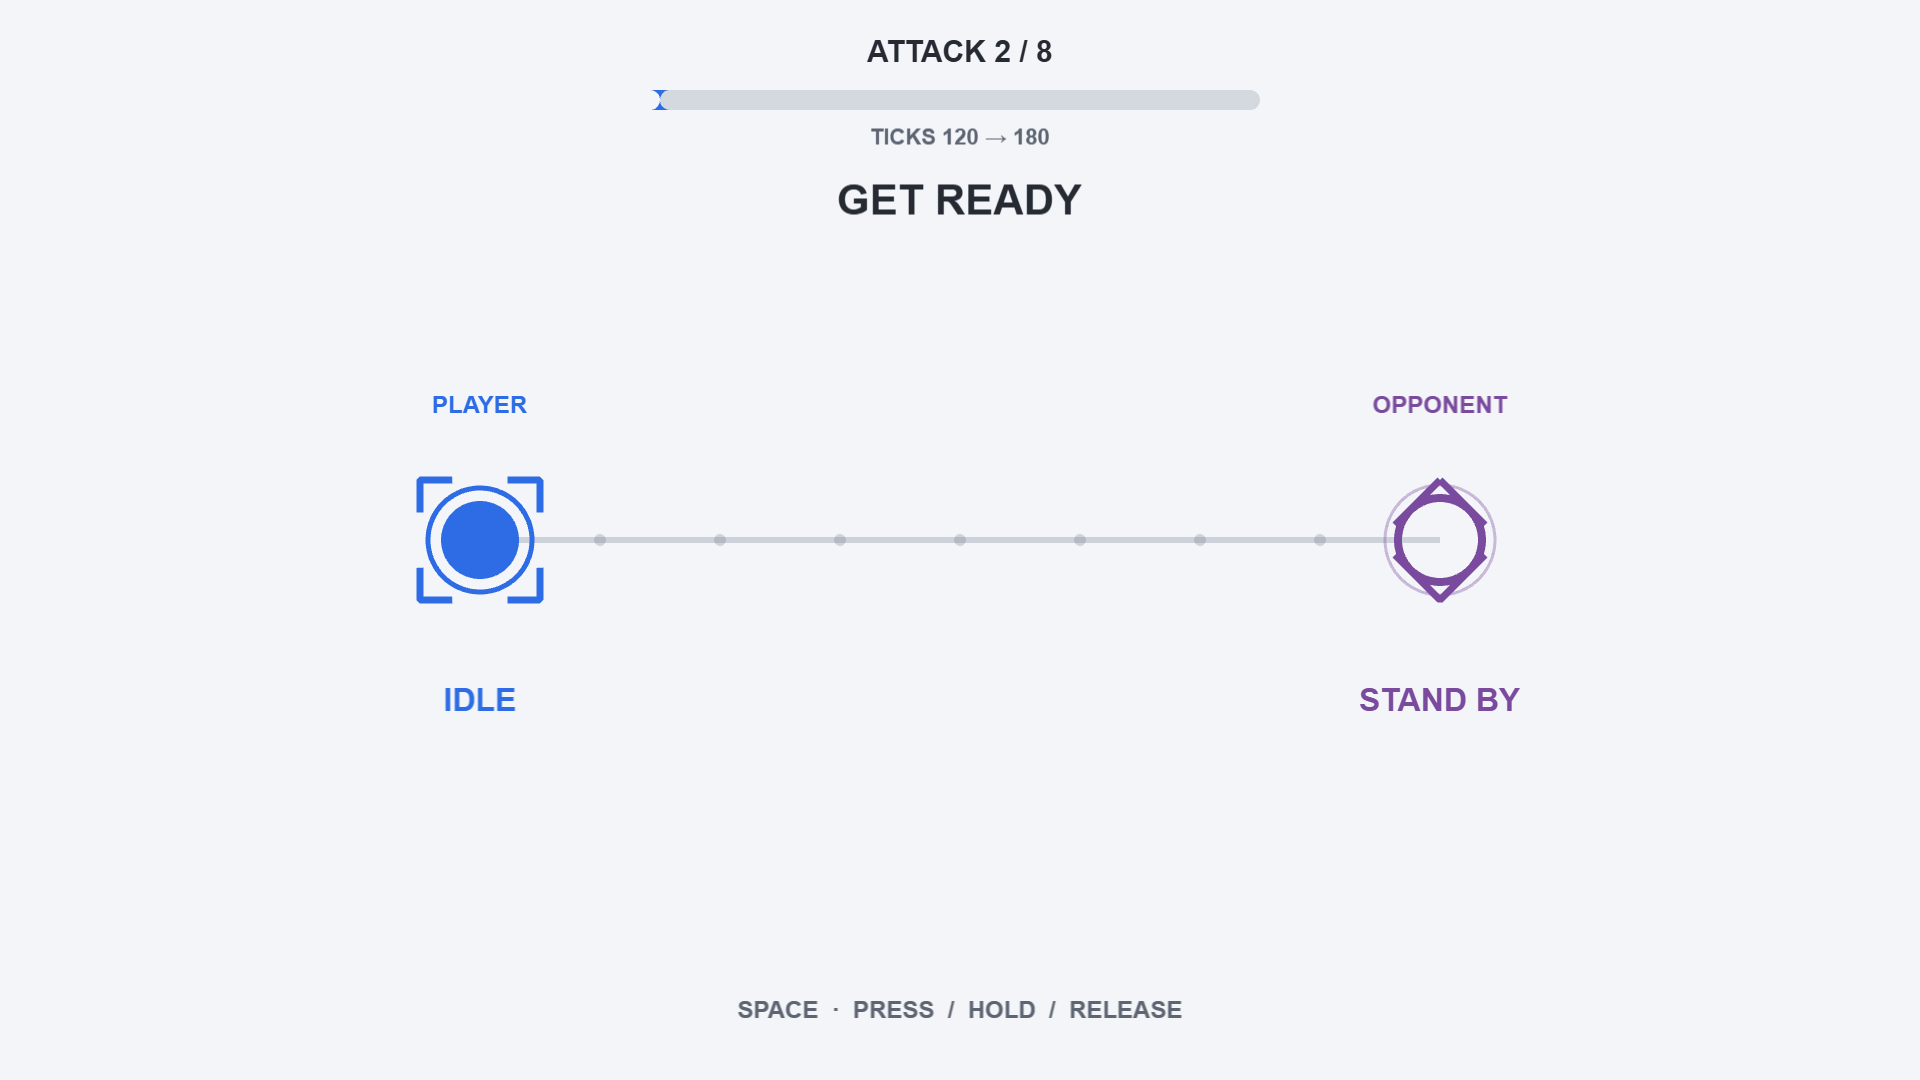}{Idle}}%

        \vspace{\AFSRowGap}
        \AFSRow{Adaptive}%
            {\AFSFrame[\AFSRooftopCrop]{2,924.0\,ms}{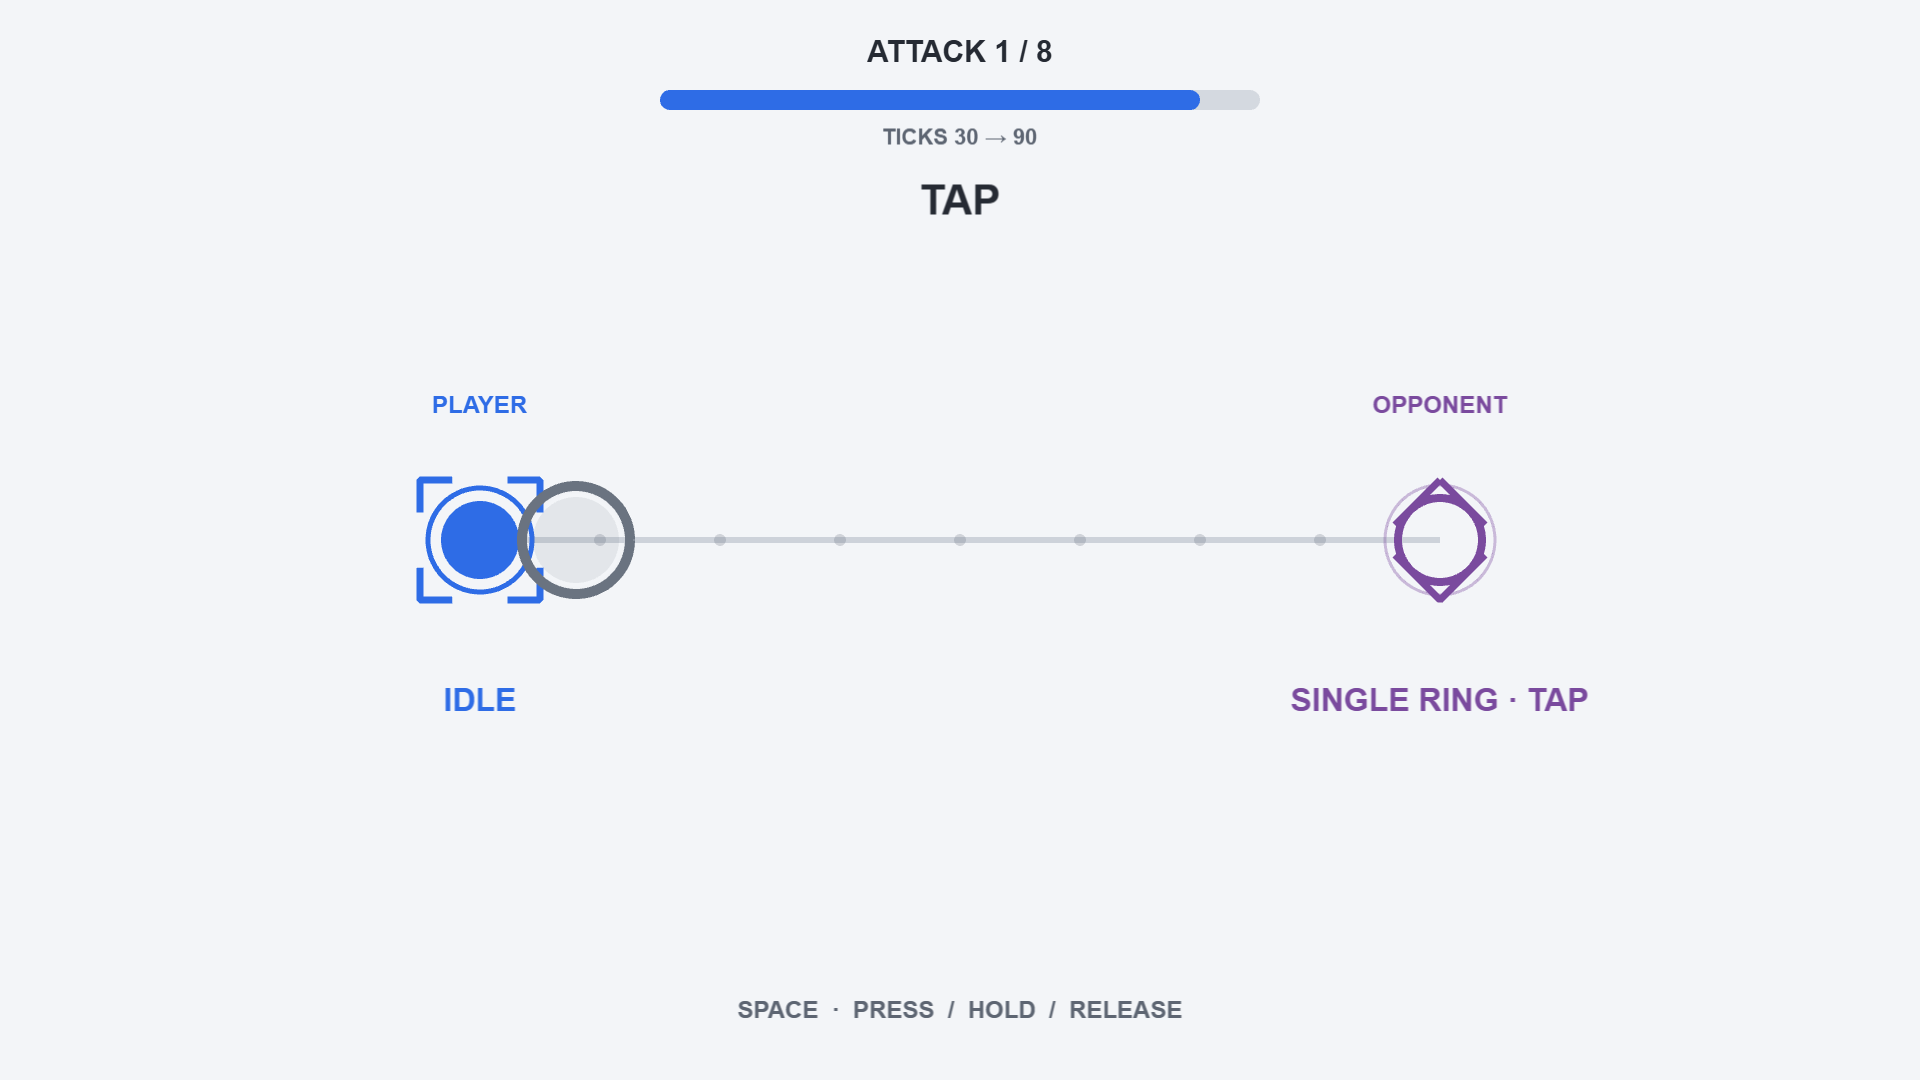}{Before Press}}%
            {\AFSFrame[\AFSRooftopCrop]{2,981.2\,ms}{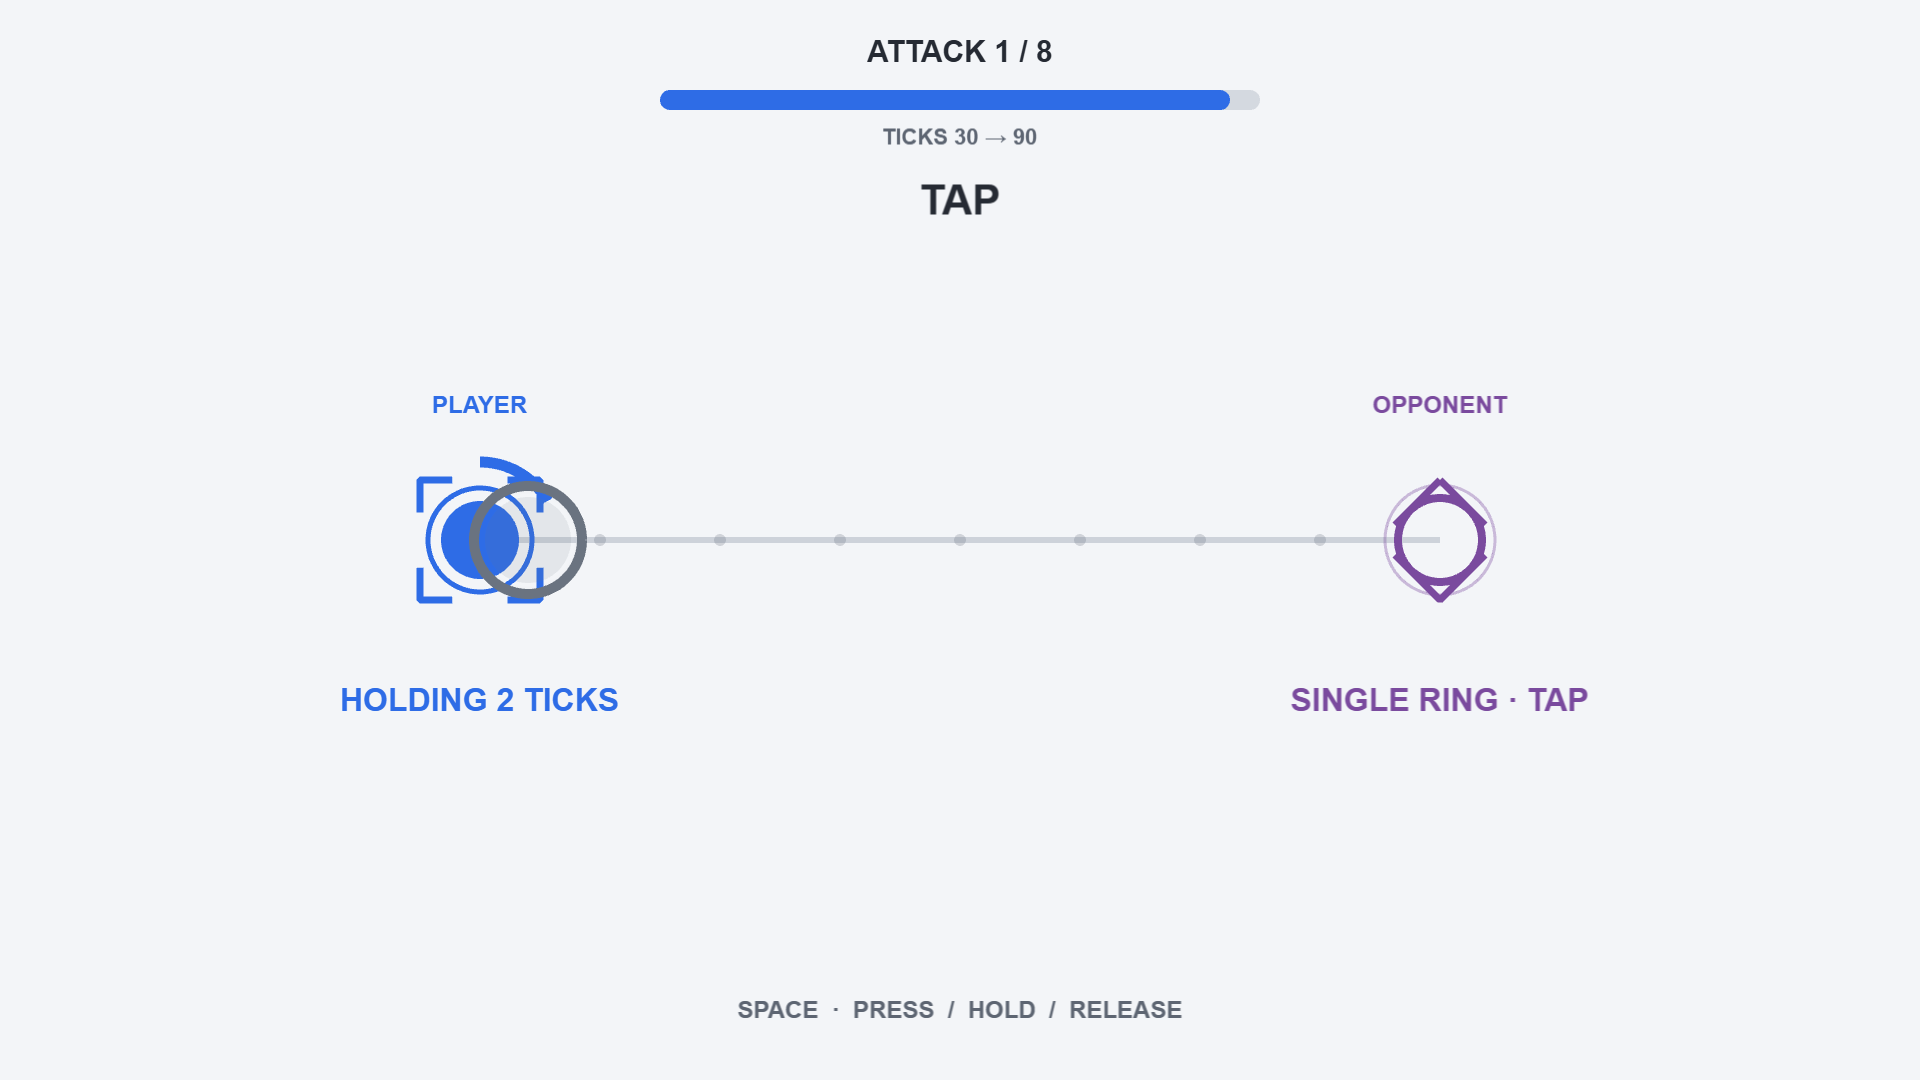}{Holding 2 Ticks}}%
            {\AFSFrame[\AFSRooftopCrop]{3,053.6\,ms}{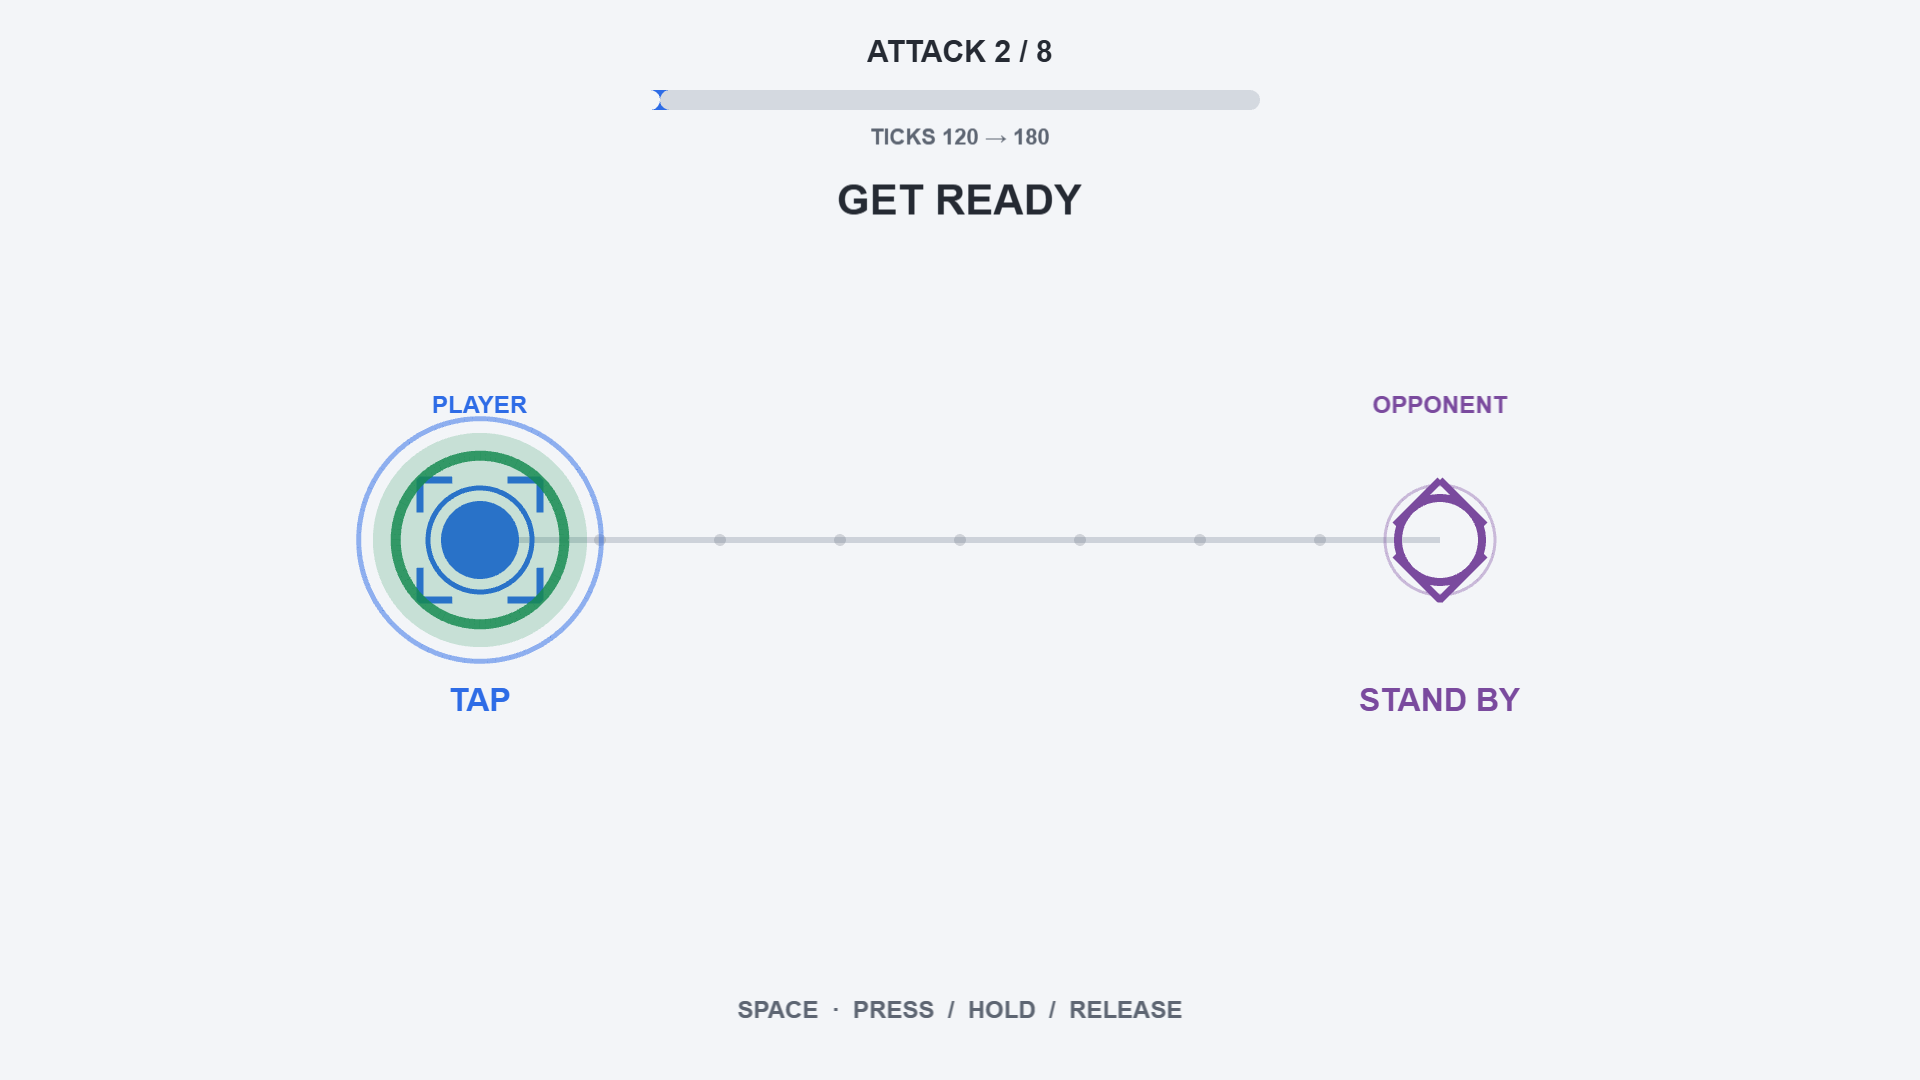}{Defense Feedback}}%
    \end{subfigure}

    \vspace{\AFSPanelGap}

    \begin{subfigure}[t]{\linewidth}
        \caption{\texttt{Tile Merge}: Merge Animation}
        \label{fig:afs_tile_merge}
        \AFSRow{Uniform}%
            {\AFSFrame[\AFSTileCrop]{7.3\,ms}{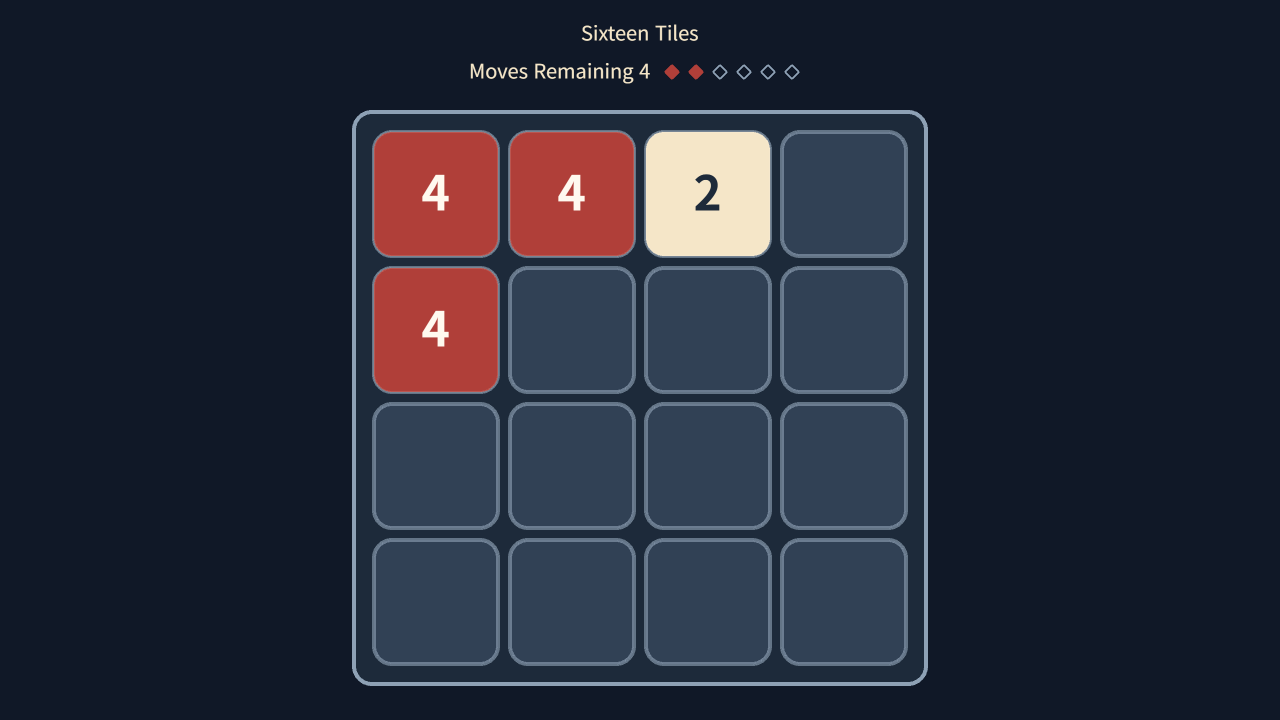}{Before Move}}%
            {\AFSFrame[\AFSTileCrop]{506.3\,ms}{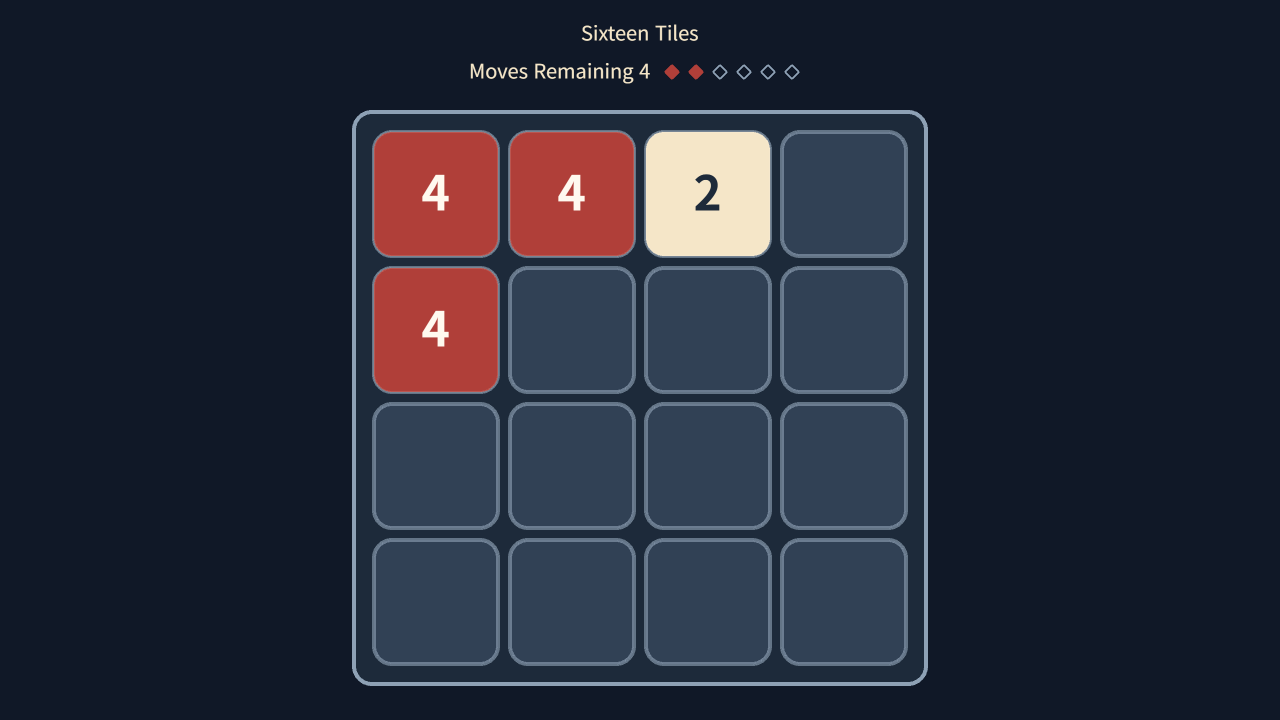}{Before Move}}%
            {\AFSFrame[\AFSTileCrop]{1,006.0\,ms}{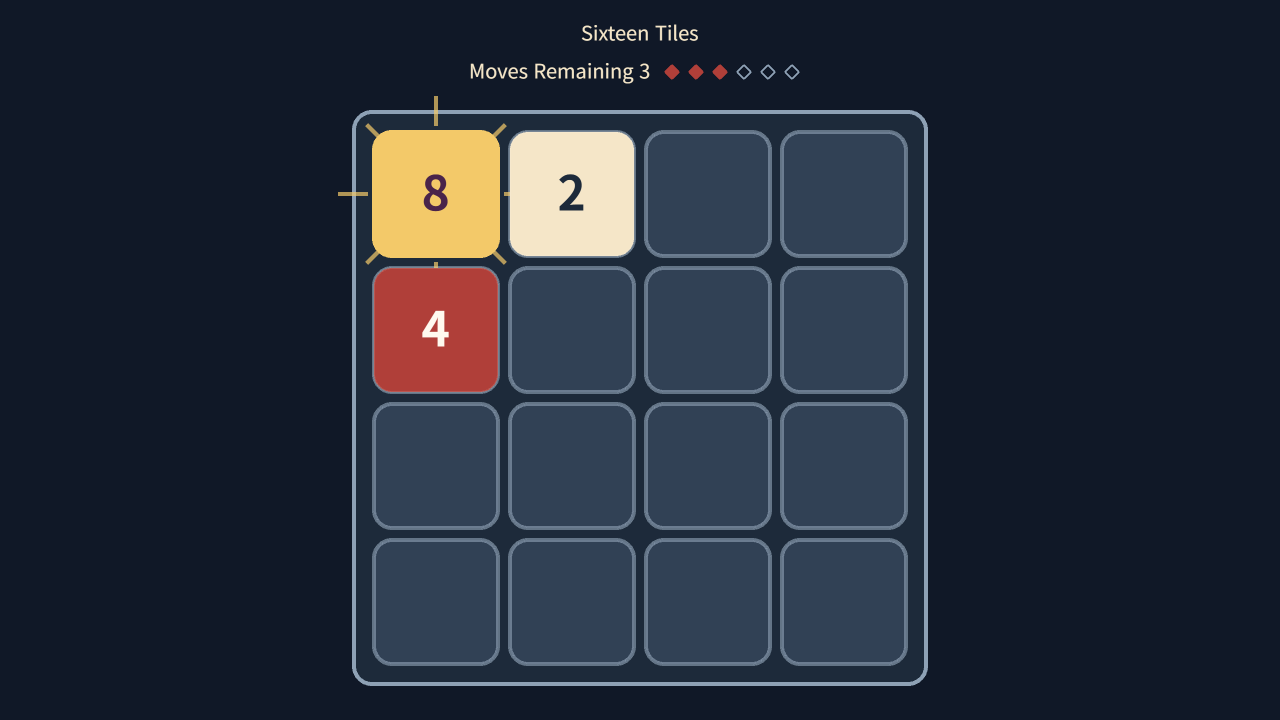}{After Merge}}%

        \vspace{\AFSRowGap}
        \AFSRow{Adaptive}%
            {\AFSFrame[\AFSTileCrop]{540.8\,ms}{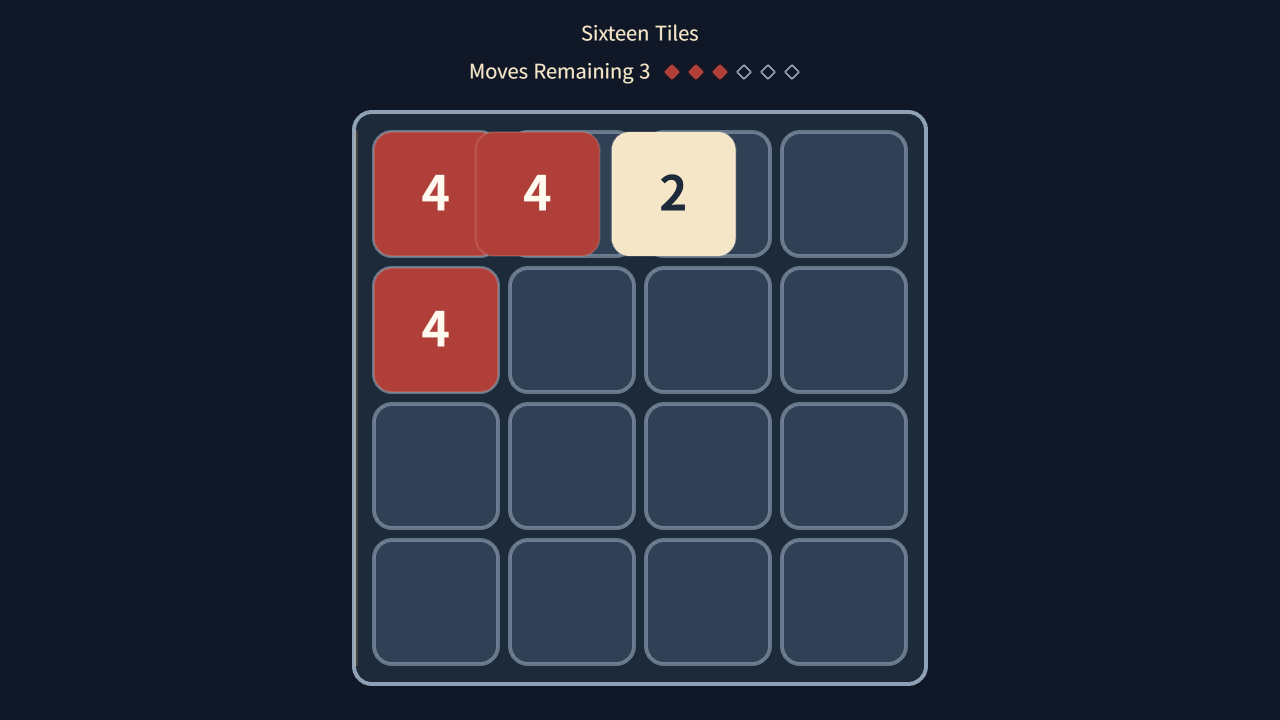}{Tiles Converging}}%
            {\AFSFrame[\AFSTileCrop]{606.2\,ms}{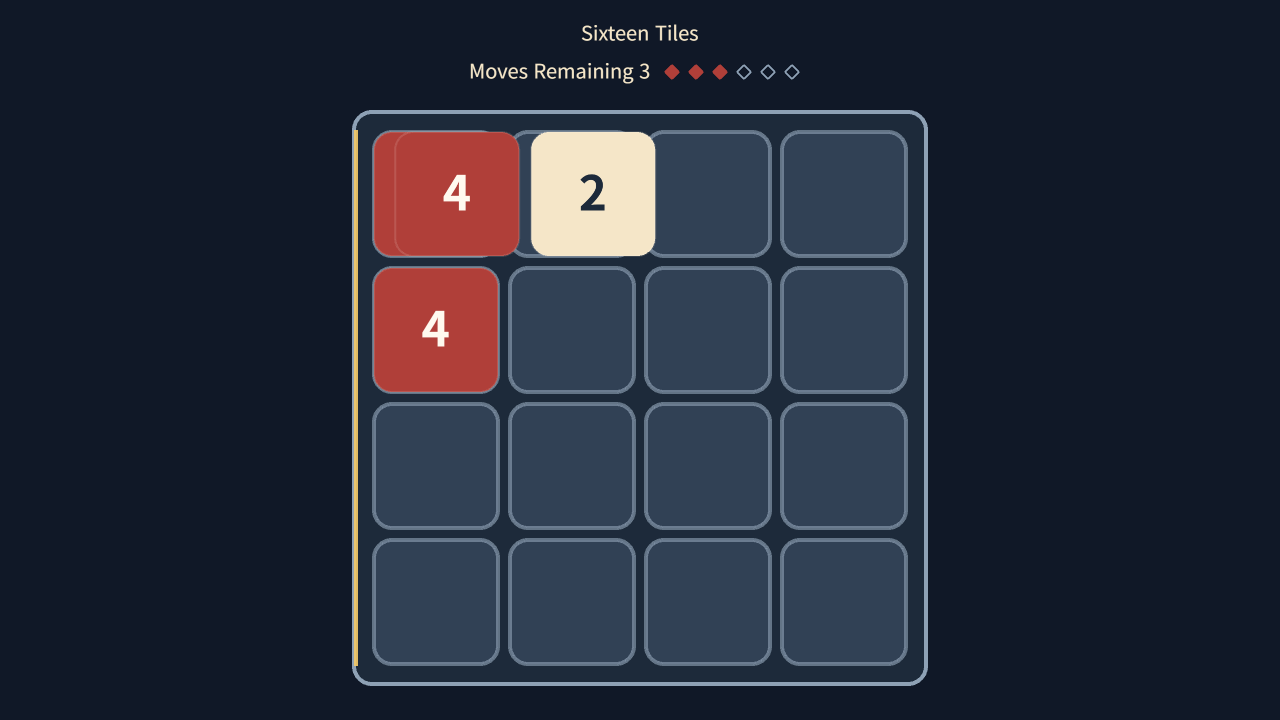}{Tiles Overlapping}}%
            {\AFSFrame[\AFSTileCrop]{756.4\,ms}{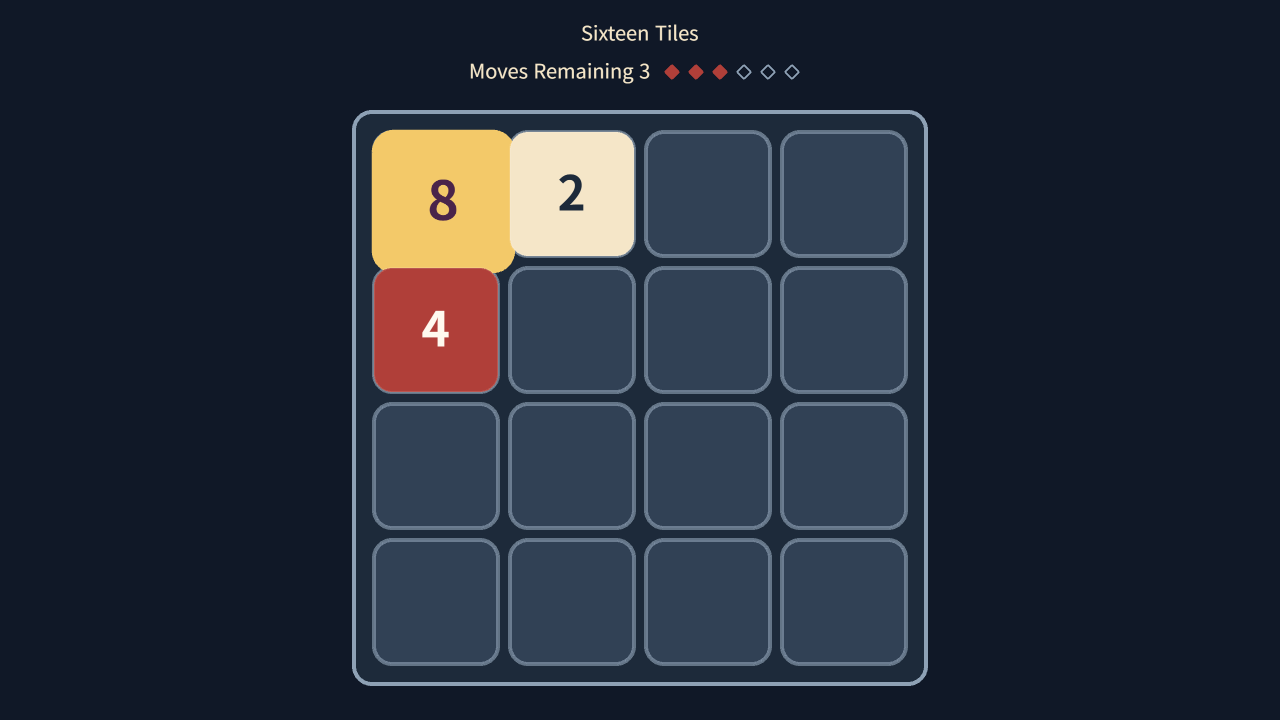}{Merged Tile}}%
    \end{subfigure}

    \caption{\textbf{Visual evidence from adaptive frame selection.}
    Each panel compares the same replay of a \emph{Small} game.
    Adaptive selection captures (a) Confirm activation, (b) the path before removal, (c) holding and defense feedback, and (d) tile convergence and overlap.
    These cues are absent from the displayed uniform samples.
    Each row shows three cropped frames with timestamps.}
    \label{fig:adaptive_frame_selection_qualitative}
\end{figure}
