# Supplementary material for: A2Z GameSpec-Bench: How Faithfully Can Coding Agents Generate Games from Game Design Specifications?
Source: arXiv:2609.39564 source file (2026-09-30)
Supplement: Supplementary file 7 [file playtest_interface.tex]

\begin{figure*}[t]
\centering
\definecolor{MacRed}{HTML}{FF5F56}
\definecolor{MacYellow}{HTML}{FFBD2E}
\definecolor{MacGreen}{HTML}{27C93F}
\definecolor{MacBar}{HTML}{313238}
\definecolor{MacBg}{HTML}{F6F8FA}
\definecolor{MacText}{HTML}{24292E}

\tcbset{
  macwindow/.style={
    enhanced,
    boxrule=0pt,
    colback=MacBg,
    coltext=MacText,
    arc=5pt,
    top=2pt, bottom=2pt, left=5pt, right=5pt,
    fonttitle=\ttfamily\bfseries\scriptsize\color{white},
    coltitle=white,
    colbacktitle=MacBar,
    titlerule=0pt,
    halign title=left,
    lefttitle=42pt,
    toptitle=2pt,
    bottomtitle=2pt,
    overlay={
      \fill[MacRed] (frame.north west) ++(14pt,-9pt) circle (2.8pt);
      \fill[MacYellow] (frame.north west) ++(25pt,-9pt) circle (2.8pt);
      \fill[MacGreen] (frame.north west) ++(36pt,-9pt) circle (2.8pt);
    }
  }
}

\begin{tcblisting}{
  macwindow,
  title={(a) The Shared \texttt{ctx} Interface},
  listing only,
  listing options={
    basicstyle=\ttfamily\scriptsize\color{MacText}\linespread{1.15}\selectfont,
    breaklines=true,
    breakatwhitespace=true,
    columns=fullflexible,
    keepspaces=true,
    showstringspaces=false,
    literate={-}{{\textcolor{gray!80!black}{-}}}{1}
  }
}
export const budgetMs: number;  export default async function run(ctx: Ctx);
interface Ctx {
  state(); live(fn); watch(fn); snapshot(label, extra?); note(msg);   // observation, read-only
  tap(key); press(keys); type(text); hold(key, ms?); down(key); up(key);   // keyboard
  click(x, y, button?); move(x, y); mouseDown(); mouseUp(); mouseHold(); drag(points); wheel(dx, dy);
  blur(); focus(); hide(); show(); pointerCancel();                    // window and document
  wait(ms); waitFrames(n); waitFor(predicate, opts?);                  // waiting
  setState(patch);                                          // adversarial only, refused in the normal playtest
}
export const scenario?: string;                             // declared scenario entry, adversarial only
\end{tcblisting}

\vspace{2pt}
\begin{tcblisting}{
  macwindow,
  title={(b) Normal Playtest Bot \hfill \normalfont\scriptsize\ttfamily magnet\_dock, excerpt},
  listing only,
  listing options={
    basicstyle=\ttfamily\scriptsize\color{MacText}\linespread{1.15}\selectfont,
    breaklines=true,
    breakatwhitespace=true,
    columns=fullflexible,
    keepspaces=true,
    showstringspaces=false,
    literate={-}{{\textcolor{gray!80!black}{-}}}{1}
  }
}
export default async function run(ctx) {
  const snap = (label, rules, kind, detail) =>
    ctx.snapshot(label, { targetRule: rules, trigger: { kind, detail } });
  ctx.watch(() => {                          // live-state fields attached to every snapshot
    const g = window.GameInspector?.exportState?.().game;
    return g && { state: g.state, polarity: g.polarity, settleTicks: g.settleTicks };
  });
  await ctx.snapshot('initial');
  await ctx.down('Space');  await ctx.waitFrames(2);   // one fresh toggle while held ...
  await snap('I5-first-polarity-toggle', ['I5'], 'input', 'fresh Space down');
  await ctx.down('Space');  await ctx.waitFrames(2);   // ... a second down must not toggle
  await snap('I3-held-space-repeat-inert', ['I3'], 'input', 'second down while held');
  await ctx.up('Space');
  if ((await ctx.state()).game.state === 'S_RESULT') {
    await ctx.click(640, 492);
    await snap('S13-result-to-title', ['S13'], 'input', 'clicked Title');
  }
}
\end{tcblisting}

\vspace{2pt}
\begin{tcblisting}{
  macwindow,
  title={(c) Adversarial Playtest Bot \hfill \normalfont\scriptsize\ttfamily magnet\_dock, rule D1, excerpt},
  listing only,
  listing options={
    basicstyle=\ttfamily\scriptsize\color{MacText}\linespread{1.15}\selectfont,
    breaklines=true,
    breakatwhitespace=true,
    columns=fullflexible,
    keepspaces=true,
    showstringspaces=false,
    literate={-}{{\textcolor{gray!80!black}{-}}}{1}
  }
}
export const scenario = 'dock_center_at_rest';       // declared scenario entry
export default async function run(ctx) {
  const gameState = async () => (await ctx.state())?.game ?? {};
  if ((await gameState()).settleTicks !== 59)        // pin the final pre-threshold tick
    await ctx.setState({ game: { state: 'S_PLAY', settleTicks: 59, x: 0, v: 0,
      polarity: 'Attract', positionQualified: true, speedQualified: true } });
  const before = await gameState();
  await ctx.snapshot('D1-before');
  let after = before;
  for (let i = 0; i < 8 && after.settleTicks < 60; i++) {
    await ctx.waitFrames(1);  after = await gameState();
  }
  await ctx.snapshot('D1-after', { targetRule: ['D1'], trigger: { kind: 'timer',
    detail: { prior: before.settleTicks, observed: after.settleTicks } } });
}
\end{tcblisting}

\vspace{-5pt}
\caption{\textbf{The playtest runtime interface and two recorded bots for \texttt{magnet\_dock}.} (a) Every bot receives the same \texttt{ctx}. (b) The normal playtest bot reads state, issues inputs, and records labelled snapshots naming the target rule. (c) The adversarial playtest bot enters through a declared scenario, pins the precondition of rule \texttt{D1} with \texttt{setState}, and observes the outcome.}
\label{fig:playtest_interface}
\end{figure*}
