# Supplementary material for: A2Z GameSpec-Bench: How Faithfully Can Coding Agents Generate Games from Game Design Specifications?
Source: arXiv:2609.39564 source file (2026-09-30)
Supplement: Supplementary file 8 [file fig_playtest_prompts.tex]

\begin{figure*}[!t]
\centering
\definecolor{MacRed}{HTML}{FF5F56}
\definecolor{MacYellow}{HTML}{FFBD2E}
\definecolor{MacGreen}{HTML}{27C93F}
\definecolor{MacBar}{HTML}{313238}
\definecolor{MacBg}{HTML}{F6F8FA}
\definecolor{MacText}{HTML}{24292E}

\tcbset{
  macwindow/.style={
    enhanced,
    boxrule=0pt,
    colback=MacBg,
    coltext=MacText,
    arc=5pt,
    top=8pt, bottom=8pt, left=10pt, right=10pt,
    fonttitle=\ttfamily\bfseries\scriptsize\color{white},
    coltitle=white,
    colbacktitle=MacBar,
    titlerule=0pt,
    halign title=left,
    lefttitle=42pt,
    toptitle=4pt,
    bottomtitle=4pt,
    overlay={
      \fill[MacRed] (frame.north west) ++(14pt,-9pt) circle (2.8pt);
      \fill[MacYellow] (frame.north west) ++(25pt,-9pt) circle (2.8pt);
      \fill[MacGreen] (frame.north west) ++(36pt,-9pt) circle (2.8pt);
    }
  }
}

\begin{tcblisting}{
  macwindow,
  title={Normal Playtest Author Prompt},
  listing only,
  listing options={
    basicstyle=\ttfamily\scriptsize\color{MacText}\linespread{1.15}\selectfont,
    breaklines=true,
    breakatwhitespace=true,
    columns=fullflexible,
    keepspaces=true,
    showstringspaces=false,
    literate={-}{{\textcolor{gray!80!black}{-}}}{1}
             {[...]}{{\textcolor{gray}{[...]}}}{5}
  }
}
[...]
- Use only normal player input after the initial page load.
- After every action aimed at one or more Rules, call `ctx.snapshot('<RuleId>[-<RuleId>...]-<what-happened>', { targetRule: ['<RuleId>', ...], trigger: { kind: 'input' | 'timer' | 'event', detail: '<what you did or waited for>' } })`. [...]
- A snapshot taken BEFORE the action (the situation, not the outcome) carries the suffix `-before` and no `targetRule`. [...]
[...]
\end{tcblisting}

\vspace{2pt}
\begin{tcblisting}{
  macwindow,
  title={Adversarial Author Prompt},
  listing only,
  listing options={
    basicstyle=\ttfamily\scriptsize\color{MacText}\linespread{1.15}\selectfont,
    breaklines=true,
    breakatwhitespace=true,
    columns=fullflexible,
    keepspaces=true,
    showstringspaces=false,
    literate={-}{{\textcolor{gray!80!black}{-}}}{1}
             {[...]}{{\textcolor{gray}{[...]}}}{5}
  }
}
[...]
- Use `ctx.setState` only when normal input cannot establish a root precondition.
- Record every assistance with `ctx.note('ASSISTED_RULE=<id>: <reason>')`.
Snapshot each attempted Rule before and after its trigger. If an expected transition does not occur, record the observed blocker and return normally; do not throw or assert.
[...]
\end{tcblisting}

\vspace{2pt}
\begin{tcblisting}{
  macwindow,
  title={Trace Judge Prompt},
  listing only,
  listing options={
    basicstyle=\ttfamily\scriptsize\color{MacText}\linespread{1.15}\selectfont,
    breaklines=true,
    breakatwhitespace=true,
    columns=fullflexible,
    keepspaces=true,
    showstringspaces=false,
    literate={-}{{\textcolor{gray!80!black}{-}}}{1}
             {[...]}{{\textcolor{gray}{[...]}}}{5}
  }
}
[...]
Verdict evidence must come from trace snapshots, trace events, or trace notes.
Absence of evidence is `unverified`, not `violated`. [...] A snapshot label is a navigation aid, not behavioral proof.
Submit exactly one entry for every requested Rule id in the supplied order.
[...]
\end{tcblisting}

\vspace{-5pt}
\caption{\textbf{Excerpts of the three adaptive-playtest system prompts.} Text is verbatim, and omitted passages are marked \texttt{[...]}.}
\label{fig:playtest-prompts}
\end{figure*}
