# Supplementary material for: A2Z GameSpec-Bench: How Faithfully Can Coding Agents Generate Games from Game Design Specifications?
Source: arXiv:2609.39564 source file (2026-09-30)
Supplement: Supplementary file 9 [file fig_replay_prompts.tex]

\begin{figure*}[t]
\centering
\definecolor{MacRed}{HTML}{FF5F56}
\definecolor{MacYellow}{HTML}{FFBD2E}
\definecolor{MacGreen}{HTML}{27C93F}
\definecolor{MacBar}{HTML}{313238}
\definecolor{MacBg}{HTML}{F6F8FA}
\definecolor{MacText}{HTML}{24292E}

\tcbset{
  macwindow/.style={
    enhanced,
    boxrule=0pt,
    colback=MacBg,
    coltext=MacText,
    arc=5pt,
    top=8pt, bottom=8pt, left=10pt, right=10pt,
    fonttitle=\ttfamily\bfseries\scriptsize\color{white},
    coltitle=white,
    colbacktitle=MacBar,
    titlerule=0pt,
    halign title=left,
    lefttitle=42pt,
    toptitle=4pt,
    bottomtitle=4pt,
    overlay={
      \fill[MacRed] (frame.north west) ++(14pt,-9pt) circle (2.8pt);
      \fill[MacYellow] (frame.north west) ++(25pt,-9pt) circle (2.8pt);
      \fill[MacGreen] (frame.north west) ++(36pt,-9pt) circle (2.8pt);
    }
  }
}

\begin{tcblisting}{
  macwindow,
  title={Frame-selection prompt (excerpt)},
  listing only,
  listing options={
    basicstyle=\ttfamily\scriptsize\color{MacText}\linespread{1.15}\selectfont,
    breaklines=true,
    breakatwhitespace=true,
    columns=fullflexible,
    keepspaces=true,
    showstringspaces=false,
    literate={-}{{\textcolor{gray!80!black}{-}}}{1}
             {[...]}{{\textcolor{gray}{[...]}}}{5}
  }
}
[...]
The executed input trace is a temporal index, not visual proof. The pre-trace and post-trace context frames are already included as deterministic replay boundaries. Map every rubric target to any additional replay intervals, first POST_RENDER points after inputs, or replay boundaries needed beyond that context. A frame may support several targets, and one target may use several locations.
After duplicate frames are removed, the complete plan must remain within the declared maximum observation count. Do not invent time offsets, game-specific event categories, visual outcomes, or composite images.
[...]
\end{tcblisting}

\vspace{2pt}
\begin{tcblisting}{
  macwindow,
  title={Scoring prompt (excerpt)},
  listing only,
  listing options={
    basicstyle=\ttfamily\scriptsize\color{MacText}\linespread{1.15}\selectfont,
    breaklines=true,
    breakatwhitespace=true,
    columns=fullflexible,
    keepspaces=true,
    showstringspaces=false,
    literate={-}{{\textcolor{gray!80!black}{-}}}{1}
             {[...]}{{\textcolor{gray}{[...]}}}{5}
  }
}
Only the individual original-resolution images in the user message are visual evidence. The frame metadata identifies their replay position and intended targets, but it is not proof by itself.
Score every original rubric requirement. Cite at least one observed frame ID for every score and explain only what the cited visual evidence supports. Do not treat the scenario text, expected outcome, trace metadata, or source code as proof that a rendered behavior occurred.
\end{tcblisting}

\vspace{-5pt}
\caption{\textbf{Excerpts of the two replay-judge system prompts.} Frame selection over the recorded replay and scoring from the selected frames. Text is verbatim, and omitted passages are marked \texttt{[...]}.}
\label{fig:replay-prompts}
\end{figure*}
