# Supplementary material for: A2Z GameSpec-Bench: How Faithfully Can Coding Agents Generate Games from Game Design Specifications?
Source: arXiv:2609.39564 source file (2026-09-30)
Supplement: Supplementary file 10 [file fig_source_prompt.tex]

\begin{figure*}[t]
\centering
\definecolor{MacRed}{HTML}{FF5F56}
\definecolor{MacYellow}{HTML}{FFBD2E}
\definecolor{MacGreen}{HTML}{27C93F}
\definecolor{MacBar}{HTML}{313238}
\definecolor{MacBg}{HTML}{F6F8FA}
\definecolor{MacText}{HTML}{24292E}

\tcbset{
  macwindow/.style={
    enhanced,
    boxrule=0pt, % 테두리 제거로 더 깔끔한 에디터 느낌 부여
    colback=MacBg,
    coltext=MacText,
    arc=5pt,
    top=8pt, bottom=8pt, left=10pt, right=10pt,
    fonttitle=\ttfamily\bfseries\scriptsize\color{white},
    coltitle=white,
    colbacktitle=MacBar,
    titlerule=0pt,
    halign title=left, % 사진처럼 제목을 좌측 정렬
    lefttitle=42pt, % 버튼 영역 확보
    toptitle=4pt, % 타이틀 바 높이 대폭 축소
    bottomtitle=4pt,
    overlay={
      % 얇아진 타이틀 바에 맞춰 버튼 위치 수직 중앙 재정렬 및 크기 조정
      \fill[MacRed] (frame.north west) ++(14pt,-9pt) circle (2.8pt);
      \fill[MacYellow] (frame.north west) ++(25pt,-9pt) circle (2.8pt);
      \fill[MacGreen] (frame.north west) ++(36pt,-9pt) circle (2.8pt);
    }
  }
}

\begin{tcblisting}{
  macwindow,
  title={Source-Code Judge Prompt},
  listing only,
  listing options={
    basicstyle=\ttfamily\scriptsize\color{MacText}\linespread{1.15}\selectfont,
    breaklines=true,
    breakatwhitespace=true,
    columns=fullflexible,
    keepspaces=true,
    showstringspaces=false,
    literate={-}{{\textcolor{gray!80!black}{-}}}{1}
             {[...]}{{\textcolor{gray}{[...]}}}{5}
  }
}
[...]
Static reading only: the question is "is this commitment implemented in the code", never "did it fire in some normal playtest" (that is a separate, trace-grounded measurement).
[...]
- fidelity is a real number 0.00-1.00 -- the degree to which the Rule as stated is implemented. Calibration anchors: 1.00 = fully as promised; 0.85 = minor deviation that does not change behavior in stated cases; 0.5 = about half the stated behavior (a condition unenforced, an effect missing); 0.2 = only traces; 0.00 = absent or contradicted. Use any intermediate value that best reflects the degree.
Judge the Rule as specified, not as you would have designed it. A reasonable alternative that does NOT do what the Rule states scores 0.
[...]
Judge a Rule EXISTENTIALLY -- does the stated mechanism exist with its stated gates and effects. Whether OTHER paths could interfere with or corrupt it (a stale callback, a re-entrant handler, an async edge that skips a re-check) is a universal property and belongs to the invariant checks, not here
[...]
- ok: true -- the code establishes the property and no reachable path violates it in scope.
- ok: false -- a code path can break it in scope, or nothing establishes it at all.
[...]
For every item, `evidence` cites what you actually read -- a file and the relevant function/line region, one sentence on how it implements (or fails) the item. "Probably implemented" without a location is not evidence; if you could not find it, the score is 0 and the evidence says what you searched.
[...]
\end{tcblisting}
\vspace{-5pt}
\caption{\textbf{Excerpt of the source-code judge system prompt.} Text is verbatim, and omitted passages are marked \texttt{[...]}.}
\label{fig:source-prompt}
\end{figure*}
