# Supplementary material for: A2Z GameSpec-Bench: How Faithfully Can Coding Agents Generate Games from Game Design Specifications?
Source: arXiv:2609.39564 source file (2026-09-30)
Supplement: Supplementary file 11 [file big_gameplay_01.tex]

\begin{figure}[p]
    \centering
    \begin{minipage}[t][\textheight][s]{\linewidth}
    \vspace{0pt}
    \captionsetup{font=small,skip=7pt}
    \renewcommand{\thesubfigure}{(\alph{subfigure})}
    \captionsetup[subfigure]{font={small,rm,bf},labelformat=simple,labelsep=space,justification=raggedright,singlelinecheck=false,position=top,skip=5pt,hypcap=true}

    % Crop margins: LEFT BOTTOM RIGHT TOP, applied before resizing.
    % The original JPGs are 960 x 540 at 72 dpi: 1 bp = 1 source pixel.
    % Zero margins retain the complete game screen and HUD.
    \newcommand{\BGQCloudCrop}{0bp 0bp 0bp 0bp}
    \newcommand{\BGQAfterglowCrop}{0bp 0bp 0bp 0bp}
    \newcommand{\BGQSiegeCrop}{0bp 0bp 0bp 0bp}
    \newcommand{\BGQLogisticsCrop}{0bp 0bp 0bp 0bp}
    \newcommand{\BGQFrameWidth}{0.322\linewidth}
    \newcommand{\BGQPanelGap}{13pt}
    \newcommand{\BGQLabelFont}{\rmfamily\color{A2ZFigText}\fontsize{8}{9.2}\selectfont}
    \newcommand{\BGQDetailFont}{\rmfamily\color{A2ZFigText}\fontsize{7.5}{8.5}\selectfont}

    % Arguments: [crop], original JPG path, mechanic label, visible detail.
    \newcommand{\BGQFrame}[4][0bp 0bp 0bp 0bp]{%
        \begin{minipage}[t]{\BGQFrameWidth}
            \centering
            \edef\BGQImageOptions{trim=#1,clip,width=\the\linewidth}
            \expandafter\includegraphics\expandafter[\BGQImageOptions]{#2}\par
            \vspace{3pt}
            {\BGQLabelFont\textbf{#3}\par}
            \vspace{1pt}
            {\BGQDetailFont #4\par}
        \end{minipage}%
    }

    % An unbreakable row keeps all three image columns together.
    \newcommand{\BGQRow}[3]{%
        \noindent\hbox to\linewidth{#1\hfil#2\hfil#3}\par
    }
    \newcommand{\BGQNote}[1]{%
        \vspace{5pt}
        {\rmfamily\color{A2ZFigText}\fontsize{8.5}{10}\selectfont\raggedright #1\par}
    }

    \begin{subfigure}[t]{\linewidth}
        \caption{\texttt{Cloud Cast}: Gearing, Reeling, and Catch Rewards}
        \label{fig:bgq_cloud_cast}
        \BGQRow%
            {\BGQFrame[\BGQCloudCrop]{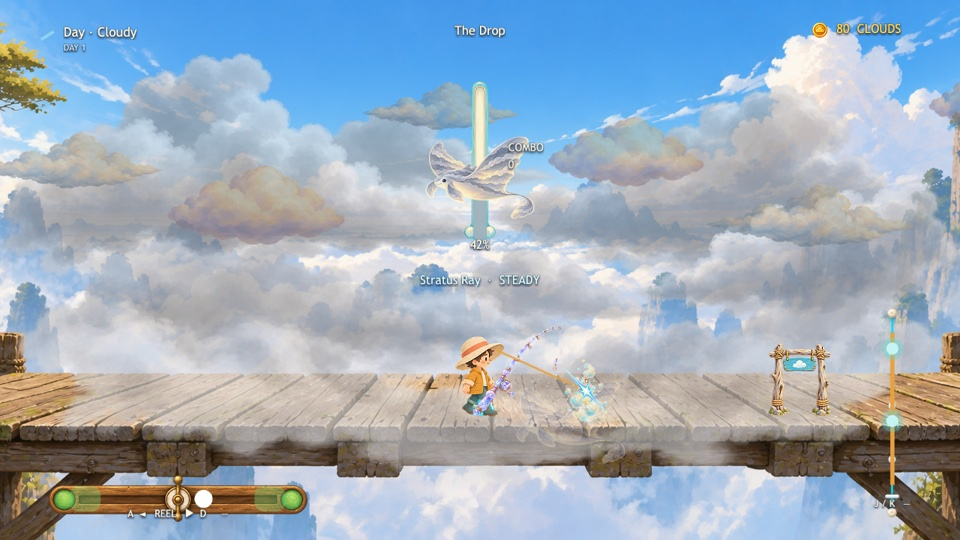}{Geared Max}{Hold and release Space}}%
            {\BGQFrame[\BGQCloudCrop]{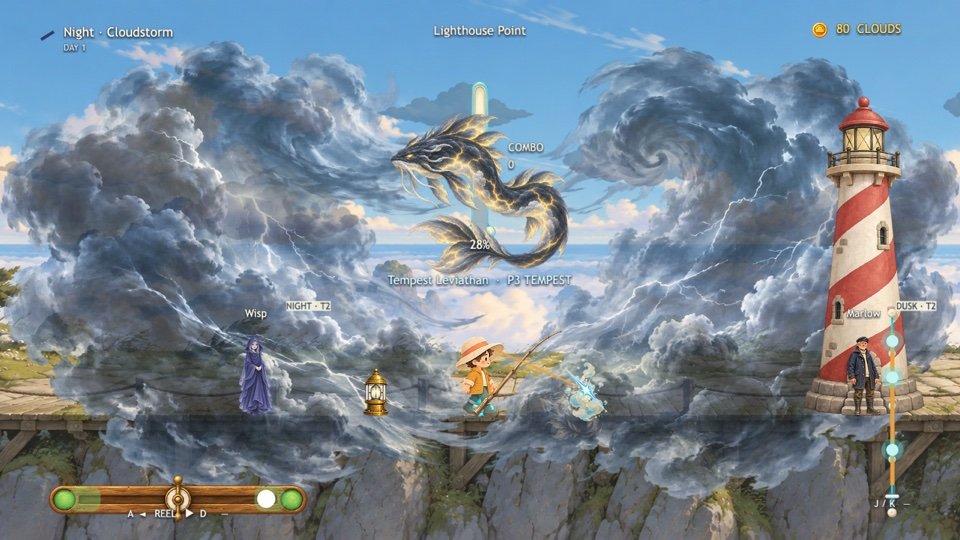}{Reel In}{Catch progress and timing}}%
            {\BGQFrame[\BGQCloudCrop]{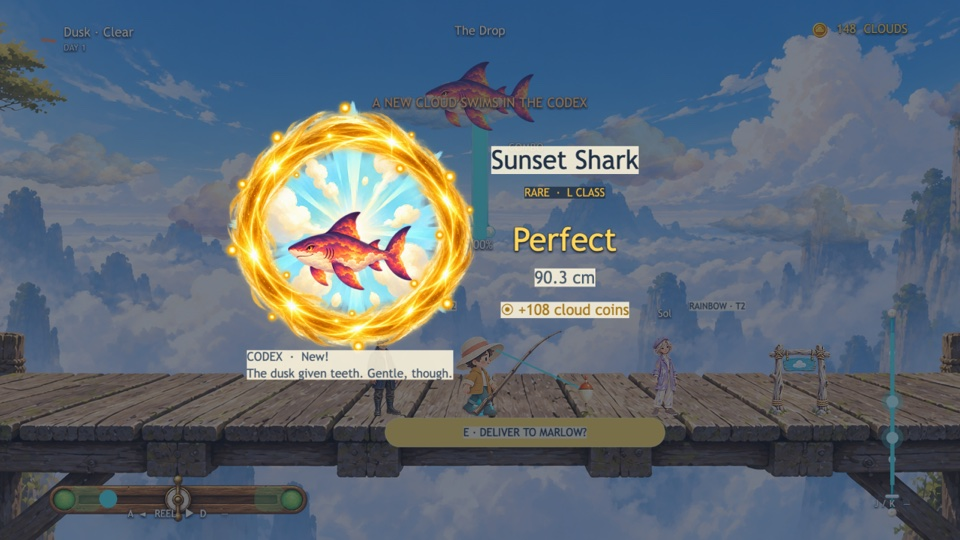}{Catch Reward}{Grade, size, and coins}}%
        \BGQNote{Casting prompts, reel controls, and timing cues support fishing. The catch screen reports the fish, its grade and size, and the coin reward.}
    \end{subfigure}

    \par\vfill

    \begin{subfigure}[t]{\linewidth}
        \caption{\texttt{Afterglow Network}: Traversal and Base Defense}
        \label{fig:bgq_afterglow_network}
        \BGQRow%
            {\BGQFrame[\BGQAfterglowCrop]{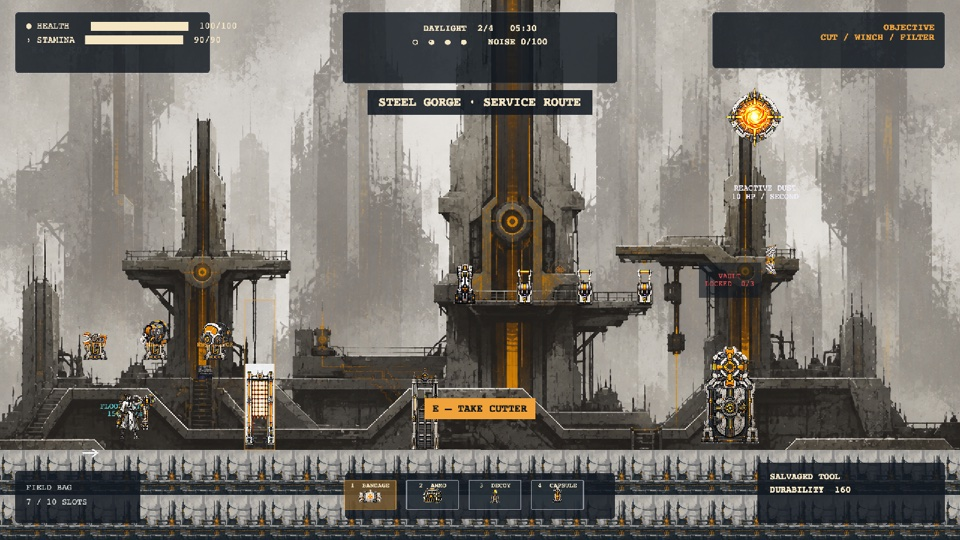}{Traversal Tools}{Cutter pickup prompt}}%
            {\BGQFrame[\BGQAfterglowCrop]{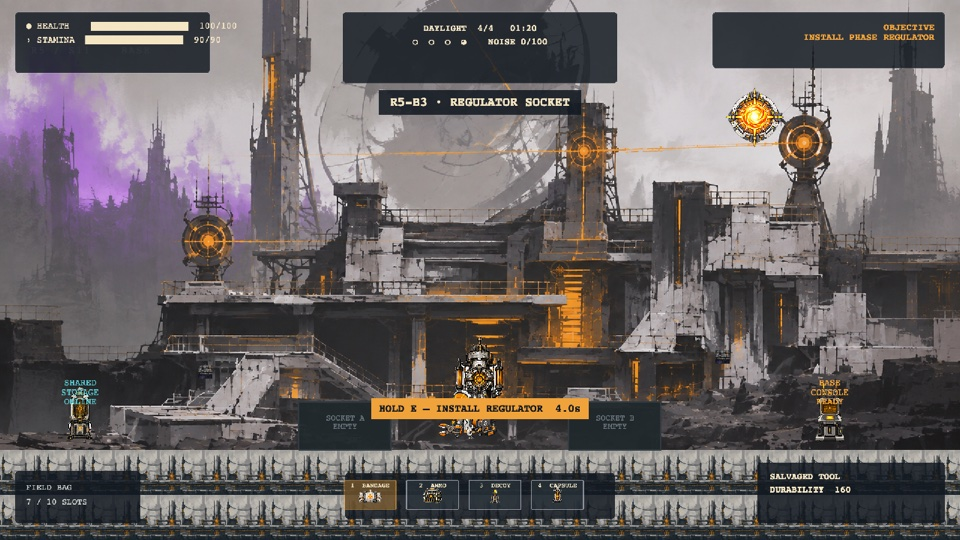}{Install a Regulator}{Timed interaction prompt}}%
            {\BGQFrame[\BGQAfterglowCrop]{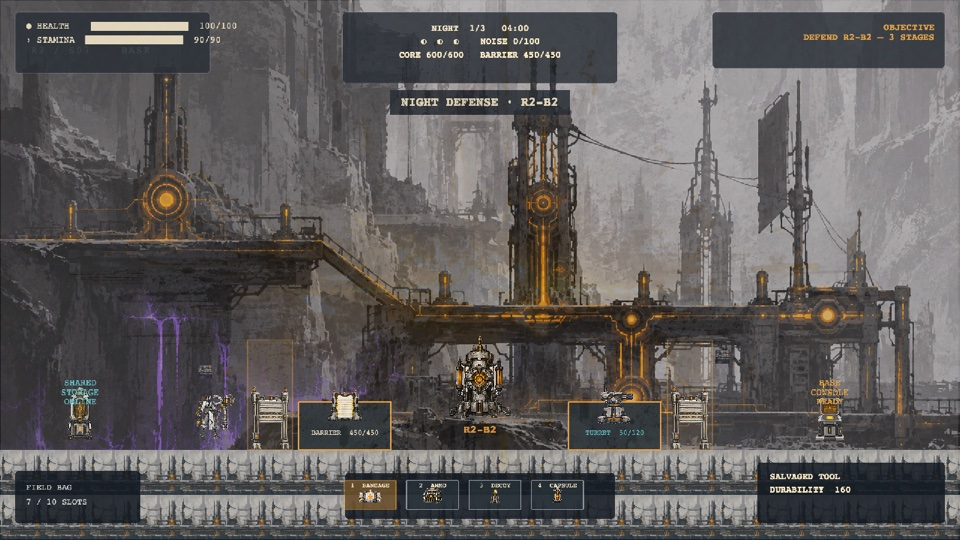}{Night Defense}{Barrier and turret status}}%
        \BGQNote{The selected states show tool pickup, a timed regulator installation prompt, and a defense site with separate core, barrier, and turret status.}
    \end{subfigure}

    \par\vfill

    \begin{subfigure}[t]{\linewidth}
        \caption{\texttt{Siege Deck 2D}: Deployment and Tactical Cards}
        \label{fig:bgq_siege_deck_2d}
        \BGQRow%
            {\BGQFrame[\BGQSiegeCrop]{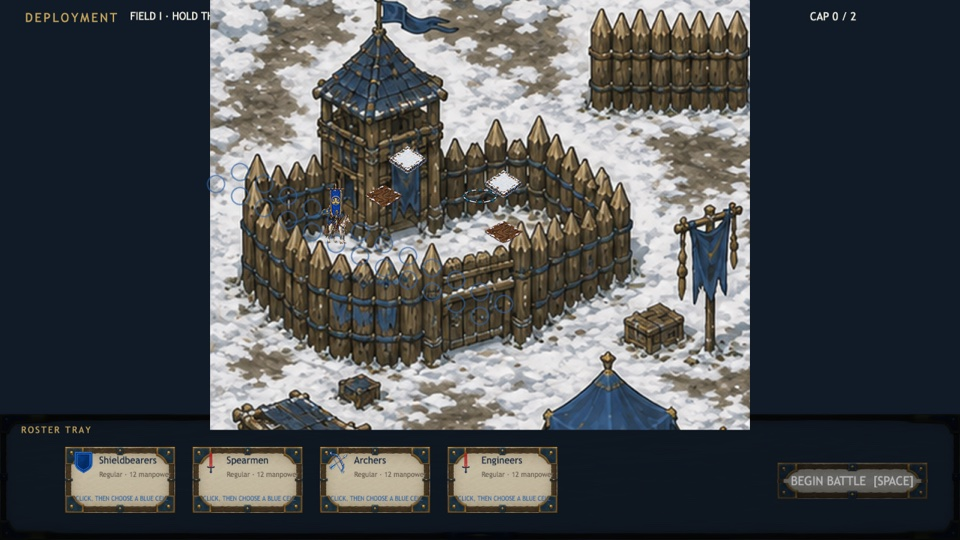}{Deploy Units}{Roster and placement cells}}%
            {\BGQFrame[\BGQSiegeCrop]{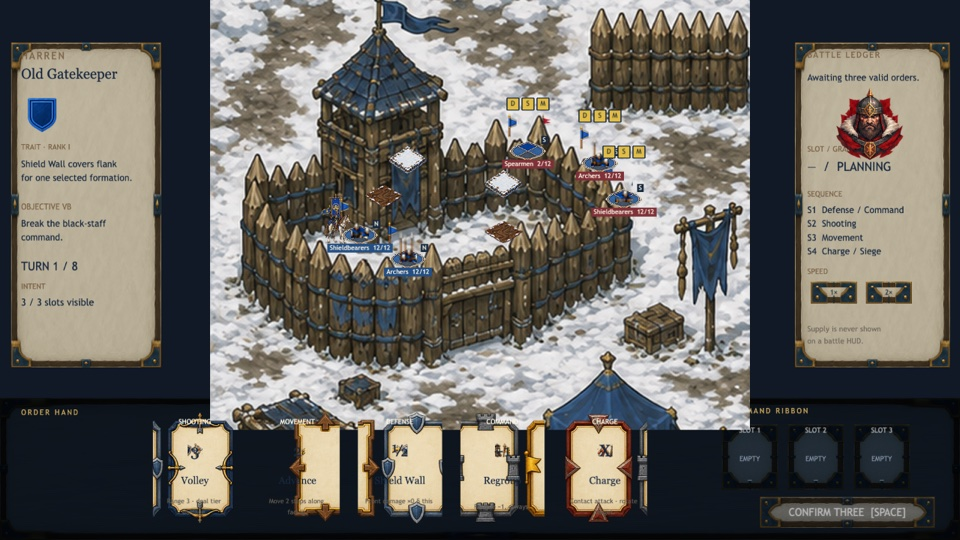}{Plan Orders}{Three order slots}}%
            {\BGQFrame[\BGQSiegeCrop]{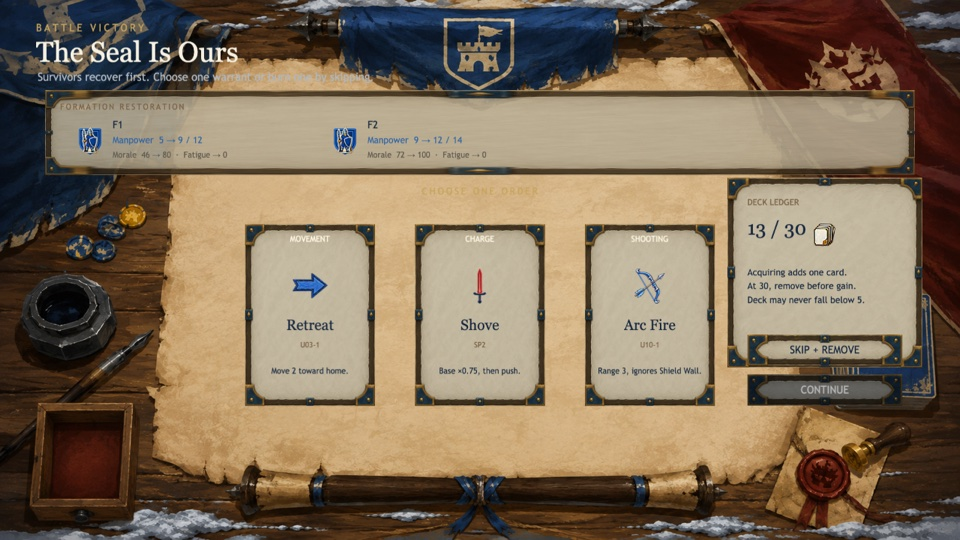}{Choose a Reward}{Cards and deck changes}}%
        \BGQNote{Deployment cells guide unit placement, and an order hand supports tactical planning. The victory screen offers new cards and deck modification options.}
    \end{subfigure}

    \par\vfill

    \begin{subfigure}[t]{\linewidth}
        \caption{\texttt{Wham Bam Logistics}: Route and Fleet Management}
        \label{fig:bgq_wham_bam_logistics}
        \BGQRow%
            {\BGQFrame[\BGQLogisticsCrop]{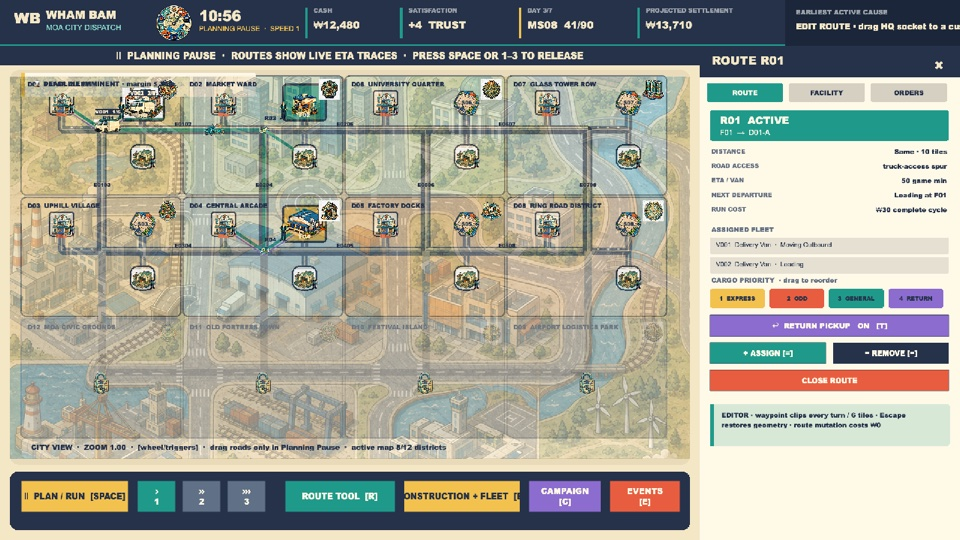}{Edit Routes}{Waypoints and cargo priorities}}%
            {\BGQFrame[\BGQLogisticsCrop]{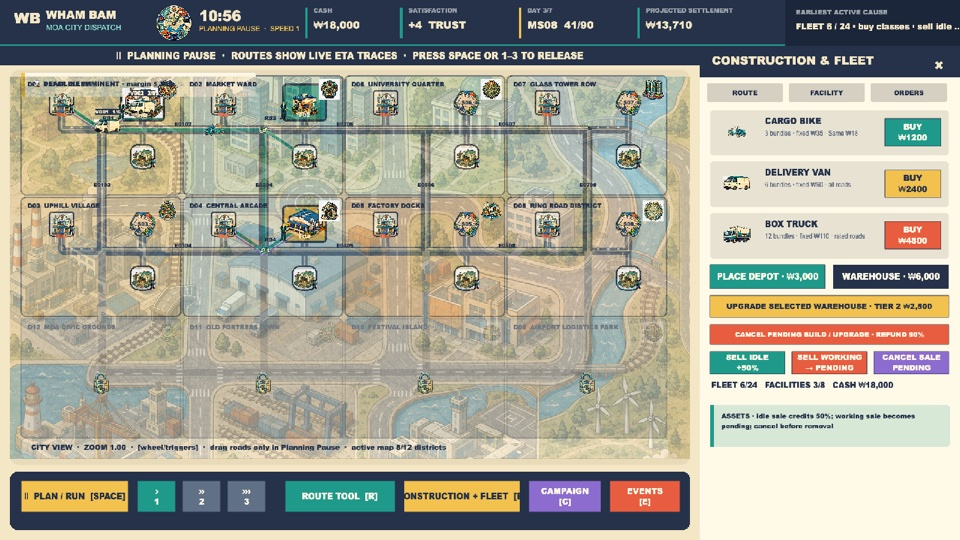}{Manage the Fleet}{Vehicles and facilities}}%
            {\BGQFrame[\BGQLogisticsCrop]{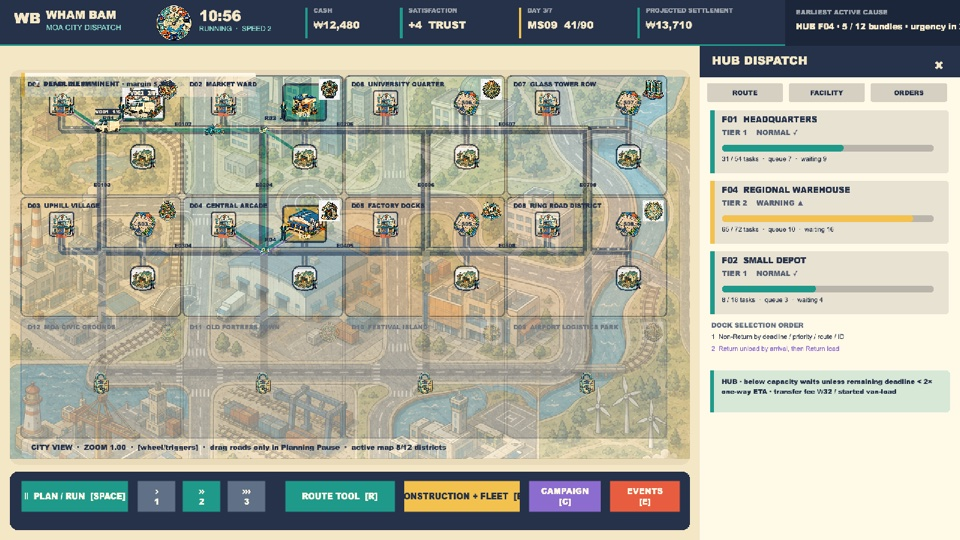}{Monitor Hub Loads}{Queues and capacity status}}%
        \BGQNote{A shared city map connects route editing, vehicle and facility purchases, and hub dispatch. Dedicated panels expose cargo priorities and facility loads.}
    \end{subfigure}

    \par\vfill
    \caption{\textbf{Sampled gameplays in generated \emph{Big} games (1).}
    Four games illustrate (a) fishing controls and catch rewards, (b) traversal tools and base defense, (c) unit deployment and tactical cards, and (d) delivery route and fleet management.
    Each row groups three scenario-specific screenshots from one game.
    Full screenshots retain the gameplay context and interface feedback.}
    \label{fig:big_gameplay_01}
    \end{minipage}
\end{figure}
