# Supplementary material for: A2Z GameSpec-Bench: How Faithfully Can Coding Agents Generate Games from Game Design Specifications?
Source: arXiv:2609.39564 source file (2026-09-30)
Supplement: Supplementary file 12 [file big_gameplay_02.tex]

% Required preamble packages: graphicx, subcaption.
% Place this file in the manuscript root, then use:
% \input{big_gameplay_mechanics_extra}
% Four additional Big games, exactly three original screenshots per row.
% The selected screenshots depict distinct scenario states within each game.
% All captions, labels, crop margins, dimensions, and spacing are editable here.

\begin{figure}[p] 
    \centering
    \begin{minipage}[t][\textheight][s]{\linewidth}
    \vspace{0pt}
    \captionsetup{font=small,skip=7pt}
    \renewcommand{\thesubfigure}{(\alph{subfigure})}
    \captionsetup[subfigure]{font={small,rm,bf},labelformat=simple,labelsep=space,justification=raggedright,singlelinecheck=false,position=top,skip=5pt,hypcap=true}

    % Crop margins: LEFT BOTTOM RIGHT TOP, applied before resizing.
    % Originals: 960 x 540. JPGs use 72 dpi; the PNG uses the 72 dpi default.
    % Thus, 1 bp corresponds to one source pixel. Zero crops retain full screens.
    \newcommand{\BGEChromaCrop}{0bp 0bp 0bp 0bp}
    \newcommand{\BGESsitgimCrop}{0bp 0bp 0bp 0bp}
    \newcommand{\BGEAlchemyCrop}{0bp 0bp 0bp 0bp}
    \newcommand{\BGEStrataCrop}{0bp 0bp 0bp 0bp}
    \newcommand{\BGEFrameWidth}{0.322\linewidth}
    \newcommand{\BGEPanelGap}{13pt}
    \newcommand{\BGELabelFont}{\rmfamily\color{A2ZFigText}\fontsize{8}{9.2}\selectfont}
    \newcommand{\BGEDetailFont}{\rmfamily\color{A2ZFigText}\fontsize{7.5}{8.5}\selectfont}

    % Arguments: [crop], original image path, mechanic label, visible detail.
    \newcommand{\BGEFrame}[4][0bp 0bp 0bp 0bp]{%
        \begin{minipage}[t]{\BGEFrameWidth}
            \centering
            \edef\BGEImageOptions{trim=#1,clip,width=\the\linewidth}
            \expandafter\includegraphics\expandafter[\BGEImageOptions]{#2}\par
            \vspace{3pt}
            {\BGELabelFont\textbf{#3}\par}
            \vspace{1pt}
            {\BGEDetailFont #4\par}
        \end{minipage}%
    }

    % An unbreakable row keeps exactly three image columns together.
    \newcommand{\BGERow}[3]{%
        \noindent\hbox to\linewidth{#1\hfil#2\hfil#3}\par
    }
    \newcommand{\BGENote}[1]{%
        \vspace{5pt}
        {\rmfamily\color{A2ZFigText}\fontsize{8.5}{10}\selectfont\raggedright #1\par}
    }

    \begin{subfigure}[t]{\linewidth}
        \caption{\texttt{ChromaShade}: Light and Shadow Traversal}
        \label{fig:bge_chromashade}
        \BGERow%
            {\BGEFrame[\BGEChromaCrop]{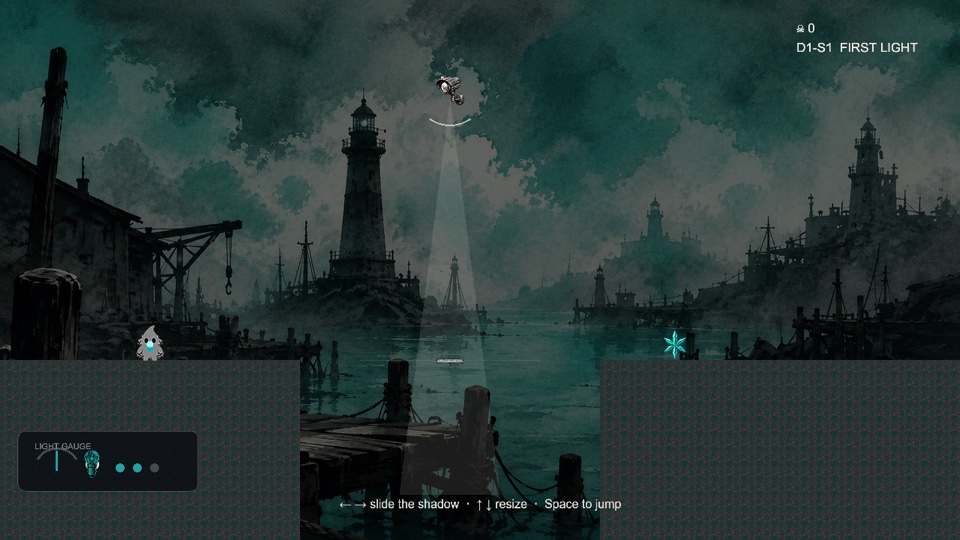}{Shape the Shadow}{Slide and resize controls}}%
            {\BGEFrame[\BGEChromaCrop]{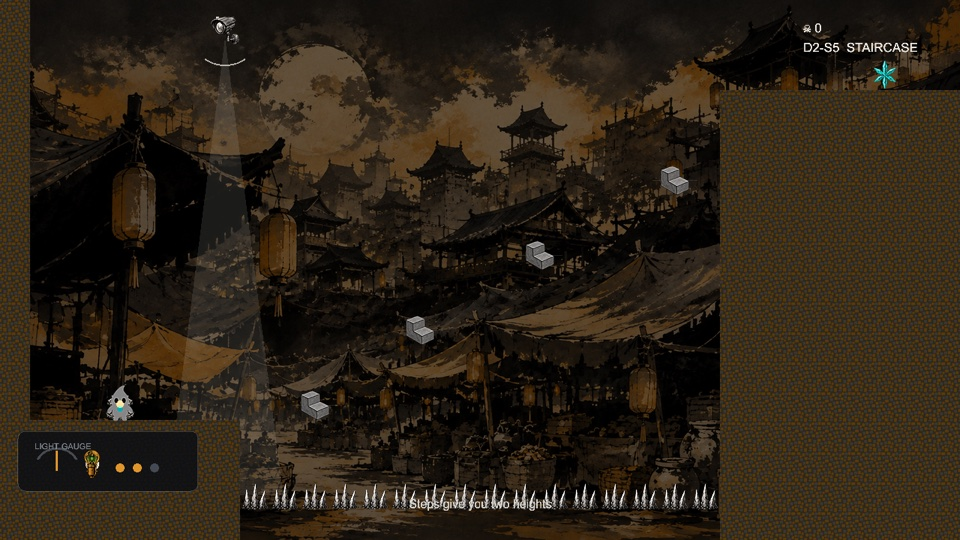}{Climb the Steps}{Platforms above floor spikes}}%
            {\BGEFrame[\BGEChromaCrop]{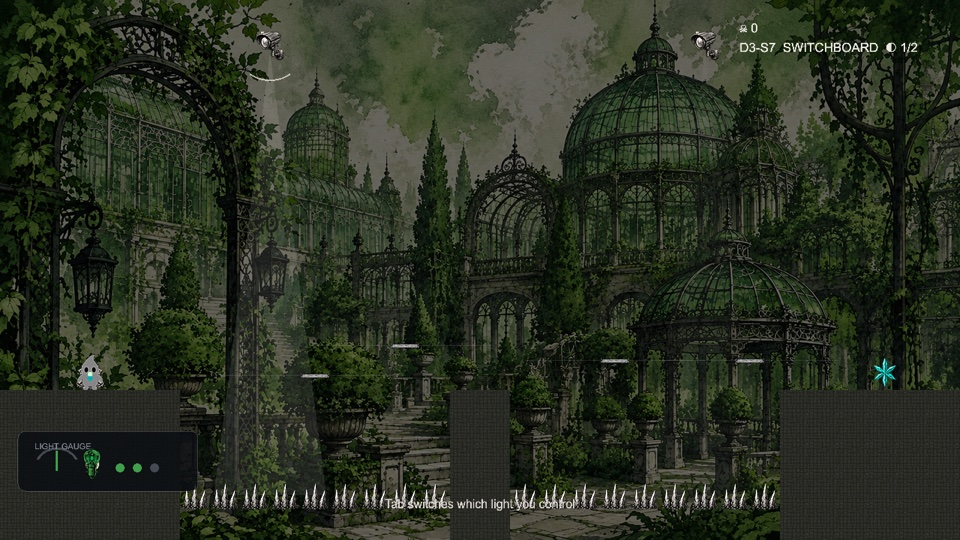}{Switch Lights}{Two controllable light sources}}%
        \BGENote{Movement puzzles combine shadow controls with platform traversal. Selected stages show stepped obstacles and the option to switch between light sources.}
    \end{subfigure}

    \par\vfill

    \begin{subfigure}[t]{\linewidth}
        \caption{\texttt{Ssitgim}: Soul Encounters and Cleansing}
        \label{fig:bge_ssitgim}
        \BGERow%
            {\BGEFrame[\BGESsitgimCrop]{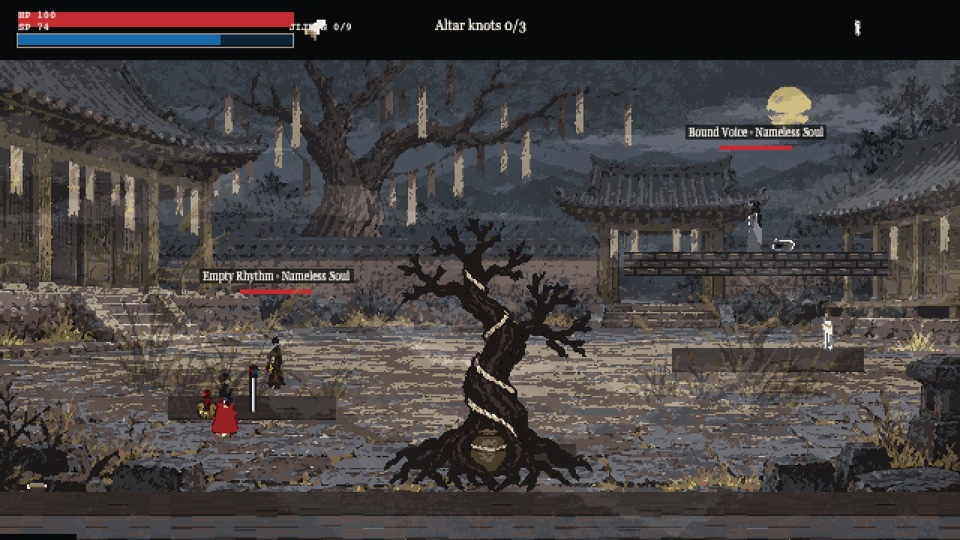}{Encounter Souls}{Two named soul types}}%
            {\BGEFrame[\BGESsitgimCrop]{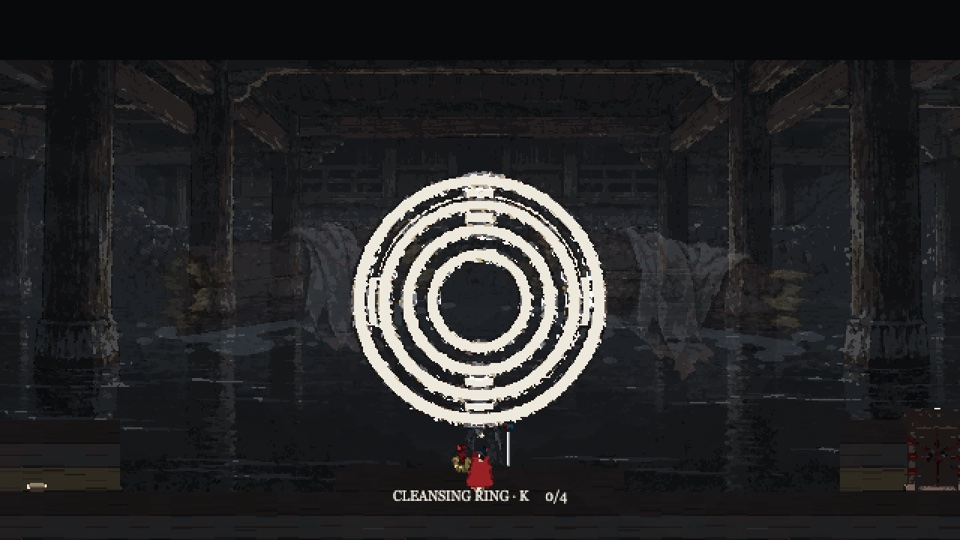}{Perform a Cleansing Rite}{Ring prompt and progress}}%
            {\BGEFrame[\BGESsitgimCrop]{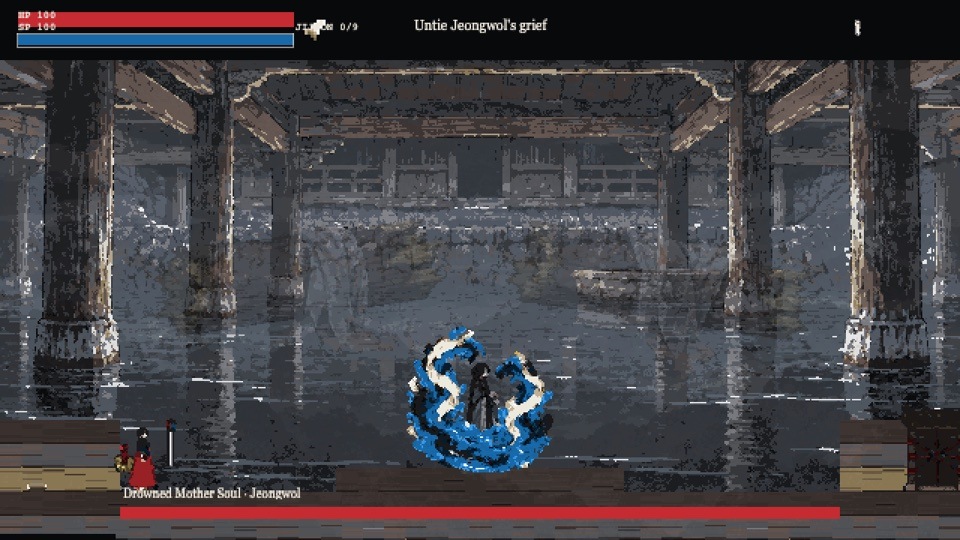}{Confront a Boss}{Boss identity and health bar}}%
        \BGENote{Soul encounters, a ring-based cleansing interface, and a boss encounter present distinct interactions within the same shrine setting.}
    \end{subfigure}

    \par\vfill

    \begin{subfigure}[t]{\linewidth}
        \caption{\texttt{Alias Alchemy Shop}: Production and Persistent Progress}
        \label{fig:bge_alias_alchemy_shop}
        \BGERow%
            {\BGEFrame[\BGEAlchemyCrop]{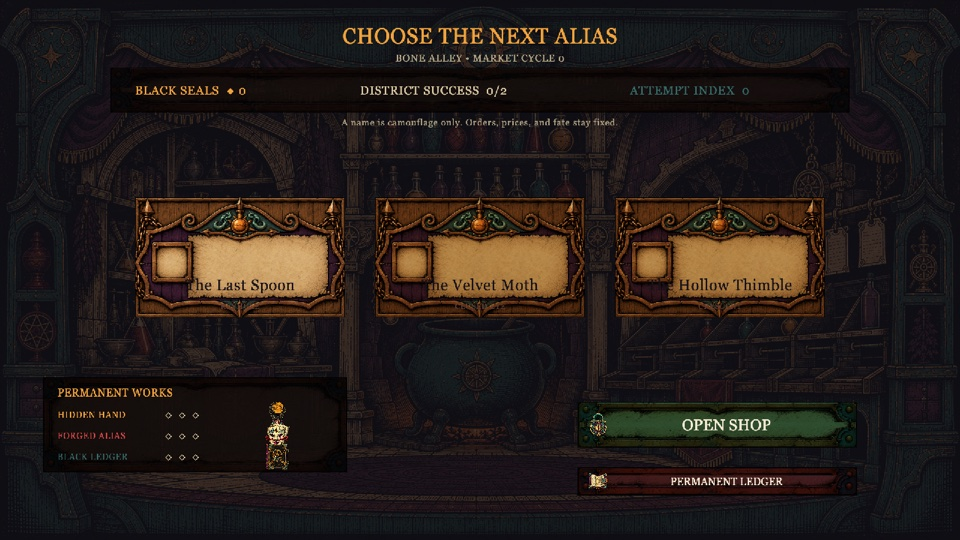}{Choose an Alias}{Shop identity and upgrades}}%
            {\BGEFrame[\BGEAlchemyCrop]{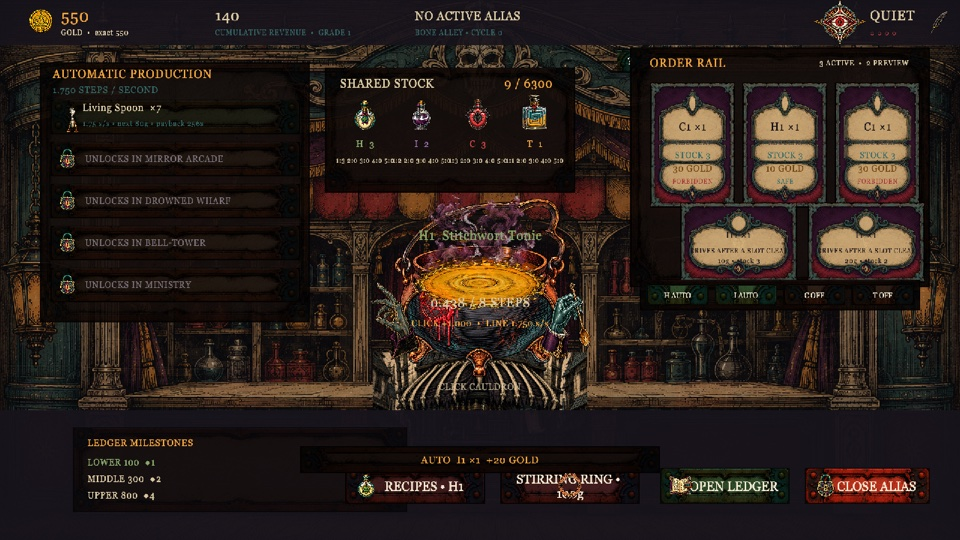}{Manage Production}{Shared stock and order cards}}%
            {\BGEFrame[\BGEAlchemyCrop]{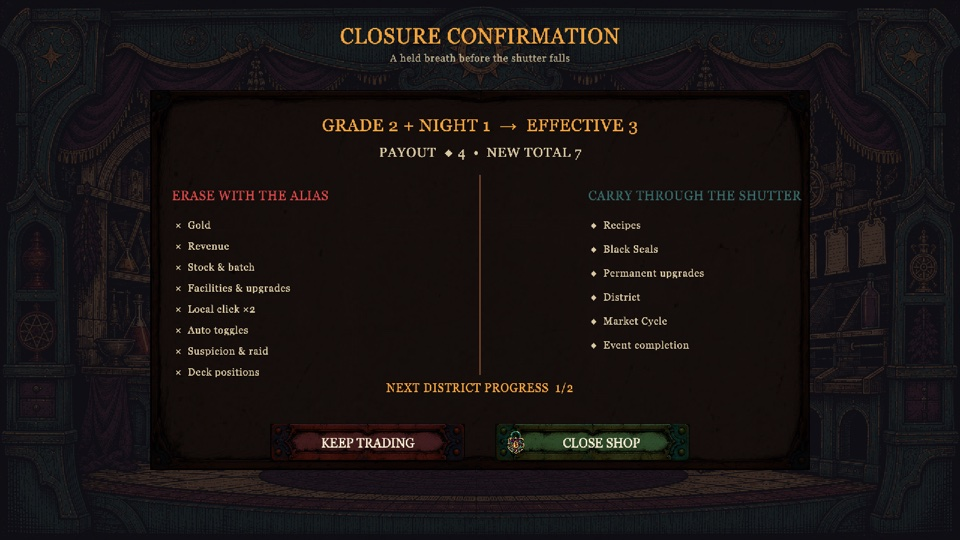}{Review Shop Closure}{Reset and persistent resources}}%
        \BGENote{The shop combines production, shared inventory, and customer orders. Its closure screen lists resources that reset and progress that carries forward.}
    \end{subfigure}

    \par\vfill

    \begin{subfigure}[t]{\linewidth}
        \caption{\texttt{Strata Keepers}: Excavation, Restoration, and Research}
        \label{fig:bge_strata_keepers}
        \BGERow%
            {\BGEFrame[\BGEStrataCrop]{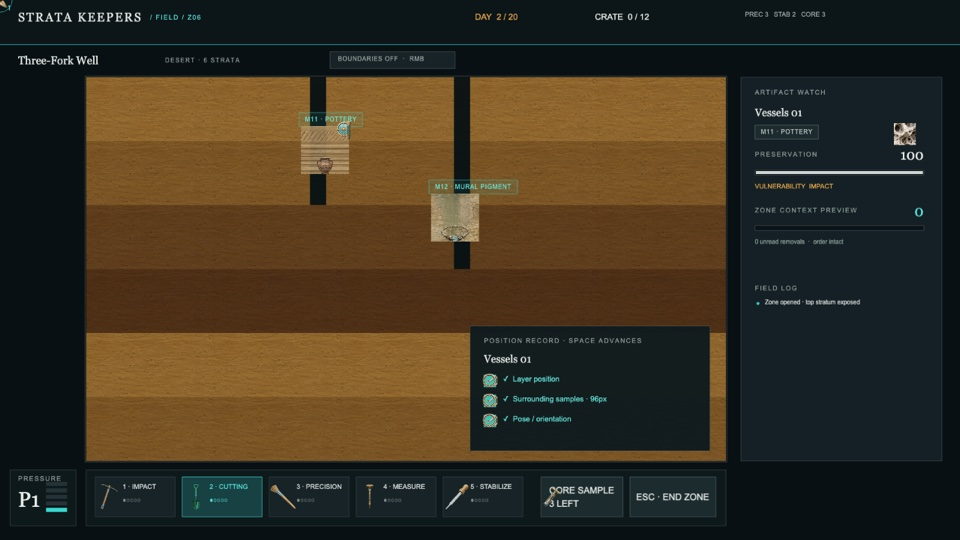}{Record a Find}{Layer, samples, and orientation}}%
            {\BGEFrame[\BGEStrataCrop]{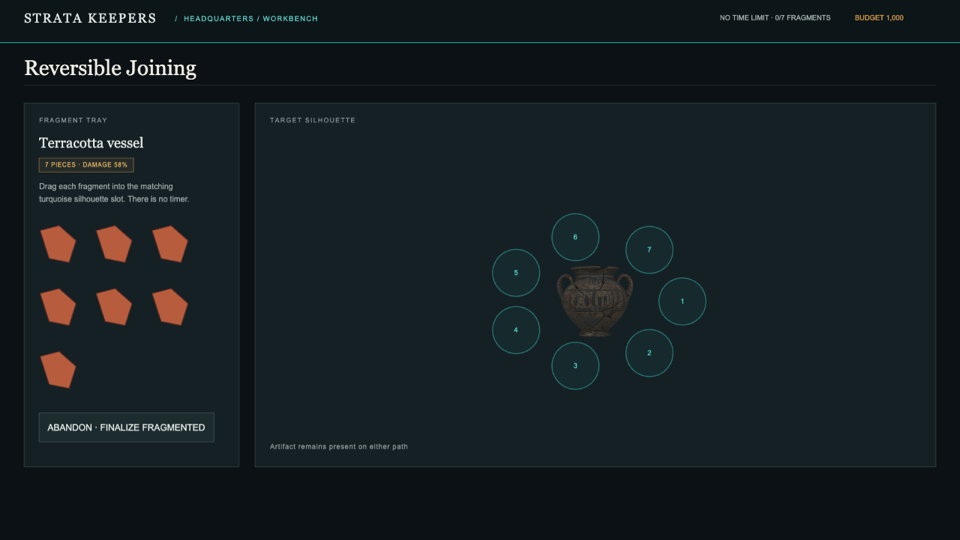}{Rejoin Fragments}{Drag pieces into target slots}}%
            {\BGEFrame[\BGEStrataCrop]{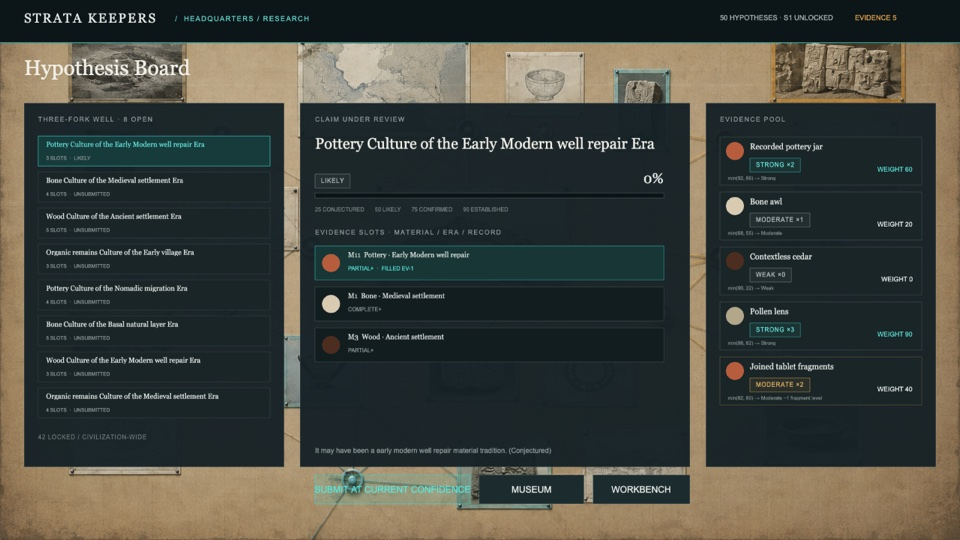}{Build a Hypothesis}{Evidence slots and confidence}}%
        \BGENote{Artifact records preserve excavation context. A joining puzzle and an evidence board provide separate interfaces for restoration and research.}
    \end{subfigure}

    \par\vfill
    \caption{\textbf{Sampled gameplays in generated \emph{Big} games (2).}
    Four games illustrate (a) light and shadow traversal, (b) soul encounters and cleansing, (c) production and persistent shop progress, and (d) excavation, restoration, and research.
    Each row groups three scenario-specific screenshots from one game.
    Full screenshots retain the gameplay context, controls, and state information.}
    \label{fig:big_gameplay_02}
    \end{minipage}
\end{figure}
