# Supplementary material for: A2Z GameSpec-Bench: How Faithfully Can Coding Agents Generate Games from Game Design Specifications?
Source: arXiv:2609.39564 source file (2026-09-30)
Supplement: Supplementary file 13 [file small_gameplay_01.tex]

\begin{figure}[p]
    \centering
    % Occupy the full text area, including the figure caption.
    % Stretch only inter-panel whitespace; preserve screenshot aspect ratios.
    \begin{minipage}[t][\textheight][s]{\linewidth}
    \vspace{0pt}
    \captionsetup{font=small,skip=7pt}
    \renewcommand{\thesubfigure}{(\alph{subfigure})}
    \captionsetup[subfigure]{font={small,rm,bf},labelformat=simple,labelsep=space,justification=raggedright,singlelinecheck=false,position=top,skip=5pt,hypcap=true}

    % Crop margins: LEFT BOTTOM RIGHT TOP.
    % All originals are 960 x 540 PNGs with no DPI metadata.
    % 0bp on all sides preserves the complete game screen and HUD.
    \newcommand{\GQMBloomCrop}{0bp 0bp 0bp 0bp}
    \newcommand{\GQMOddCrop}{0bp 0bp 0bp 0bp}
    \newcommand{\GQMOrbitCrop}{0bp 0bp 0bp 0bp}
    \newcommand{\GQMEchoCrop}{0bp 0bp 0bp 0bp}
    \newcommand{\GQMFrameWidth}{0.322\linewidth}
    \newcommand{\GQMLabelFont}{\rmfamily\color{A2ZFigText}\fontsize{8}{9.2}\selectfont}
    \newcommand{\GQMDetailFont}{\rmfamily\color{A2ZFigText}\fontsize{7.5}{8.5}\selectfont}

    % Arguments: [crop], PNG path, mechanic label, visible state detail.
    \newcommand{\GQMFrame}[4][0bp 0bp 0bp 0bp]{%
        \begin{minipage}[t]{\GQMFrameWidth}
            \centering
            \edef\GQMImageOptions{trim=#1,clip,width=\the\linewidth}
            \expandafter\includegraphics\expandafter[\GQMImageOptions]{#2}\par
            \vspace{3pt}
            {\GQMLabelFont\textbf{#3}\par}
            \vspace{1pt}
            {\GQMDetailFont #4\par}
        \end{minipage}%
    }

    % Exactly three images in one unbreakable horizontal row.
    \newcommand{\GQMRow}[3]{%
        \noindent\hbox to\linewidth{#1\hfil#2\hfil#3}\par
    }
    \newcommand{\GQMNote}[1]{%
        \vspace{5pt}
        {\rmfamily\color{A2ZFigText}\fontsize{8.5}{10}\selectfont\raggedright #1\par}
    }

    \begin{subfigure}[t]{\linewidth}
        \caption{\texttt{Bloom or Weed}: Selective Clicking}
        \label{fig:gqm_bloom_or_weed}
        \GQMRow%
            {\GQMFrame[\GQMBloomCrop]{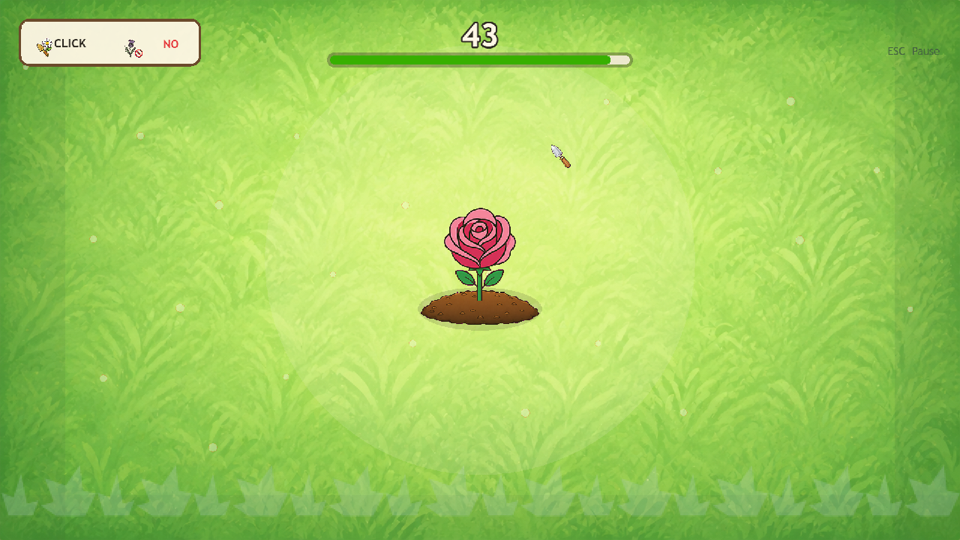}{Click the Bloom}{Rose prompt}}%
            {\GQMFrame[\GQMBloomCrop]{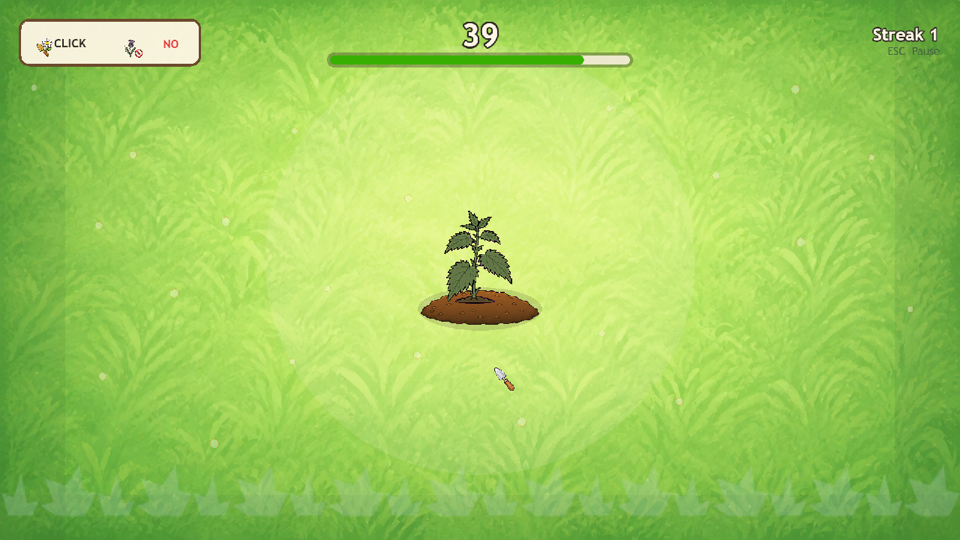}{Ignore the Weed}{Withhold input}}%
            {\GQMFrame[\GQMBloomCrop]{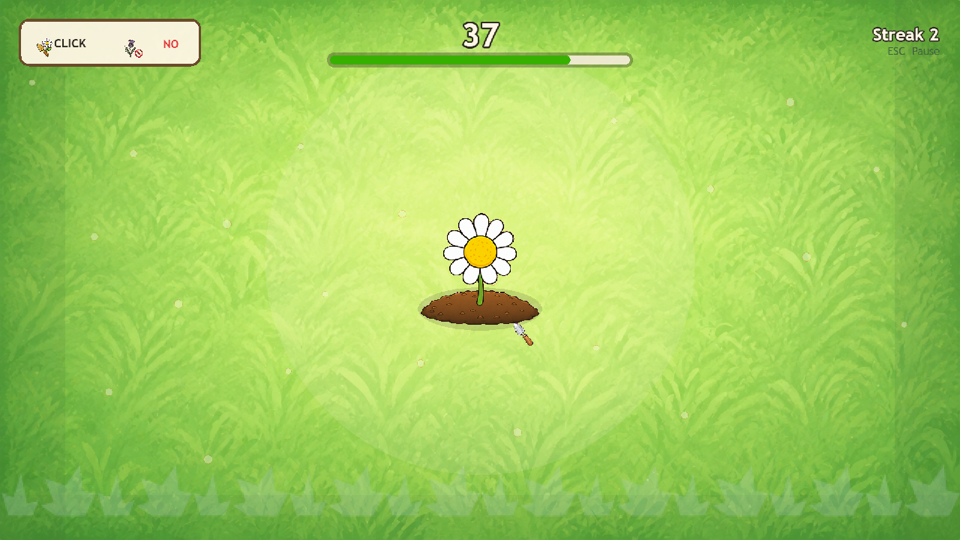}{Click the Bloom}{Daisy prompt}}%
        \GQMNote{Bloom and weed prompts require different responses: click the flowers and withhold input for the weeds.}
    \end{subfigure}

    \par\vfill

    \begin{subfigure}[t]{\linewidth}
        \caption{\texttt{Odd Patch}: Color and Shape Discrimination}
        \label{fig:gqm_odd_patch}
        \GQMRow%
            {\GQMFrame[\GQMOddCrop]{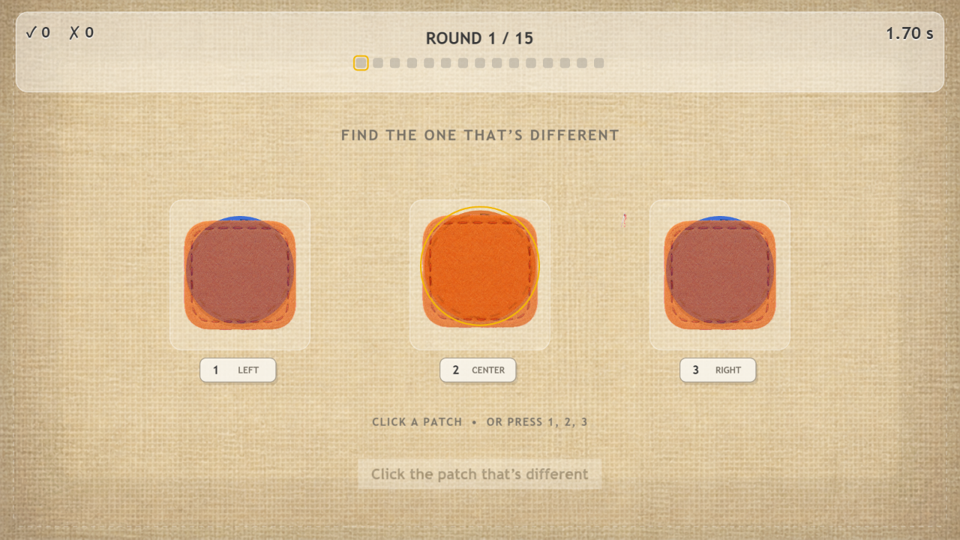}{Different Color}{Round 1: center patch}}%
            {\GQMFrame[\GQMOddCrop]{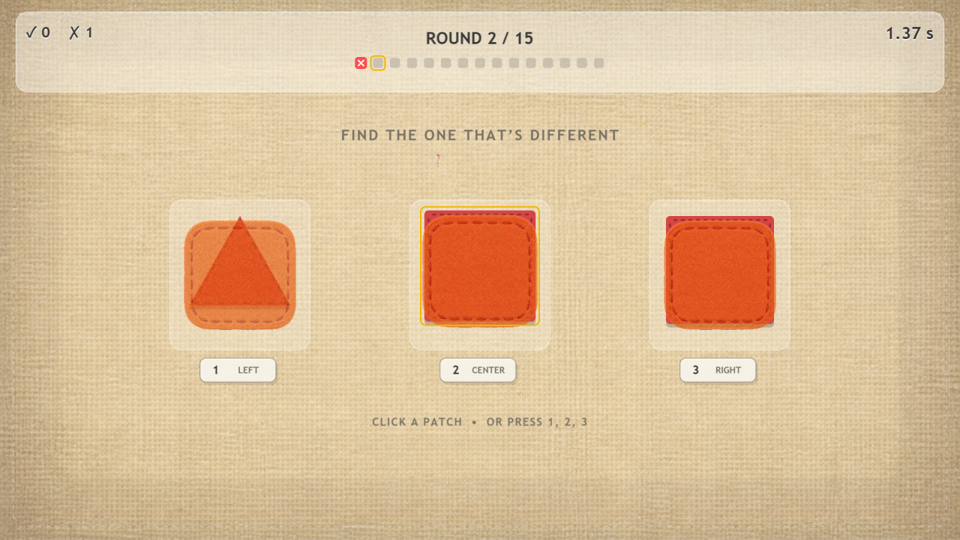}{Different Shape}{Round 2: left patch}}%
            {\GQMFrame[\GQMOddCrop]{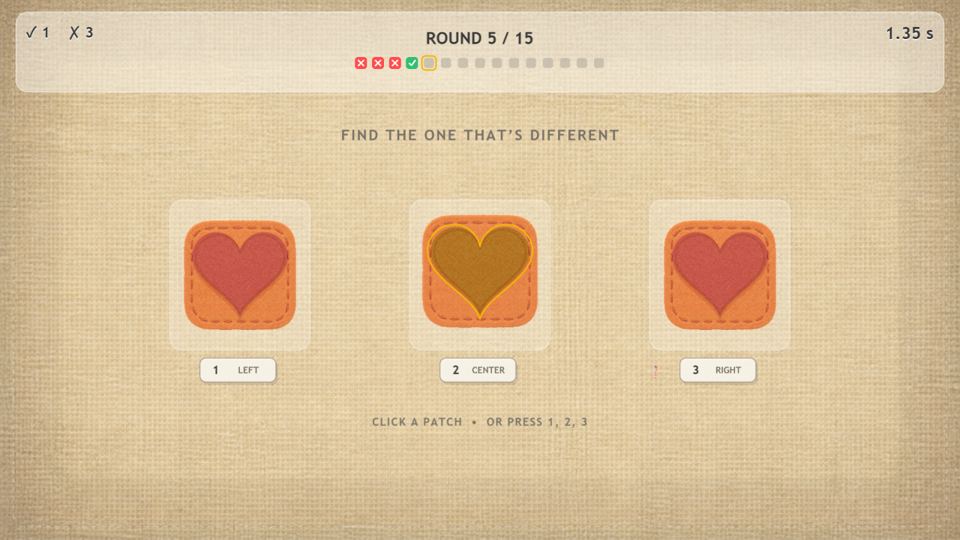}{Different Color}{Round 5: center patch}}%
        \GQMNote{Choose the patch that differs from the other two. The distinguishing attribute changes across rounds, from color to shape.}
    \end{subfigure}

    \par\vfill

    \begin{subfigure}[t]{\linewidth}
        \caption{\texttt{Orbit}: Ring Switching and Hazard Contact}
        \label{fig:gqm_orbit}
        \GQMRow%
            {\GQMFrame[\GQMOrbitCrop]{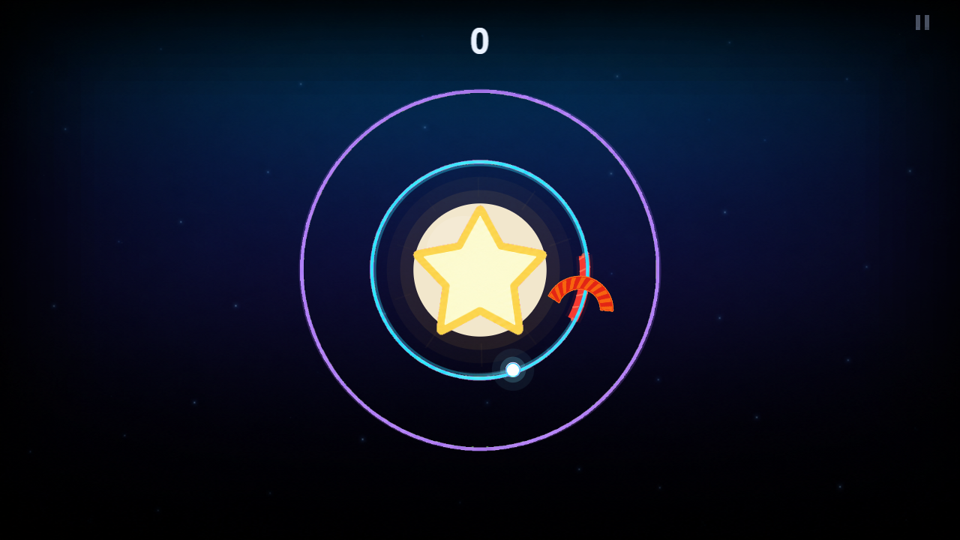}{Inner Ring}{Player on cyan orbit}}%
            {\GQMFrame[\GQMOrbitCrop]{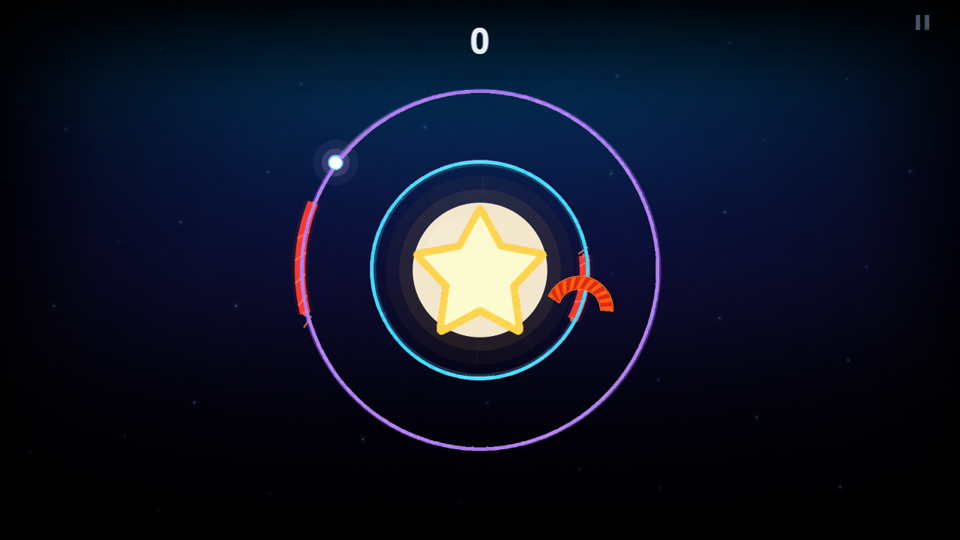}{Outer Ring}{Player on purple orbit}}%
            {\GQMFrame[\GQMOrbitCrop]{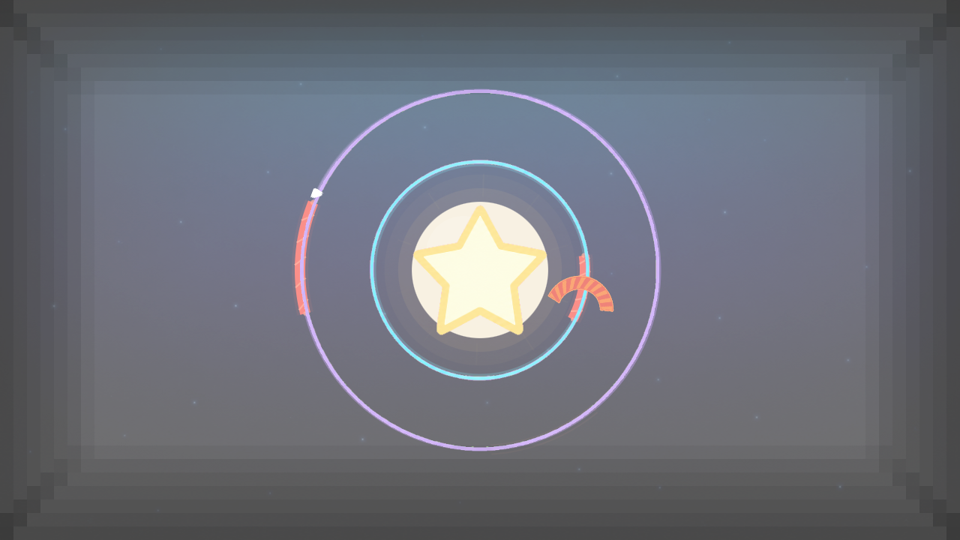}{Hazard Contact}{Visible collision flash}}%
        \GQMNote{The player moves between two concentric rings. The final frame shows a screen flash when the player reaches the red hazard.}
    \end{subfigure}

    \par\vfill

    \begin{subfigure}[t]{\linewidth}
        \caption{\texttt{Echo Three}: Observe and Repeat}
        \label{fig:gqm_echo_three}
        \GQMRow%
            {\GQMFrame[\GQMEchoCrop]{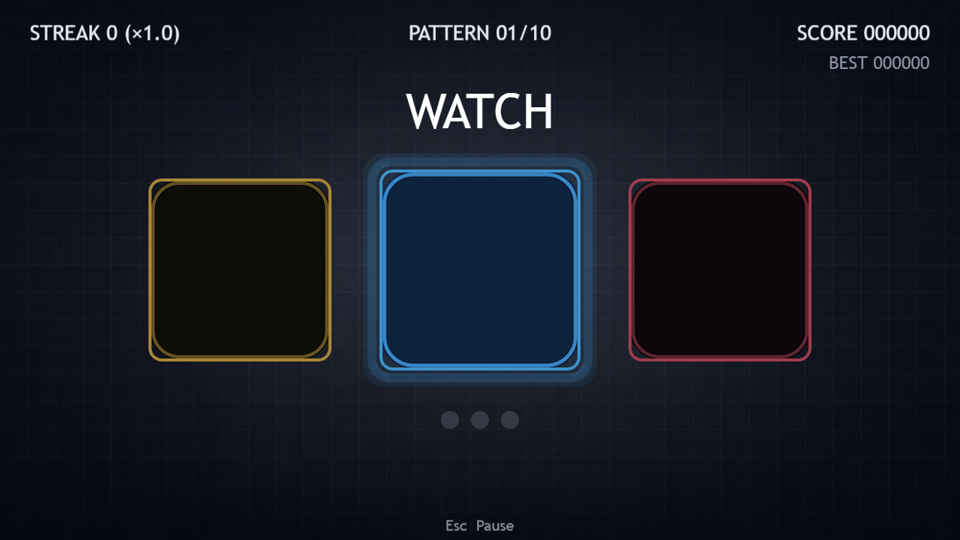}{Watch the Pattern}{Pattern 1: blue pad}}%
            {\GQMFrame[\GQMEchoCrop]{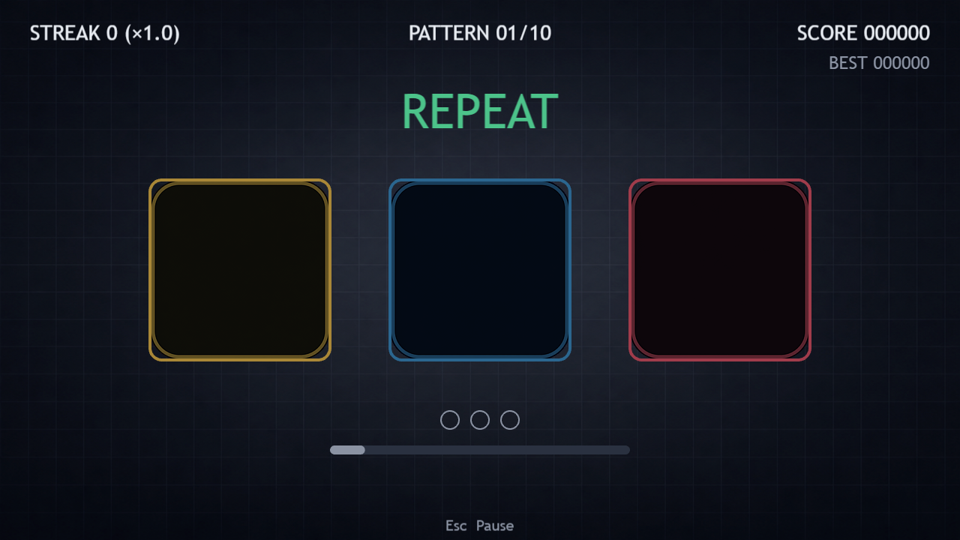}{Repeat the Pattern}{Pattern 1: input phase}}%
            {\GQMFrame[\GQMEchoCrop]{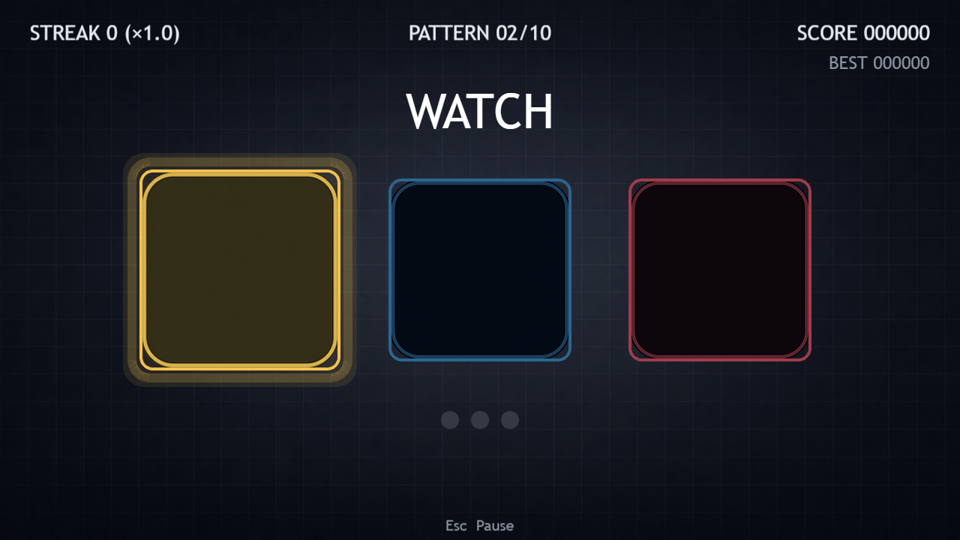}{Watch the Next Pattern}{Pattern 2: yellow pad}}%
        \GQMNote{Illuminated pads present a pattern during WATCH, followed by a timed REPEAT phase for player input. A new pattern then begins.}
    \end{subfigure}

    \par\vfill
    \caption{\textbf{Sampled gameplay in generated \emph{Small} games (01).}
    Four games from the \emph{Small} split illustrate (a) selective clicking, (b) visual discrimination, (c) ring switching and collision feedback, and (d) the observation and input phases of a memory task.
    Each row shows three states in the order of the supplied capture sequence.
    The full game screens are retained, including their prompts and feedback.}
    \label{fig:small_gameplay_01}
    \end{minipage}
\end{figure}
