# Supplementary material for: A2Z GameSpec-Bench: How Faithfully Can Coding Agents Generate Games from Game Design Specifications?
Source: arXiv:2609.39564 source file (2026-09-30)
Supplement: Supplementary file 14 [file small_gameplay_02.tex]

% Version v2: Key Under Cups, Bin Bit, Greedy Die, Safe Dial.
% Required preamble packages: graphicx, subcaption.
% Place this file in the manuscript root, then use:
% \input{small_gameplay}
% Revised selection: four additional Small games, three images per row.
% All layout, text, labels, and crop margins are editable in this file.
% Keep the supplied original PNGs unchanged.

\begin{figure}[p]
    \centering
    % Match the full text-area height, including the caption.
    % Flexible row spacing preserves all screenshot aspect ratios.
    \begin{minipage}[t][\textheight][s]{\linewidth}
    \vspace{0pt}
    \captionsetup{font=small,skip=7pt}
    \renewcommand{\thesubfigure}{(\alph{subfigure})}
    \captionsetup[subfigure]{font={small,bf},labelformat=simple,labelsep=space,justification=raggedright,singlelinecheck=false,position=top,skip=5pt,hypcap=true}

    % Crop margins: LEFT BOTTOM RIGHT TOP, before resizing.
    % All panels currently show the complete original screenshots.
    % Original size: 1920 x 1080, except Greedy Die at 1280 x 720.
    % The PNGs have no DPI metadata; 1 bp corresponds to one source pixel
    % with the standard 72 dpi image default.
    \newcommand{\SGECupsCrop}{0bp 0bp 0bp 0bp}
    \newcommand{\SGEBinCrop}{0bp 0bp 0bp 0bp}
    \newcommand{\SGEDieCrop}{0bp 0bp 0bp 0bp}
    \newcommand{\SGEDialCrop}{0bp 0bp 0bp 0bp}
    \newcommand{\SGEFrameWidth}{0.322\linewidth}
    \newcommand{\SGEPanelGap}{13pt}
    \newcommand{\SGELabelFont}{\fontsize{8}{9.2}\selectfont}
    \newcommand{\SGEDetailFont}{\fontsize{7.5}{8.5}\selectfont}

    % Arguments: [crop margins], original PNG path, label, visible detail.
    \newcommand{\SGEFrame}[4][0bp 0bp 0bp 0bp]{%
        \begin{minipage}[t]{\SGEFrameWidth}
            \centering
            \edef\SGEImageOptions{trim=#1,clip,width=\the\linewidth}
            \expandafter\includegraphics\expandafter[\SGEImageOptions]{#2}\par
            \vspace{3pt}
            {\SGELabelFont\textbf{#3}\par}
            \vspace{1pt}
            {\SGEDetailFont #4\par}
        \end{minipage}%
    }

    % The unbreakable horizontal box guarantees three image columns.
    \newcommand{\SGERow}[3]{%
        \noindent\hbox to\linewidth{#1\hfil#2\hfil#3}\par
    }
    \newcommand{\SGENote}[1]{%
        \vspace{5pt}
        {\fontsize{8.5}{10}\selectfont\raggedright #1\par}
    }

    \begin{subfigure}[t]{\linewidth}
        \caption{\texttt{Key Under Cups}: Visual Tracking and Reveal}
        \label{fig:sge_key_under_cups}
        \SGERow%
            {\SGEFrame[\SGECupsCrop]{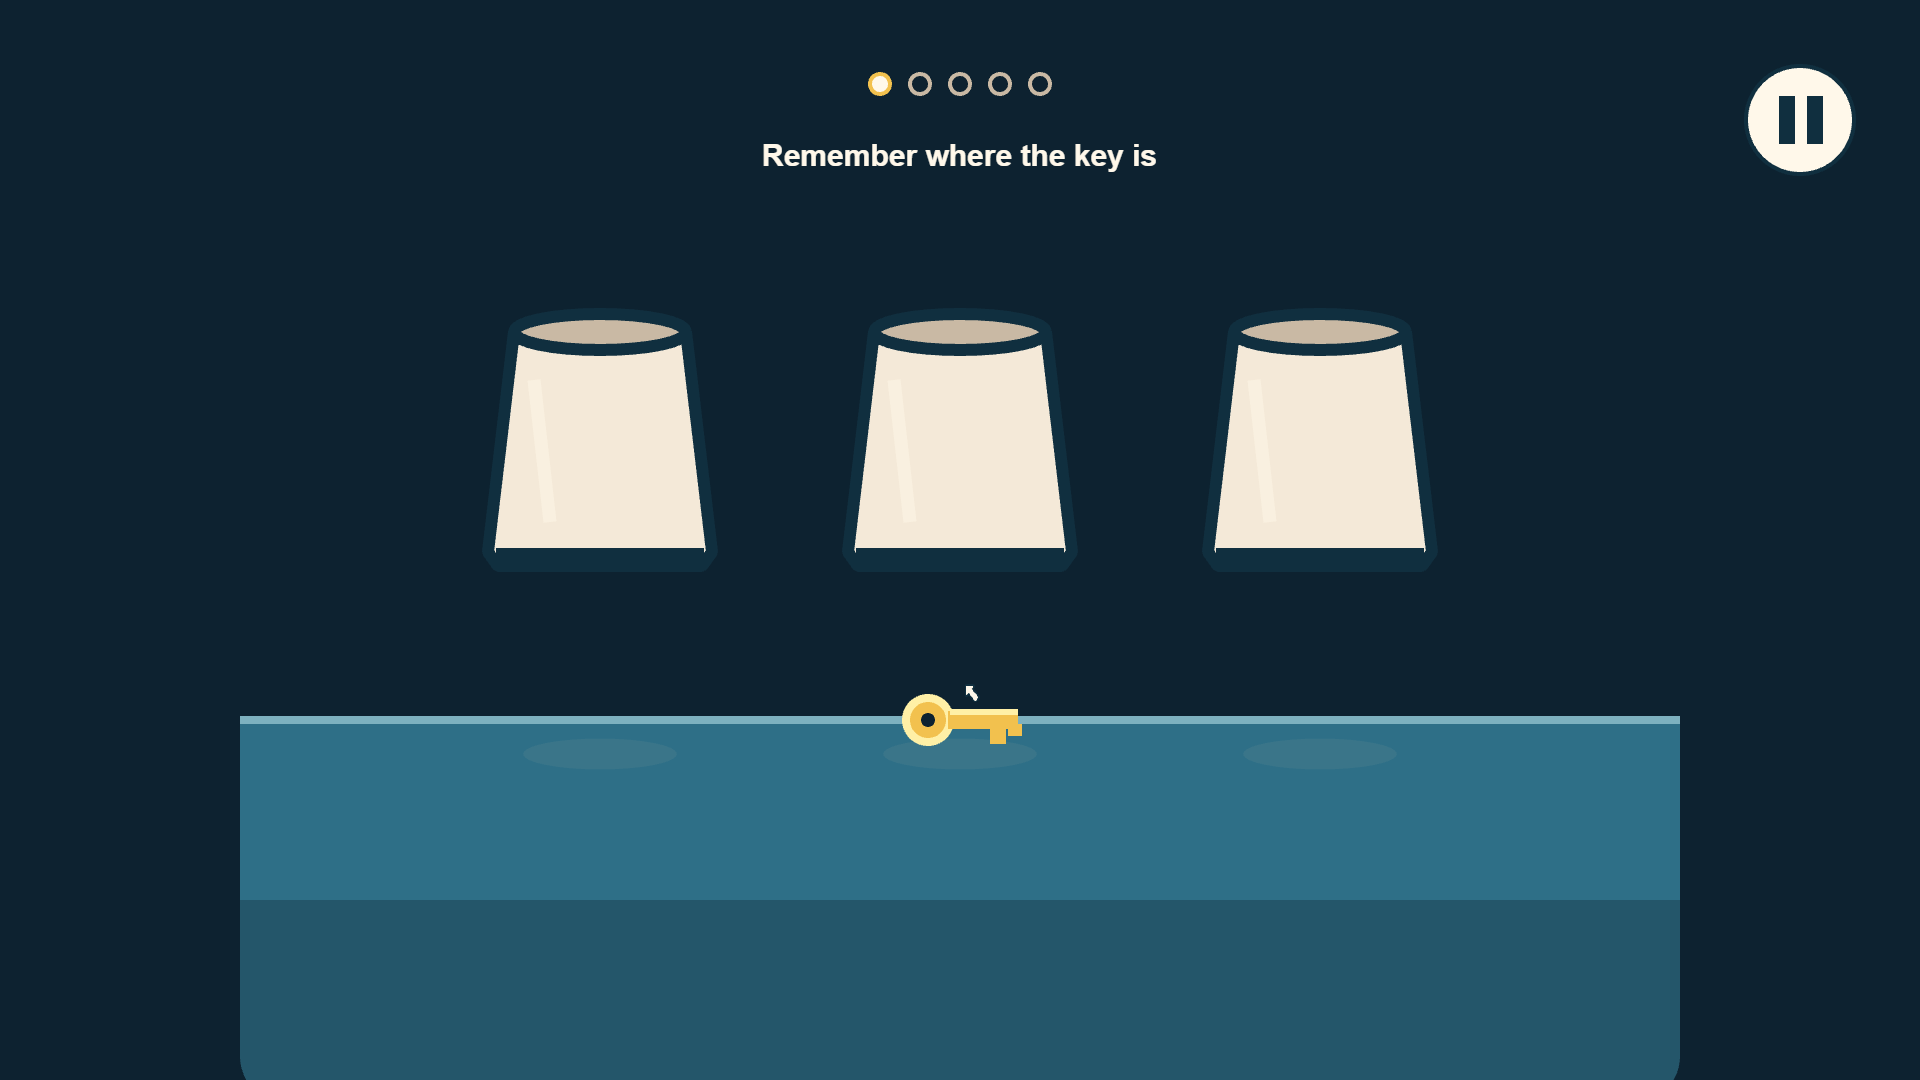}{Remember the Key}{Key exposed before shuffling}}%
            {\SGEFrame[\SGECupsCrop]{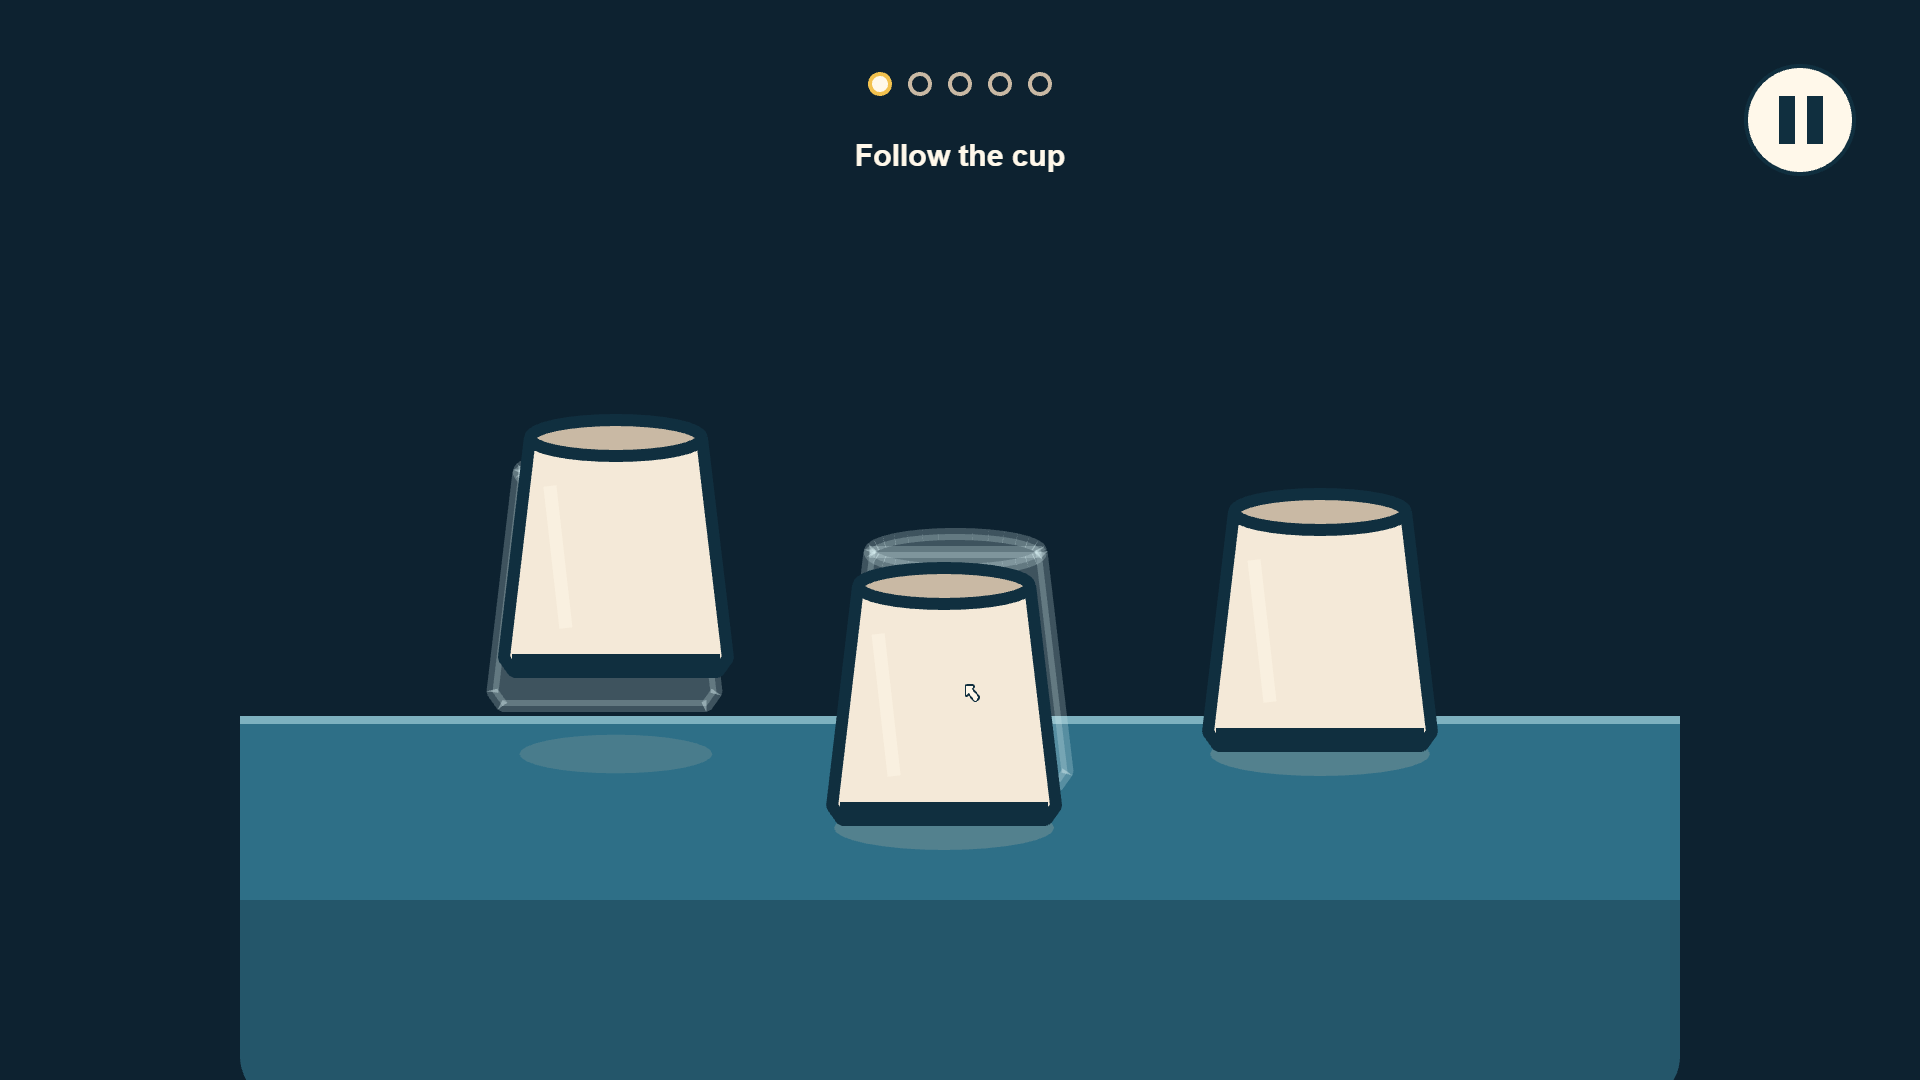}{Follow the Shuffle}{Cups exchange positions}}%
            {\SGEFrame[\SGECupsCrop]{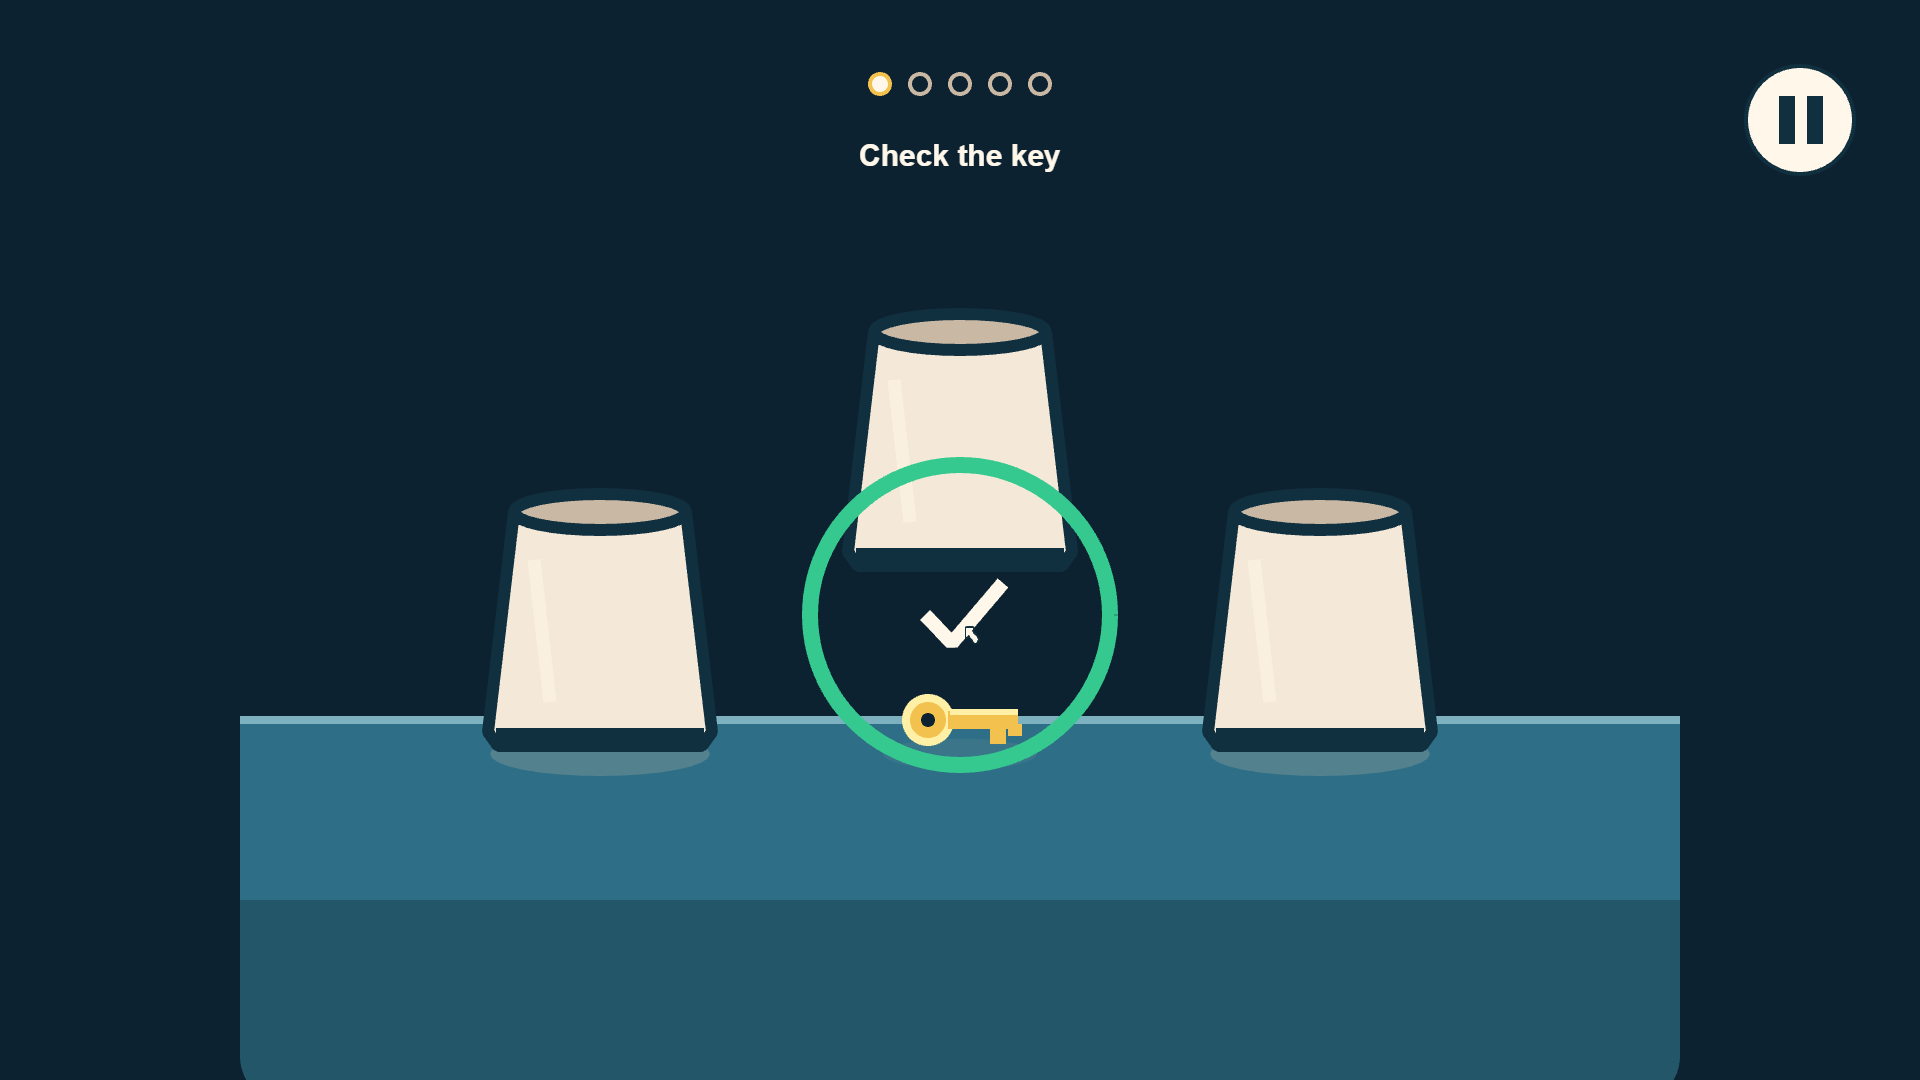}{Check the Choice}{Key and correct-answer mark}}%
        \SGENote{The key is revealed before the cups move. After the shuffle, the selected cup lifts to expose the key, accompanied by a green check mark.}
    \end{subfigure}

    \par\vfill

    \begin{subfigure}[t]{\linewidth}
        \caption{\texttt{Bin Bit}: Shape Sorting and Immediate Feedback}
        \label{fig:sge_bin_bit}
        \SGERow%
            {\SGEFrame[\SGEBinCrop]{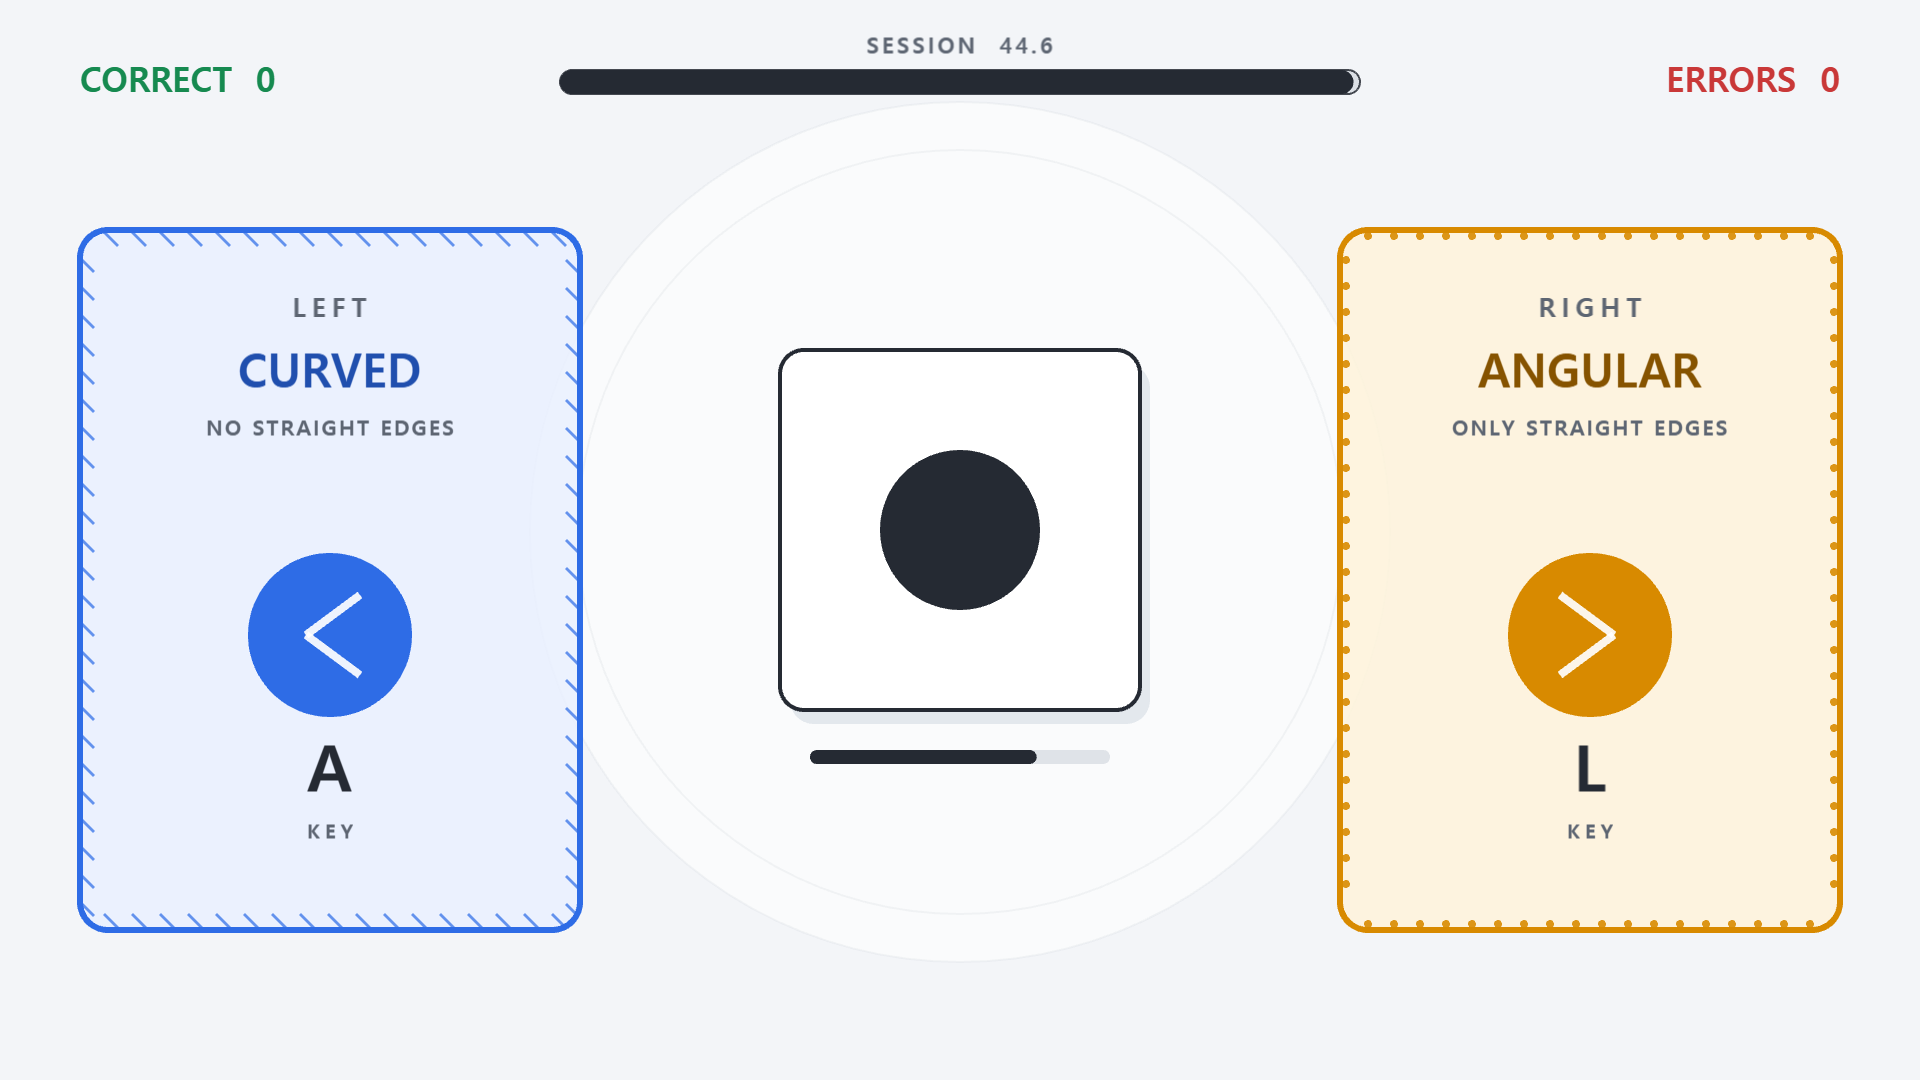}{Read the Shape}{Circle prompt; correct count 0}}%
            {\SGEFrame[\SGEBinCrop]{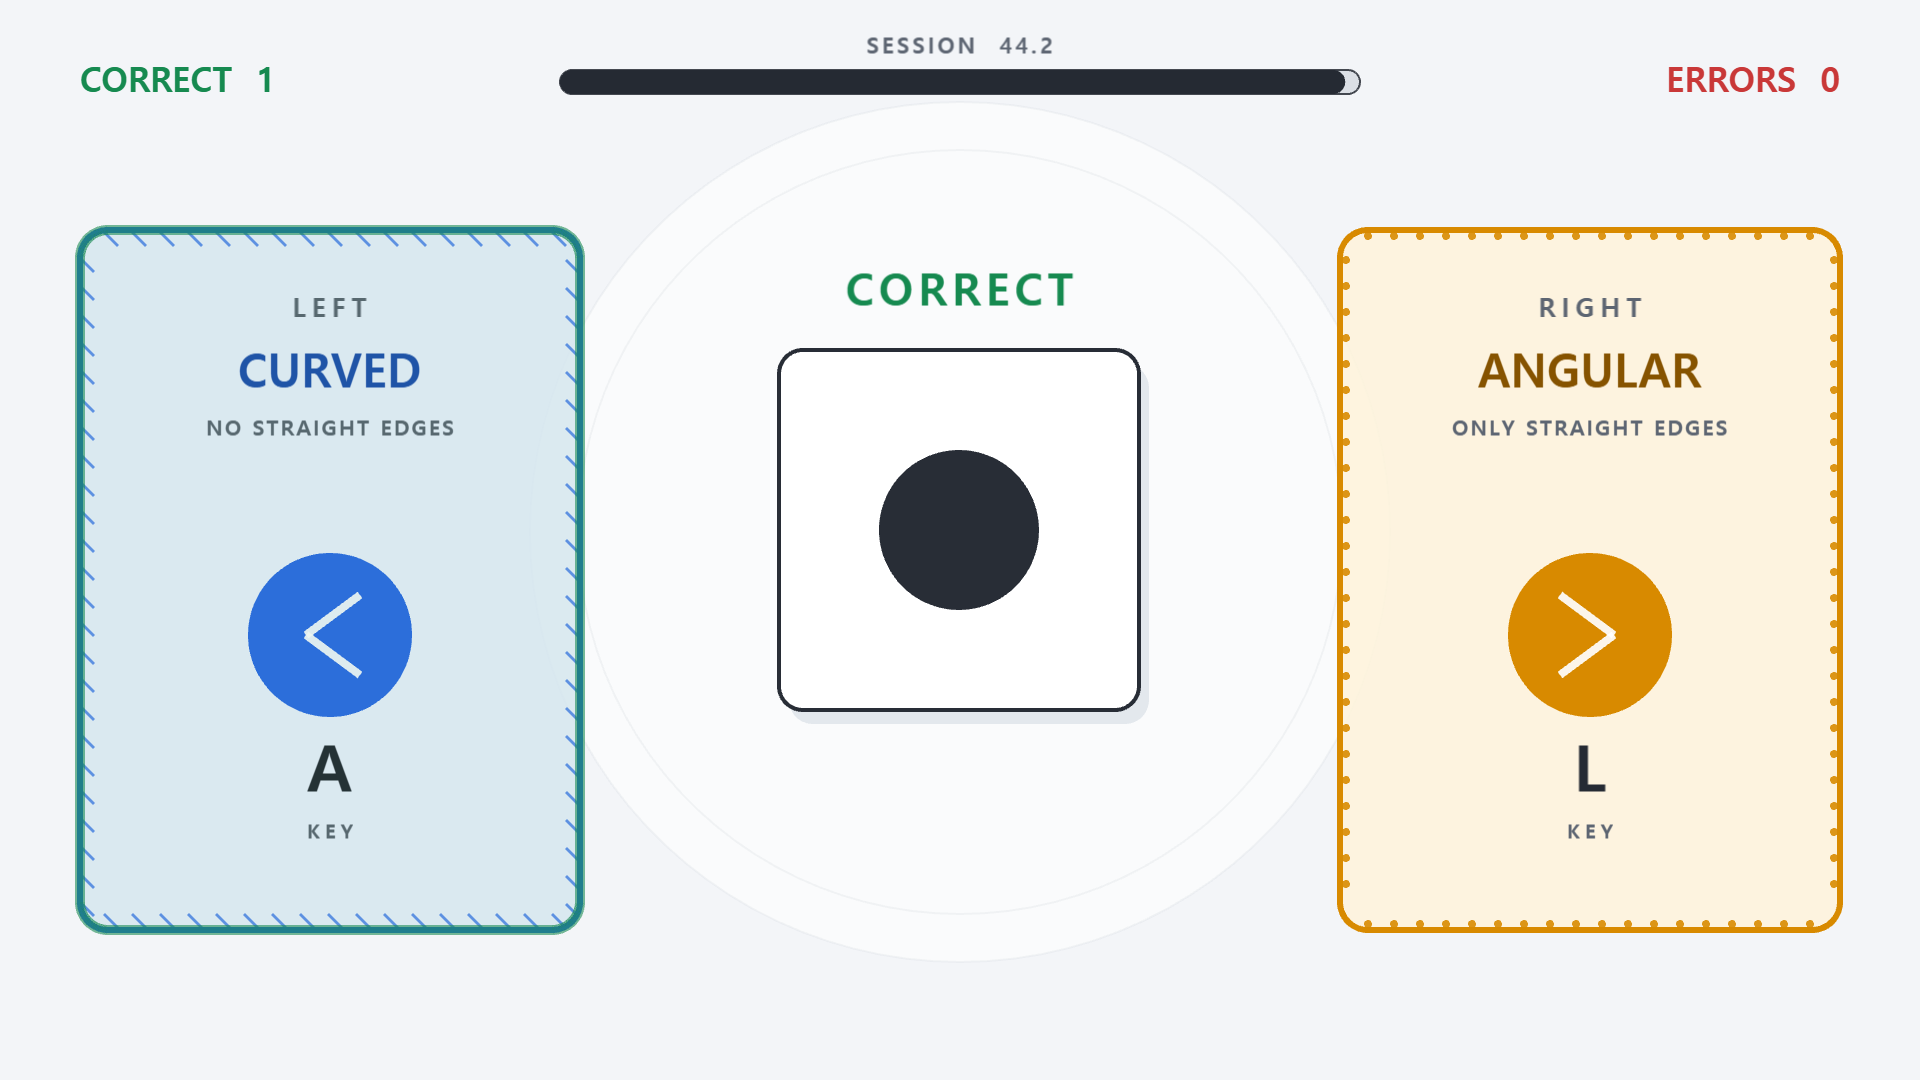}{Choose Curved}{Left bin highlighted; count 1}}%
            {\SGEFrame[\SGEBinCrop]{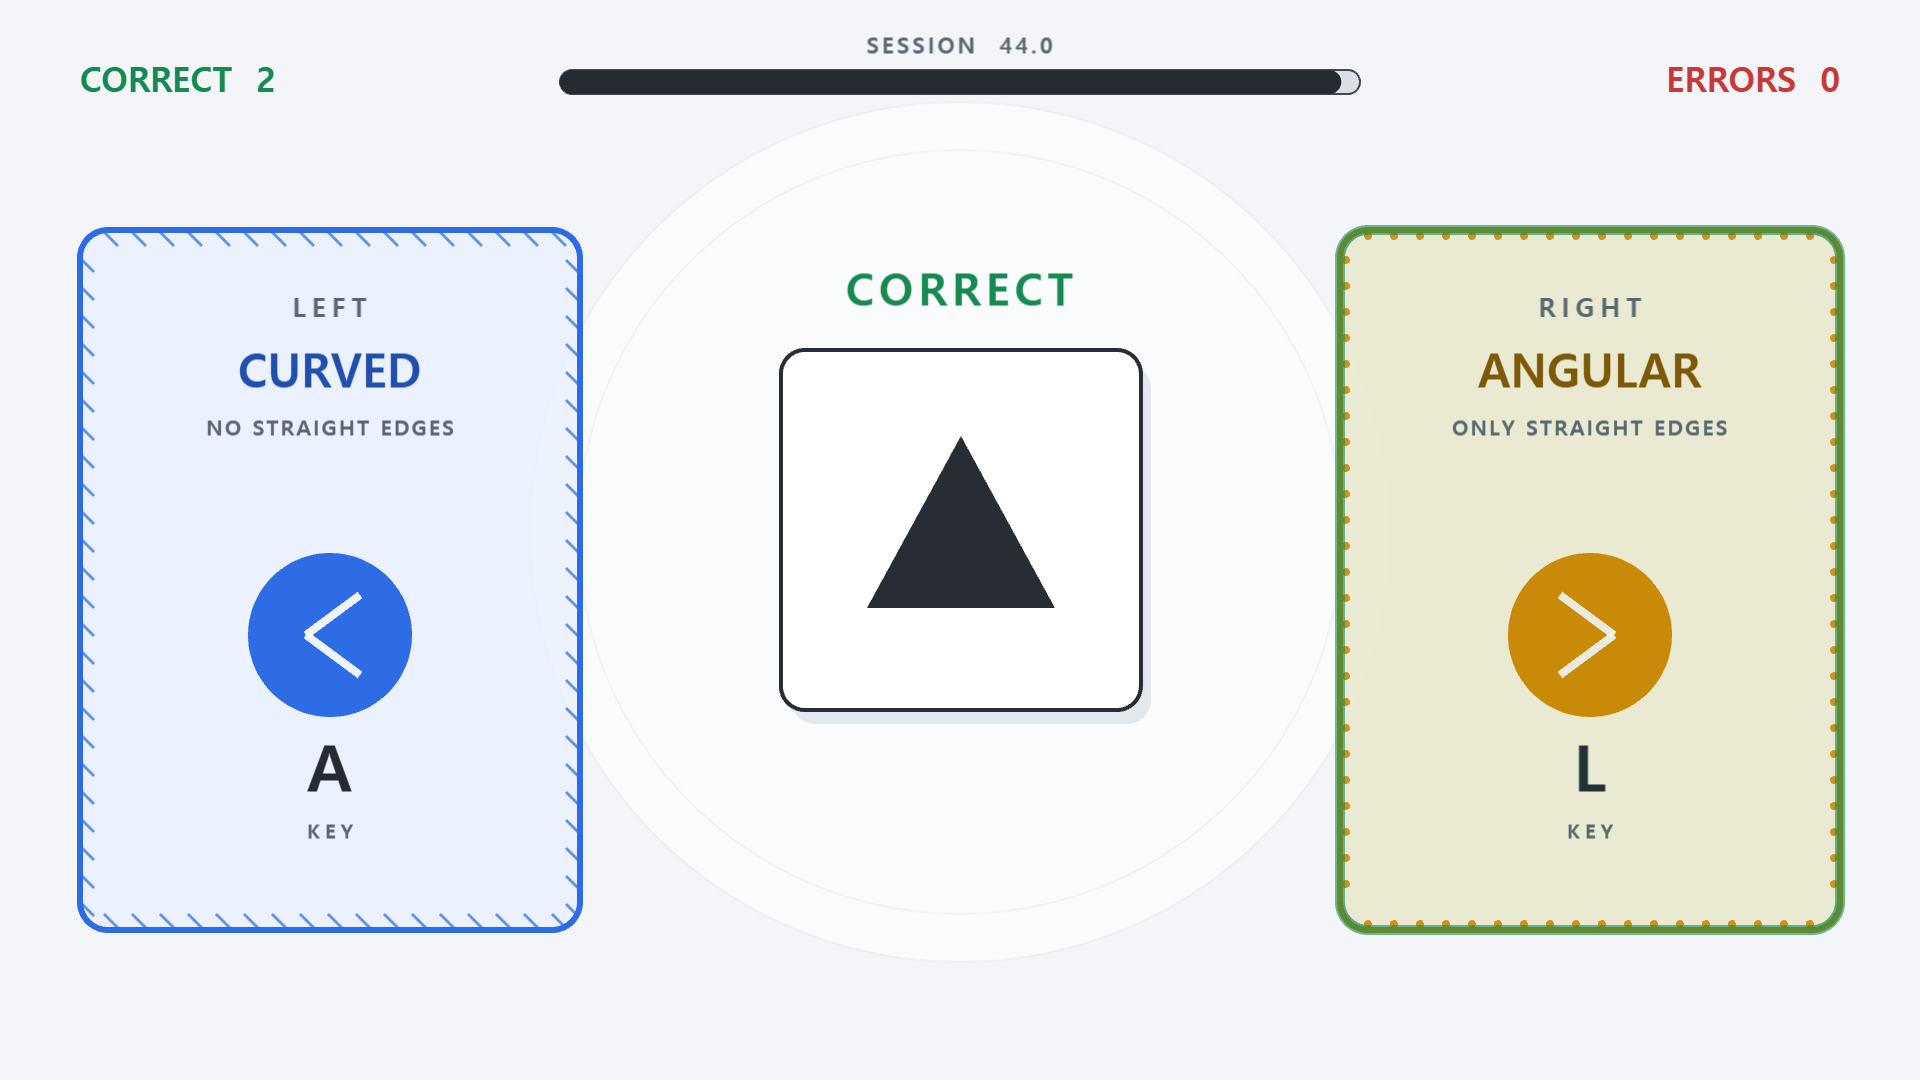}{Choose Angular}{Right bin highlighted; count 2}}%
        \SGENote{Blue and gold bins retain their curved and angular labels. Correct choices highlight the corresponding bin and increment the visible counter.}
    \end{subfigure}

    \par\vfill

    \begin{subfigure}[t]{\linewidth}
        \caption{\texttt{Greedy Die}: Rolling, Accumulation, and Banking}
        \label{fig:sge_greedy_die}
        \SGERow%
            {\SGEFrame[\SGEDieCrop]{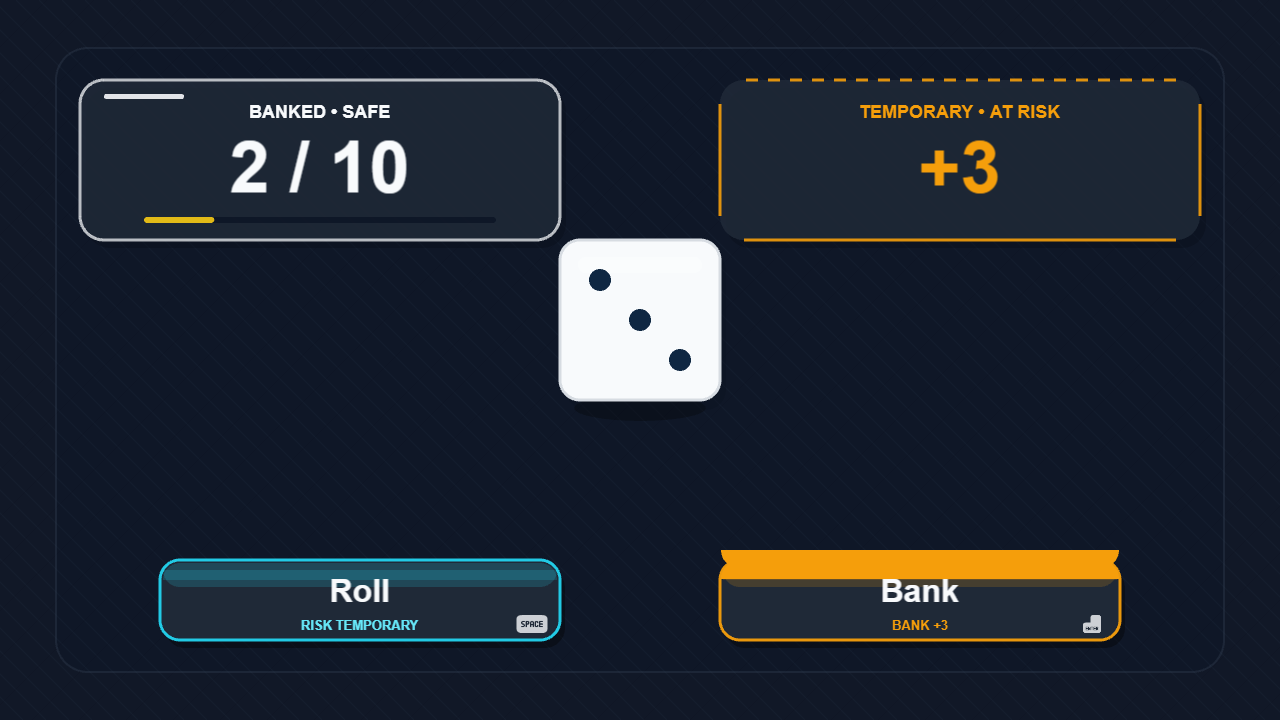}{Choose Roll or Bank}{Banked: 2; temporary: +3}}%
            {\SGEFrame[\SGEDieCrop]{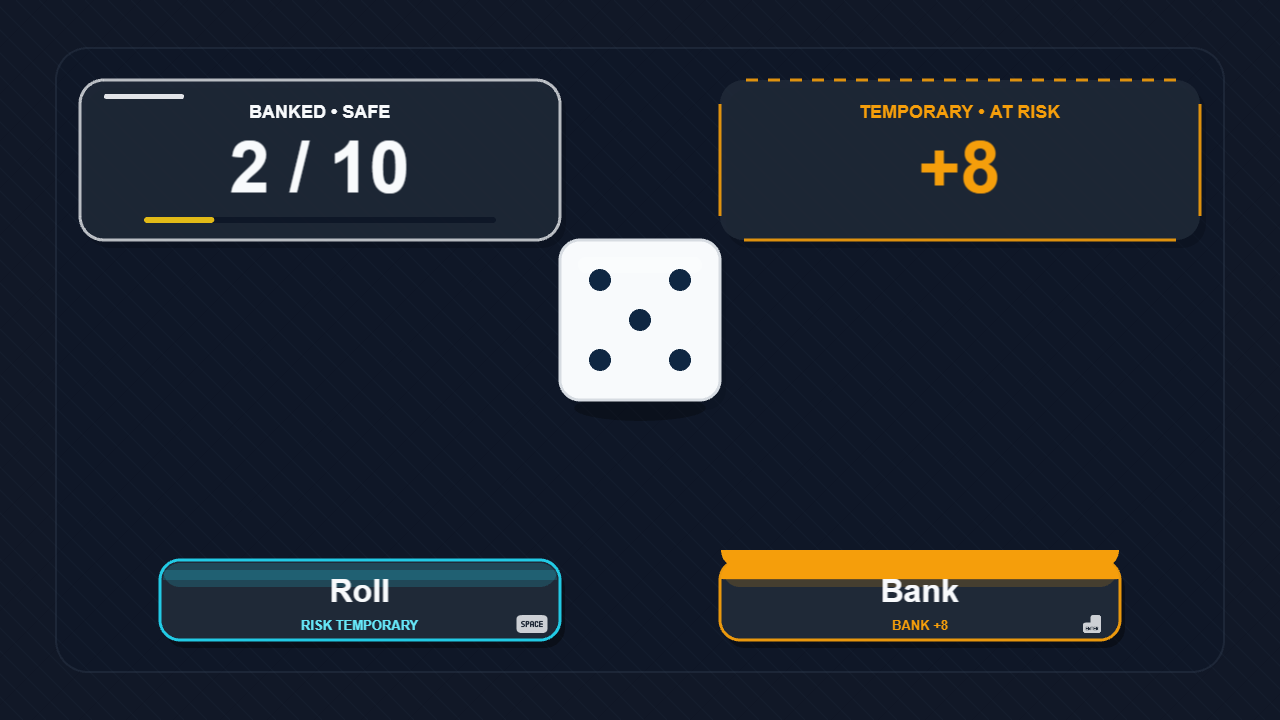}{Accumulate Points}{Roll of 5; temporary: +8}}%
            {\SGEFrame[\SGEDieCrop]{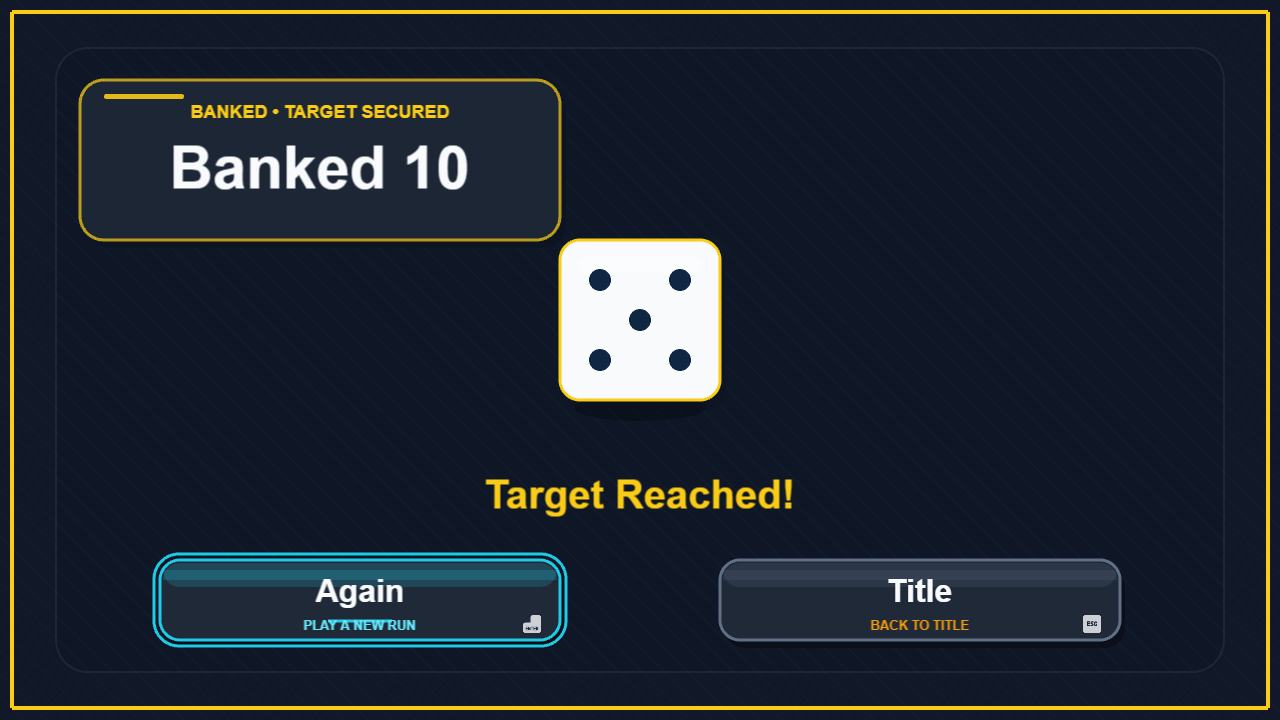}{Bank the Total}{Banked: 10; target reached}}%
        \SGENote{Separate panels distinguish banked points from the temporary total. Rolling adds five temporary points; banking then secures the target of ten.}
    \end{subfigure}

    \par\vfill

    \begin{subfigure}[t]{\linewidth}
        \caption{\texttt{Safe Dial}: Dial Rotation and Combination Cues}
        \label{fig:sge_safe_dial}
        \SGERow%
            {\SGEFrame[\SGEDialCrop]{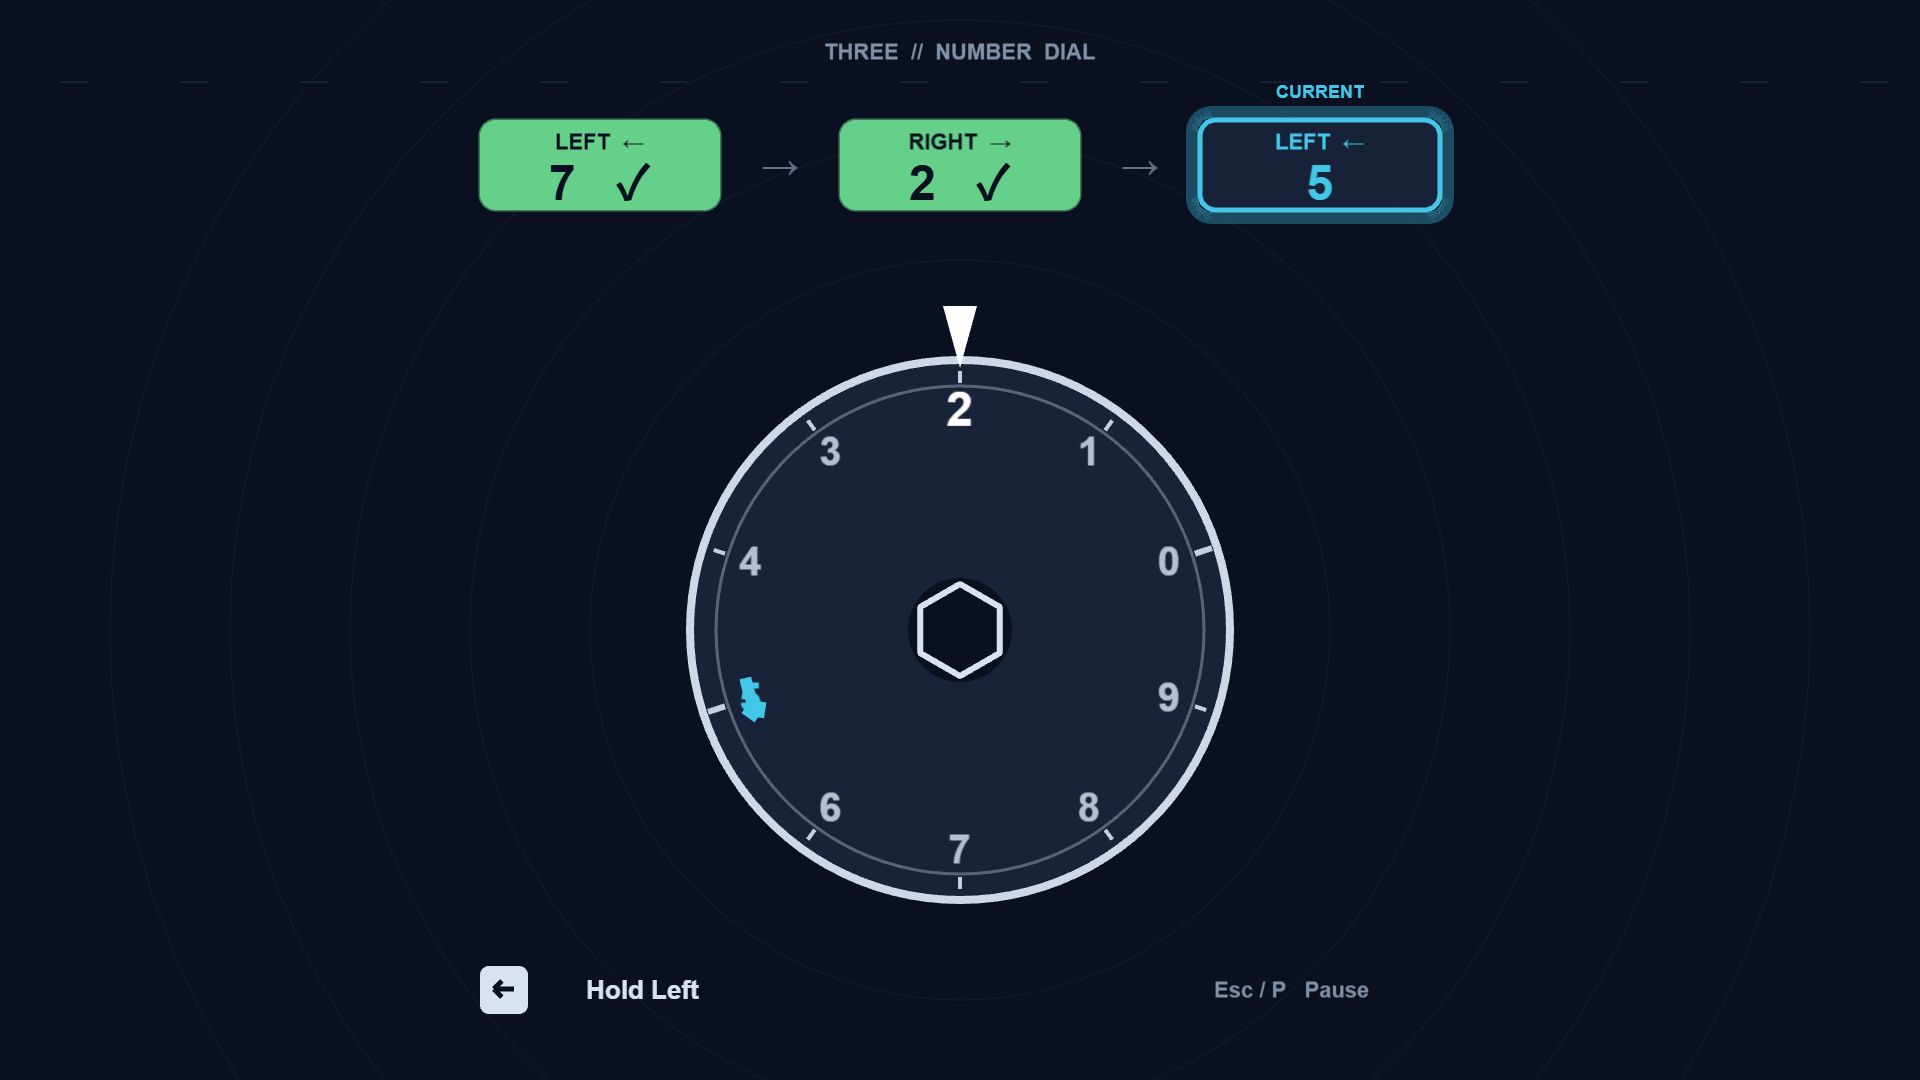}{Read the Next Target}{Entries 7 and 2 confirmed}}%
            {\SGEFrame[\SGEDialCrop]{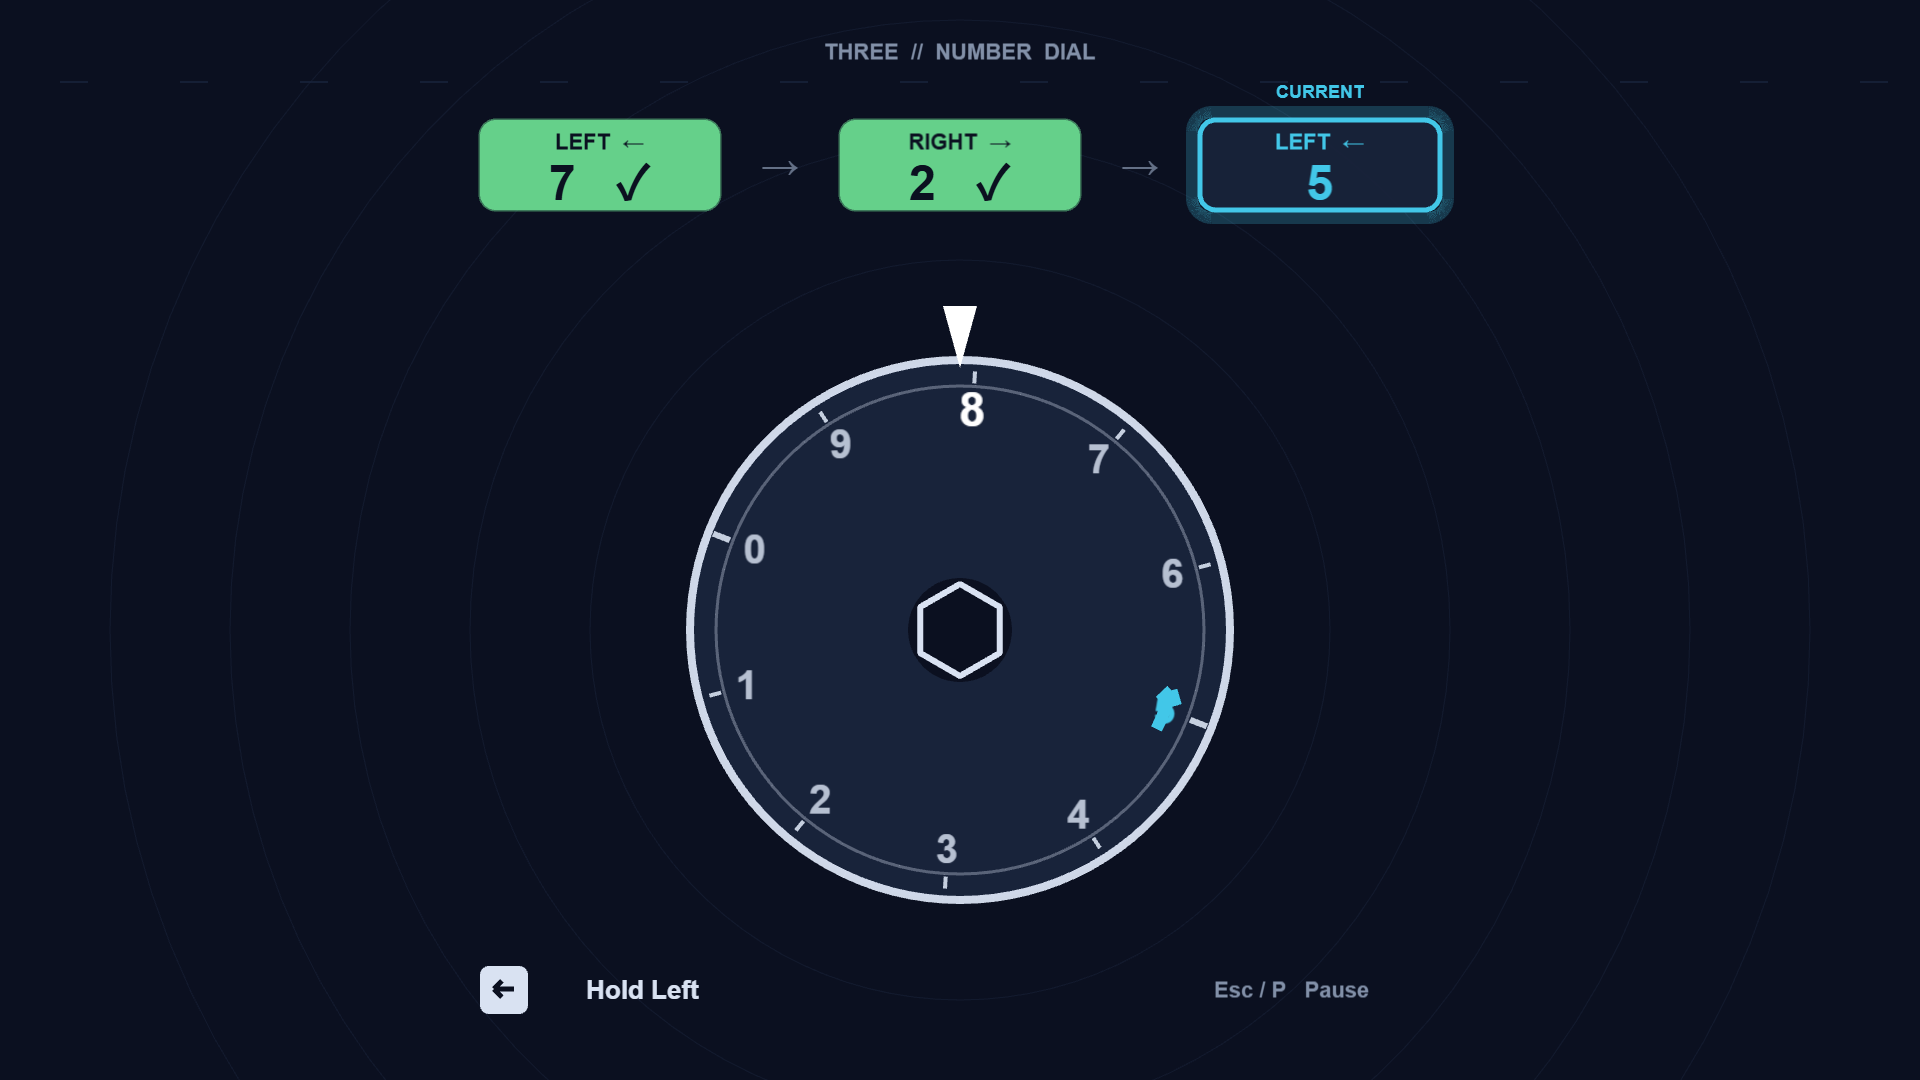}{Rotate the Dial}{Final target: left to 5}}%
            {\SGEFrame[\SGEDialCrop]{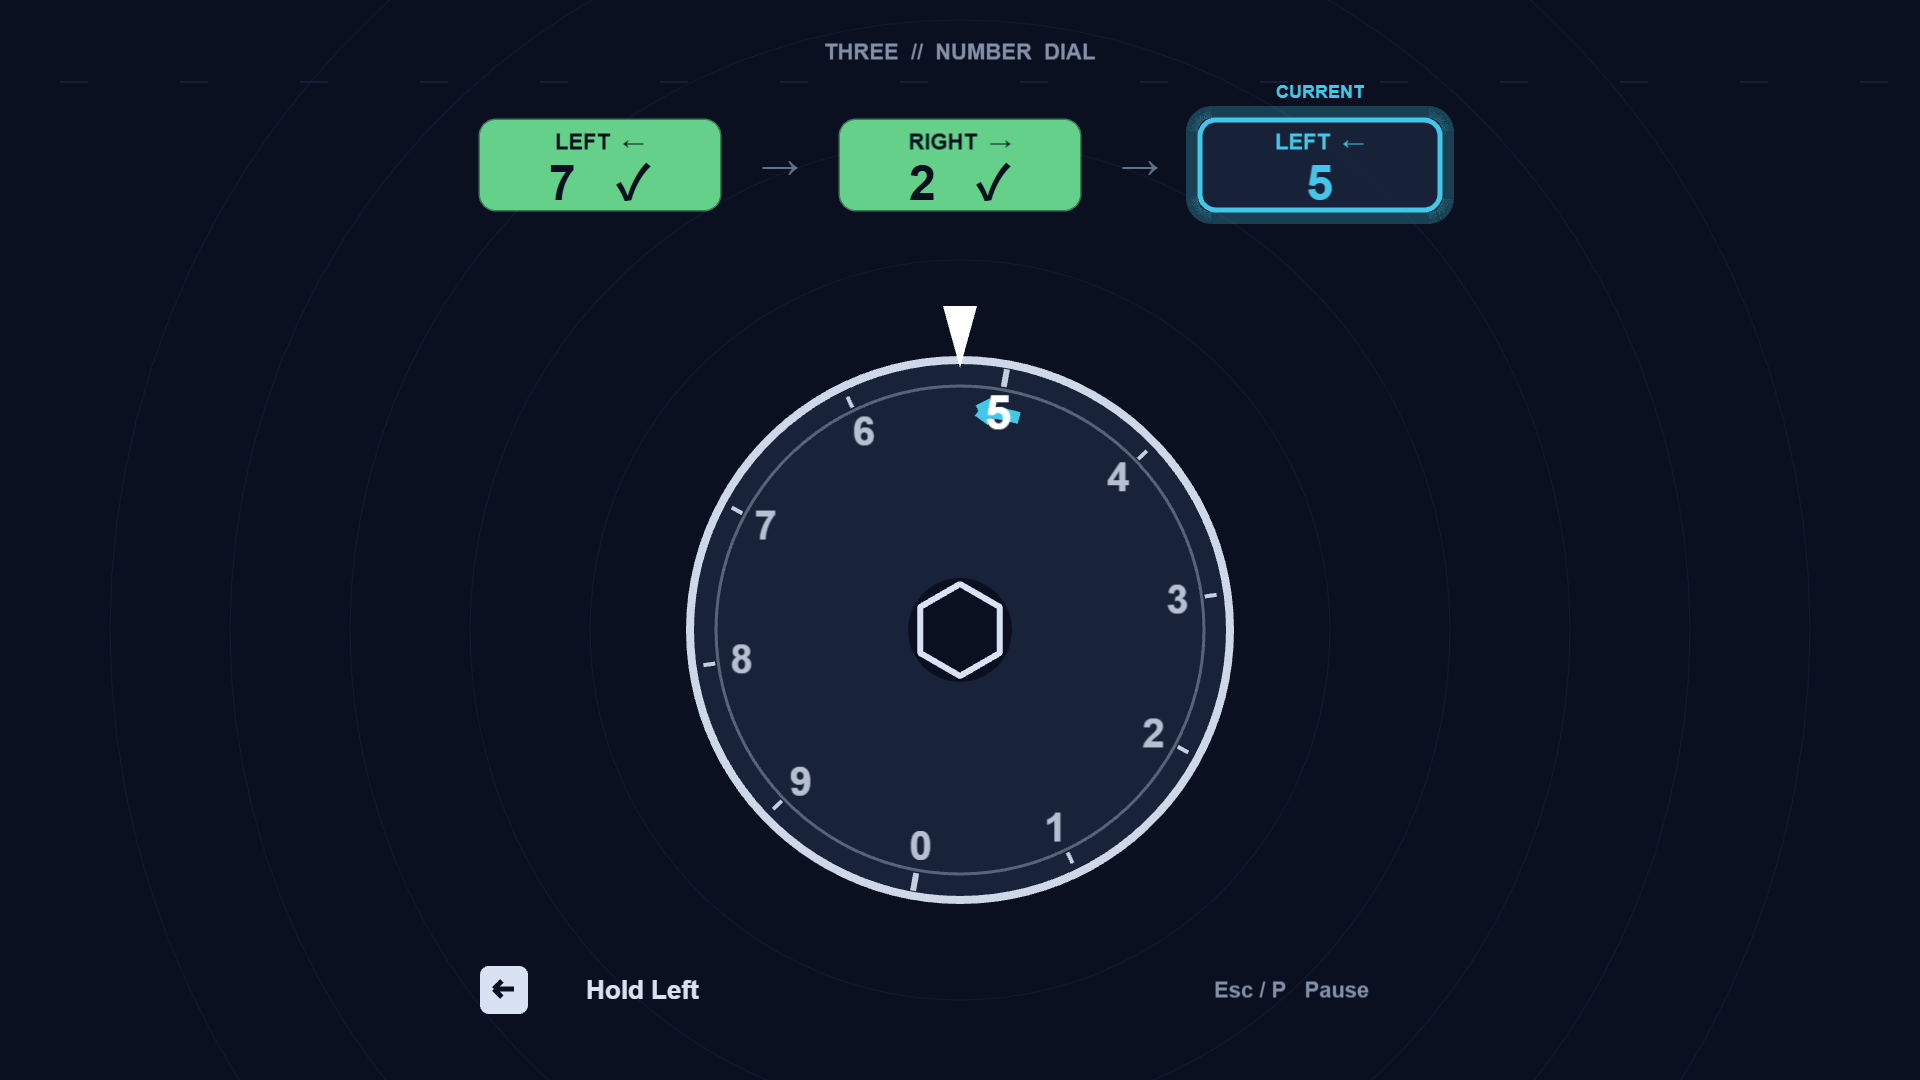}{Approach the Pointer}{Highlighted 5 near the pointer}}%
        \SGENote{With two entries already confirmed, the dial rotates toward the highlighted final target. A fixed pointer and progress cards expose the current state.}
    \end{subfigure}

    \par\vfill
    \caption{\textbf{Sampled gameplays in generated~\emph{Small} games (02)}
    Additional four frames illustrate (a) tracking a hidden key through a cup shuffle, (b) sorting curved and angular shapes, (c) accumulating and banking dice points, and (d) rotating a combination dial with persistent progress cues.
    Each row contains three full screenshots from one replay scenario, ordered from left to right.}
    \label{fig:small_gameplay_02}
    \end{minipage}
\end{figure}
