# Supplementary material for: A2Z GameSpec-Bench: How Faithfully Can Coding Agents Generate Games from Game Design Specifications?
Source: arXiv:2609.39564 source file (2026-09-30)
Supplement: Supplementary file 15 [file big_gdd_feats.tex]

\begin{table}[t]
    \centering
    \caption{\textbf{Genre distribution of the \emph{Big} GDD split.}}
    \label{tab:big-genre-distribution}

    \scriptsize
    \setlength{\tabcolsep}{4pt}
    \renewcommand{\arraystretch}{1.08}

    \begin{tabularx}{\linewidth}{
        @{}
        c
        >{\raggedright\arraybackslash}p{0.27\linewidth}
        c
        >{\raggedright\arraybackslash}X
        @{}
    }
        \toprule
        \# & Genre & $n$ & Games \\
        \midrule

        1
        & Platformer \& Metroidvania
        & 7
        & \texttt{afterglow},
          \texttt{chromashade},
          \texttt{rainwright},
          \texttt{ssitgim},
          \texttt{turning\_keep},
          \texttt{neon\_spray},
          \texttt{the\_librarians\_hook}
        \\

        2
        & Action Roguelite \& Survival
        & 4
        & \texttt{abyssal\_chain},
          \texttt{seamline},
          \texttt{todays\_best\_spot},
          \texttt{afterglow\_network}
        \\

        3
        & Shooter \& Bullet-hell
        & 3
        & \texttt{golem\_workshop},
          \texttt{magma\_arc},
          \texttt{snowfall\_draw}
        \\

        4
        & Rhythm
        & 4
        & \texttt{beat\_reroute},
          \texttt{beatstorm},
          \texttt{cloud\_cast},
          \texttt{rhythm\_of\_response}
        \\

        5
        & Puzzle
        & 4
        & \texttt{chameleon\_slide},
          \texttt{fable\_knot},
          \texttt{fogfall\_delivery},
          \texttt{u001\_toyfit}
        \\

        6
        & Strategy \& Tactics
        & 5
        & \texttt{ashen\_citadel},
          \texttt{gateline\_2d},
          \texttt{siege\_deck\_2d},
          \texttt{chroma\_bastion},
          \texttt{xl001\_edens\_debt}
        \\

        7
        & RPG
        & 4
        & \texttt{four\_of\_the\_depths},
          \texttt{linkbound},
          \texttt{dh001\_echo\_gate\_guild},
          \texttt{borrowed\_faces\_2d}
        \\

        8
        & Simulation \& Management
        & 8
        & \texttt{anomaly\_factory},
          \texttt{grand\_atelier\_2d},
          \texttt{night\_shift\_rx},
          \texttt{rainbow\_hoof},
          \texttt{reef\_bistro},
          \texttt{strata\_keepers},
          \texttt{wham\_bam\_logistics},
          \texttt{wind\_winter\_camp}
        \\

        9
        & Idle \& Clicker
        & 2
        & \texttt{alias\_alchemy\_shop},
          \texttt{hell\_casino}
        \\

        10
        & Adventure \& Narrative
        & 6
        & \texttt{cold\_case\_archive},
          \texttt{u003\_acting\_human\_again},
          \texttt{whispers\_of\_the\_wild},
          \texttt{harukaze\_student\_council\_casebook},
          \texttt{last\_announcement},
          \texttt{backwalker\_camp}
        \\

        11
        & Sports \& Racing
        & 3
        & \texttt{last\_catch},
          \texttt{pixel\_pennant},
          \texttt{toybox\_rider}
        \\

        \bottomrule
    \end{tabularx}
\end{table}
