# Supplementary material for: A2Z GameSpec-Bench: How Faithfully Can Coding Agents Generate Games from Game Design Specifications?
Source: arXiv:2609.39564 source file (2026-09-30)
Supplement: Supplementary file 16 [file criteria_for_gdd.tex]

\begin{table*}[t]
\centering\small
\caption{\textbf{Criteria for golden GDDs.} Each criterion excludes one way a GDD can
invalidate conformance-based evaluation. Example violations are taken from our validation logs.}
\setlength{\tabcolsep}{6pt}
\renewcommand{\arraystretch}{1.1}
% X columns vertically centered; relative widths via \hsize (sum = 3)
\renewcommand{\tabularxcolumn}[1]{m{#1}}
\newcommand{\crit}[3]{\begin{tabular}[c]{@{}c@{}}\textbf{#1}\\[1pt] #2\\ #3\end{tabular}}
\newcommand{\bl}[1]{\par\noindent\hangindent=0.9em\hangafter=1\makebox[0.9em][l]{\textbullet}#1}
\begin{tabularx}{\textwidth}{@{}>{\centering\arraybackslash}m{2.1cm}
  >{\raggedright\arraybackslash\hsize=1.15\hsize}X
  >{\raggedright\arraybackslash\itshape\hsize=0.85\hsize}X
  >{\raggedright\arraybackslash\hsize=1.0\hsize}X@{}}
\toprule
\textbf{Criterion} & \textbf{Requirement} & \textbf{\upshape Failure if violated} & \textbf{Example violation} \\
\midrule
\crit{G1}{Structural}{Conformance}
& \bl{Standalone, all sections present}
  \bl{No empty or \texttt{[TBD]} section}
  \bl{No dangling identifier}
& The requirement cannot be checked.
& A section cited elsewhere had been removed. \\
\addlinespace[5pt]
\crit{G2}{Referential}{Consistency}
& \bl{One canonical definition (\texttt{DBT-}$n$)}
  \bl{Every citation resolves}
  \bl{Repeated values agree}
& Contradictions; no implementation can satisfy all.
& \texttt{bool[56]} declared for 55 species; 1~wave in App.~A vs.\ 3 in App.~B. \\
\addlinespace[5pt]
\crit{G3}{Behavioral}{Soundness}
& \bl{Total, deterministic rule tables}
  \bl{No unreachable or dead mechanic}
  \bl{Difficulty never decreases}
& Faithful implementations are penalized.
& A 90\,s boss timer never fires; HP decay kills the patient at 40\,s. \\
\addlinespace[5pt]
\crit{G4}{Executable}{Formulas}
& \bl{Variables bound to constants}
  \bl{Fixed evaluation order, bounds}
  \bl{Worked example that recomputes}
& Agent and evaluator can compute different answers.
& Kill time ignores the boss's DEF; \texttt{ceil(50/4)} written as 12. \\
\bottomrule
\end{tabularx}

\label{tab:golden_criteria}
\end{table*}
