# Supplementary material for: A2Z GameSpec-Bench: How Faithfully Can Coding Agents Generate Games from Game Design Specifications?
Source: arXiv:2609.39564 source file (2026-09-30)
Supplement: Supplementary file 17 [file gdd_causal_dataset.tex]

\begin{table}[t]
    \centering
    \small
    \setlength{\tabcolsep}{6pt}
    \renewcommand{\arraystretch}{1.08}
    \caption{
        \textbf{Causal-sentence estimates in external game-design corpora.}
        Rates are CiRA predictions on retained prose.
        The pooled rate weights corpora by sentence count, while the macro average gives equal weight to the three corpora.
    }
    \label{tab:causality_corpora}
    \begin{tabular}{lrrr}
        \toprule
        \textbf{Corpus} & \textbf{Documents} & \textbf{Sentences} & \textbf{Causal} (\%) \\
        \midrule
        Studio GDDs                   & 10  & 11,741 & 37.9 \\
        Game benchmark specifications & 246 & 11,441 & 32.0 \\
        Board game rulebooks          & 97  & 50,518 & 45.3 \\
        \midrule
        Pooled                        & 353 & 73,700 & 42.0 \\
        Macro average over corpora    & --  & --     & \textbf{38.4} \\
        \bottomrule
    \end{tabular}
\end{table}
