# Supplementary material for: A2Z GameSpec-Bench: How Faithfully Can Coding Agents Generate Games from Game Design Specifications?
Source: arXiv:2609.39564 source file (2026-09-30)
Supplement: Supplementary file 18 [file gdd_dataset_stats.tex]

\begin{table}[!t]
    \centering
    \caption{
        \textbf{GDD dataset statistics.}
        Document length and requirement composition of the
        \emph{Small} and \emph{Big} splits.
        Outcome requirements count individual promises in GDD
        rule-table rows, including presentation outcomes.
    }
    \label{tab:gdd_statistics}

    \small
    \setlength{\tabcolsep}{6pt}
    \renewcommand{\arraystretch}{1.12}

    \begin{tabular*}{\linewidth}{
        @{\extracolsep{\fill}}lcc@{}
    }
        \toprule
        \textbf{Statistic}
        & \textbf{\emph{Small}}
        & \textbf{\emph{Big}} \\
        \midrule

        Documents
        & 50
        & 50 \\

        Lines (mean)
        & 629
        & 1,153 \\

        \addlinespace[3pt]
        \textbf{Tokens (total)}
        & \textbf{704,270}
        & \textbf{1,314,862} \\

        Tokens (mean, range)
        & 14,085 (5,240--24,022)
        & 26,297 (12,489--51,433) \\

        \midrule

        \textbf{Outcome requirements (total)}
        & \textbf{2,710}
        & \textbf{4,202} \\

        Outcome requirements (mean, range)
        & 54.2 (9--151)
        & 84.0 (10--246) \\

        \addlinespace[3pt]
        Invariants (total)
        & 1,378
        & 1,862 \\

        Scenarios (total)
        & 646
        & 1,385 \\

        \bottomrule
    \end{tabular*}
\end{table}
