# Supplementary material for: A2Z GameSpec-Bench: How Faithfully Can Coding Agents Generate Games from Game Design Specifications?
Source: arXiv:2609.39564 source file (2026-09-30)
Supplement: Supplementary file 19 [file small_gdd_feats.tex]

\begin{table}[t]
    \centering
    \caption{\textbf{Task-family distribution of the \emph{Small} GDDs.}}
    \label{tab:small-family-distribution}

    \scriptsize
    \setlength{\tabcolsep}{4pt}
    \renewcommand{\arraystretch}{1.08}

    \begin{tabularx}{\linewidth}{
        @{}
        c
        >{\raggedright\arraybackslash}p{0.20\linewidth}
        c
        >{\raggedright\arraybackslash}X
        @{}
    }
        \toprule
        \# & \textbf{Task Family} & \textbf{$n$} & \textbf{Games} \\
        \midrule

        1
        & Reaction, Inhibition \newline \&  Speed Classification
        & 9
        & \texttt{reaction\_test},
          \texttt{no\_response\_test},
          \texttt{bloom\_or\_weed},
          \texttt{orbit},
          \texttt{bin\_bit},
          \texttt{odd\_even\_flash},
          \texttt{odd\_patch},
          \texttt{same\_or\_shift},
          \texttt{three\_letter\_delivery}
        \\

        2
        & Temporal Precision \newline \& Rhythm
        & 7
        & \texttt{beat\_bistro},
          \texttt{centerline},
          \texttt{chord\_snap},
          \texttt{half\_beat\_bell},
          \texttt{ooga\_ooga\_tower},
          \texttt{ozone\_dash},
          \texttt{rooftop\_rumble}
        \\

        3
        & Continuous \newline \& Precision Motor Control
        & 9
        & \texttt{cursor\_pursuit},
          \texttt{still\_cursor},
          \texttt{chalk\_escape},
          \texttt{stamp\_register},
          \texttt{pocket\_curling},
          \texttt{magnet\_dock},
          \texttt{safe\_dial},
          \texttt{warm\_ascent},
          \texttt{wheel\_steps}
        \\

        4
        & Short-Term Memory \newline \&  Attentional Tracking
        & 3
        & \texttt{echo\_three},
          \texttt{hidden\_spot},
          \texttt{key\_under\_cups}
        \\

        5
        & Perceptual Estimation \newline \& Psychophysics
        & 4
        & \texttt{blink\_count},
          \texttt{equal\_slice},
          \texttt{mobile\_balance},
          \texttt{whisper\_compass}
        \\

        6
        & Spatial Reasoning \newline \&  Mental Transformation
        & 5
        & \texttt{one\_fold\_letter},
          \texttt{shadow\_pair},
          \texttt{lighthouse\_mirrors},
          \texttt{tiny\_moving\_van},
          \texttt{untangled\_cords}
        \\

        7
        & Deduction \newline \& Constraint Solving
        & 6
        & \texttt{clue\_lock},
          \texttt{mini\_nonogram},
          \texttt{three\_switches},
          \texttt{traces\_left},
          \texttt{one\_segment\_equation},
          \texttt{last\_match}
        \\

        8
        & Planning  \newline \& Sequential Decision
        & 7
        & \texttt{blackout\_dispatch},
          \texttt{crate\_corner},
          \texttt{color\_flood},
          \texttt{peg\_garden},
          \texttt{pancake\_prefix},
          \texttt{tile\_merge},
          \texttt{greedy\_die}
        \\

        \bottomrule
    \end{tabularx}
\end{table}
