# Supplementary material for: A2Z GameSpec-Bench: How Faithfully Can Coding Agents Generate Games from Game Design Specifications?
Source: arXiv:2609.39564 source file (2026-09-30)
Supplement: Supplementary file 20 [file source_code_cost.tex]

\begin{table}[t]
    \centering
    \caption{\textbf{Agreement and cost across source-code judge configurations.}
    Rule-level correlation and invariant agreement are measured against a fixed set of reference judgments from GPT-5.6-Sol at extra-high reasoning effort.
    The first row reports an independent re-run of that configuration.
    Mean Rule Score reports the average rule implementation score in each run.
    Relative cost is estimated from token usage per call and the prices used in the experiment, normalized to the first row.}
    \label{tab:fid-effort}
    \vspace{2pt}

    \footnotesize
    \setlength{\tabcolsep}{3pt}
    \renewcommand{\arraystretch}{1.14}
    \setlength{\extrarowheight}{0pt}

    % Vertically center multiline cells within this table.
    \renewcommand{\tabularxcolumn}[1]{m{#1}}

    \begin{tabularx}{0.98\linewidth}{
        @{}
        >{\raggedright\arraybackslash}m{0.175\linewidth}
        >{\raggedright\arraybackslash}m{0.105\linewidth}
        *{5}{>{\centering\arraybackslash}X}
        @{}
    }
        \toprule

        \multicolumn{1}{c}{\textbf{Judge}}
        & \multicolumn{1}{c}{\textbf{Effort}}
        & {\bfseries Rule-Level\newline \mbox{Correlation {\boldmath$r$}}}
        & {\bfseries Invariant\newline Agreement}
        & {\bfseries Mean\newline Rule Score}
        & {\bfseries Tokens/Call\newline {\boldmath$(10^3)$}}
        & {\bfseries Relative\newline Cost}
        \\
        \midrule

        \multirow[c]{4}{*}{\textbf{GPT-5.6-Sol}}
        & Extra high & 0.74 & 0.83 & 0.76 & 213 & 1.00 \\
        & High       & 0.70 & 0.83 & 0.76 & 214 & 1.00 \\
        & Medium     & 0.75 & 0.88 & 0.78 & 176 & 0.83 \\
        & Low        & 0.80 & 0.86 & 0.79 & 160 & 0.75 \\
        \midrule

        \multirow[c]{4}{*}{\textbf{GPT-5.6-Luna}}
        & Extra high & 0.72 & 0.77 & 0.79 & 198 & 0.15 \\
        & High       & 0.72 & 0.76 & 0.79 & 187 & 0.15 \\
        & Medium     & 0.69 & 0.75 & 0.80 & 169 & 0.13 \\
        & Low        & 0.71 & 0.73 & 0.77 & 151 & 0.12 \\

        \bottomrule
    \end{tabularx}
\end{table}
